# Supplementary material for: Magnesium abundances in cool metal-polluted white dwarfs
Source: arXiv:2006.04755 ancillary file (2020-09-10)

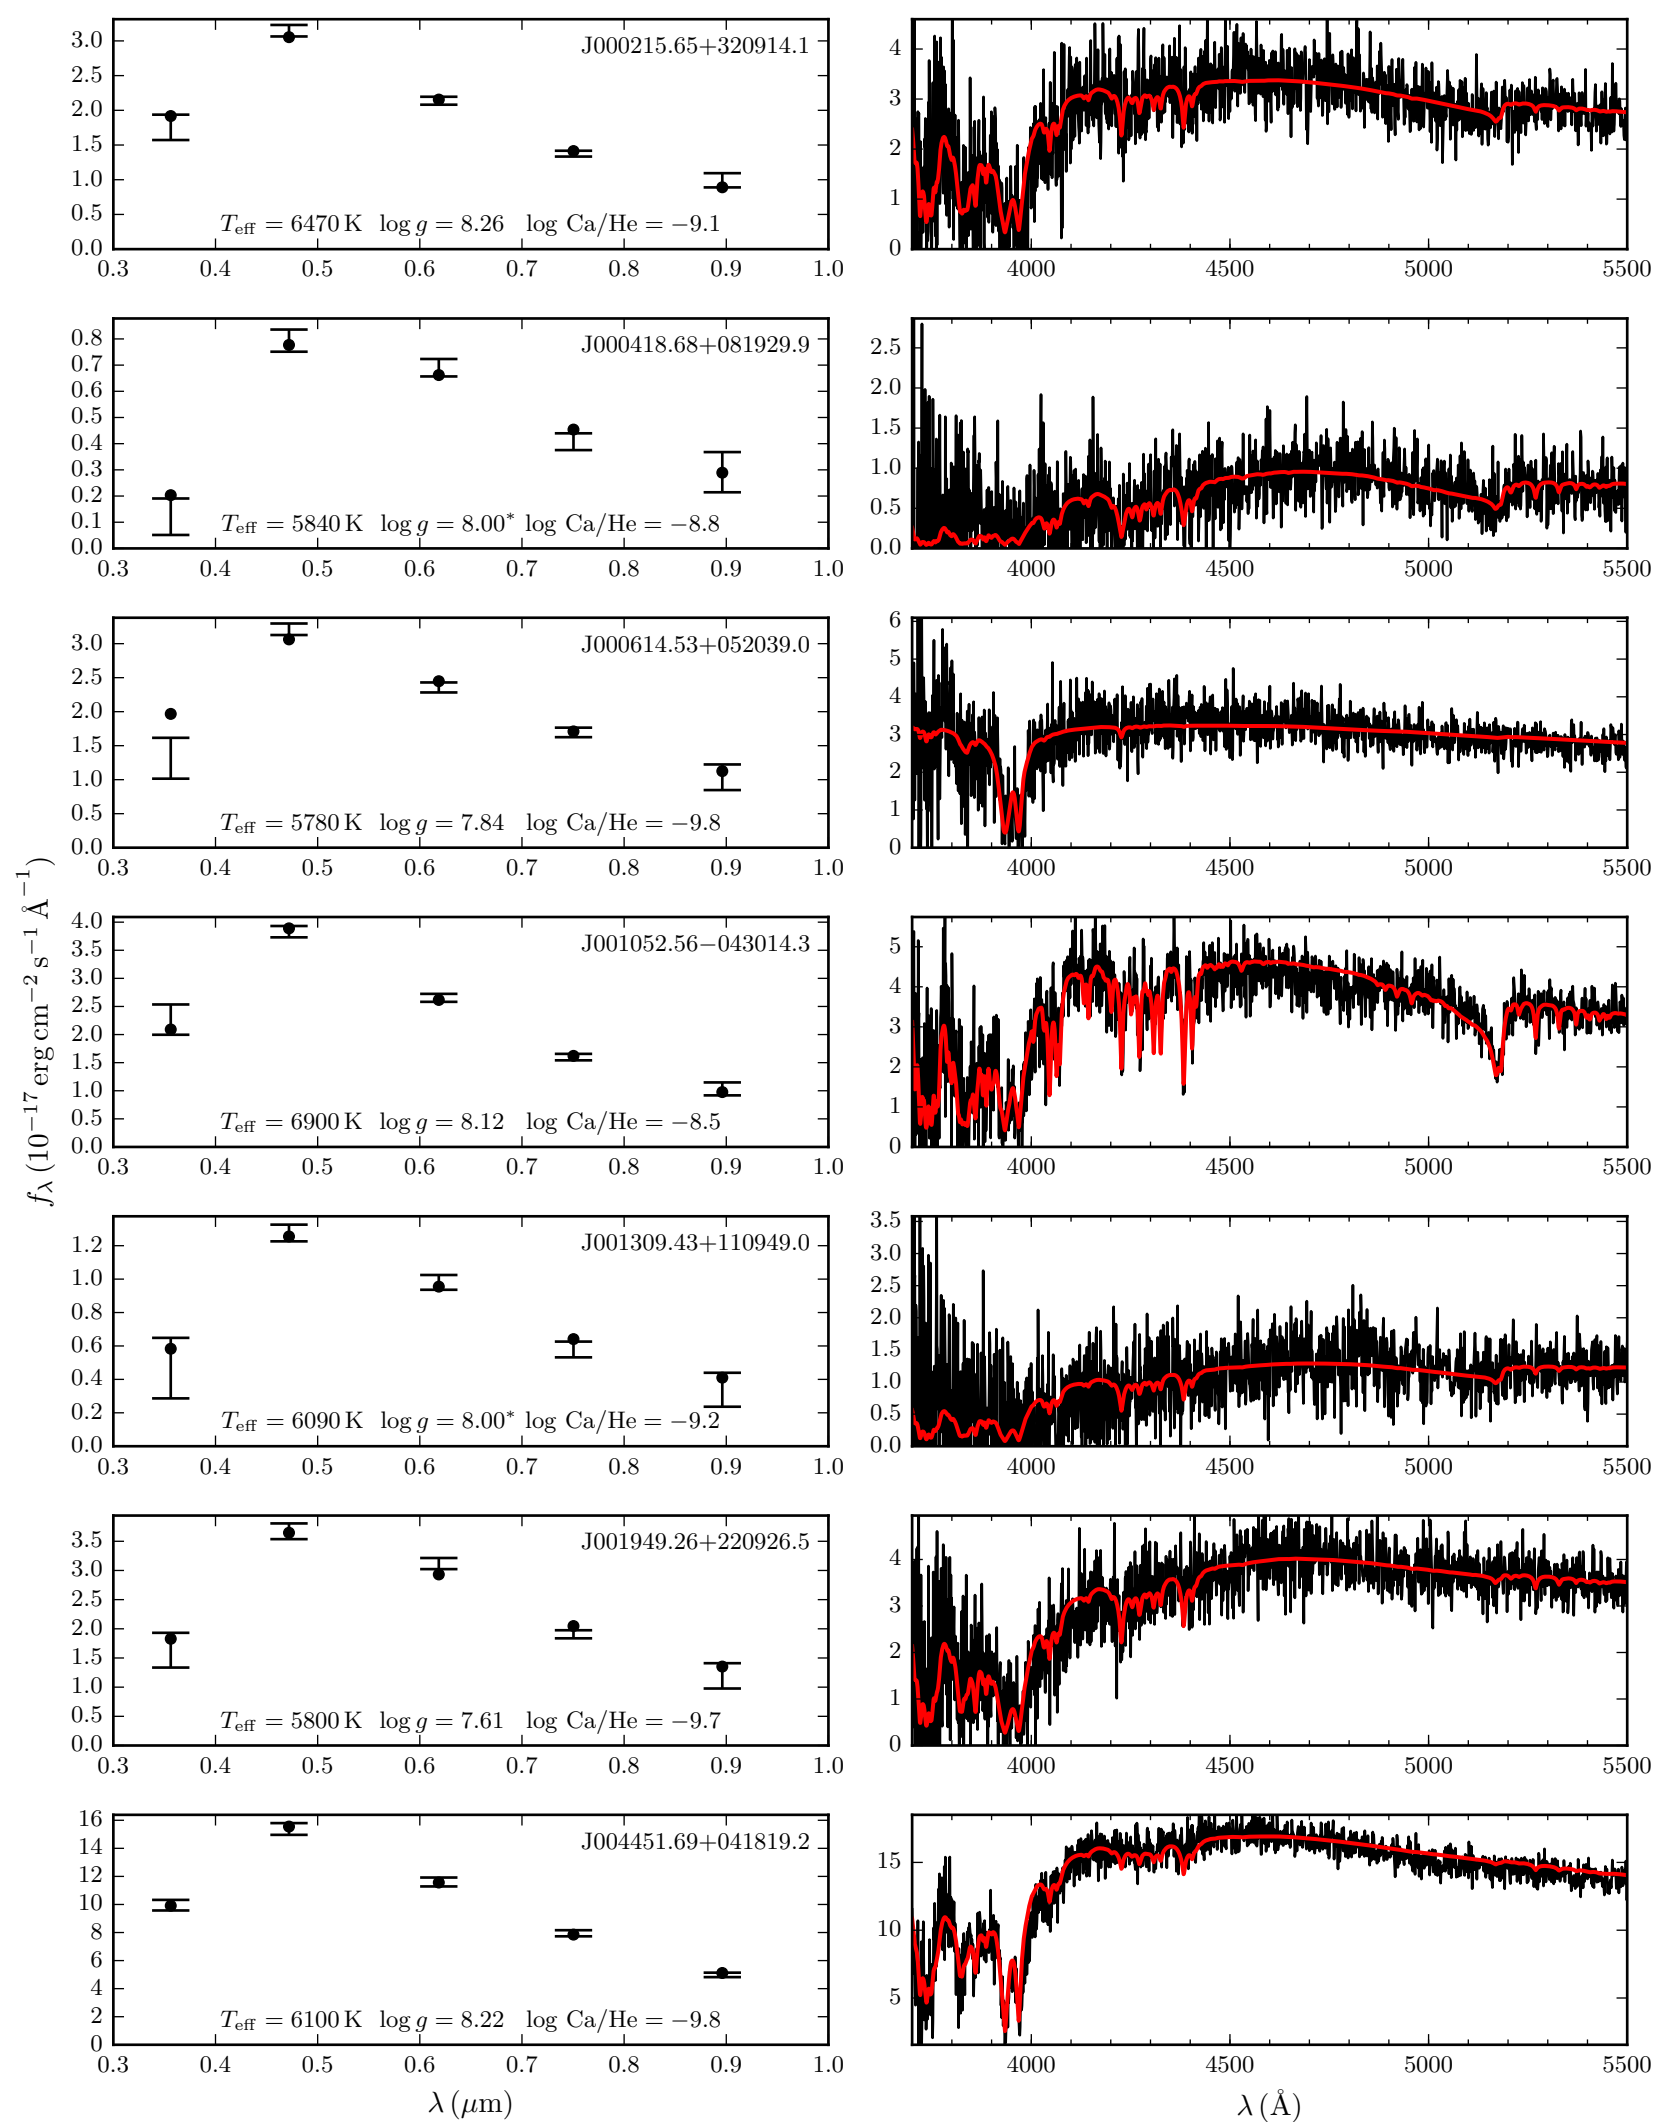

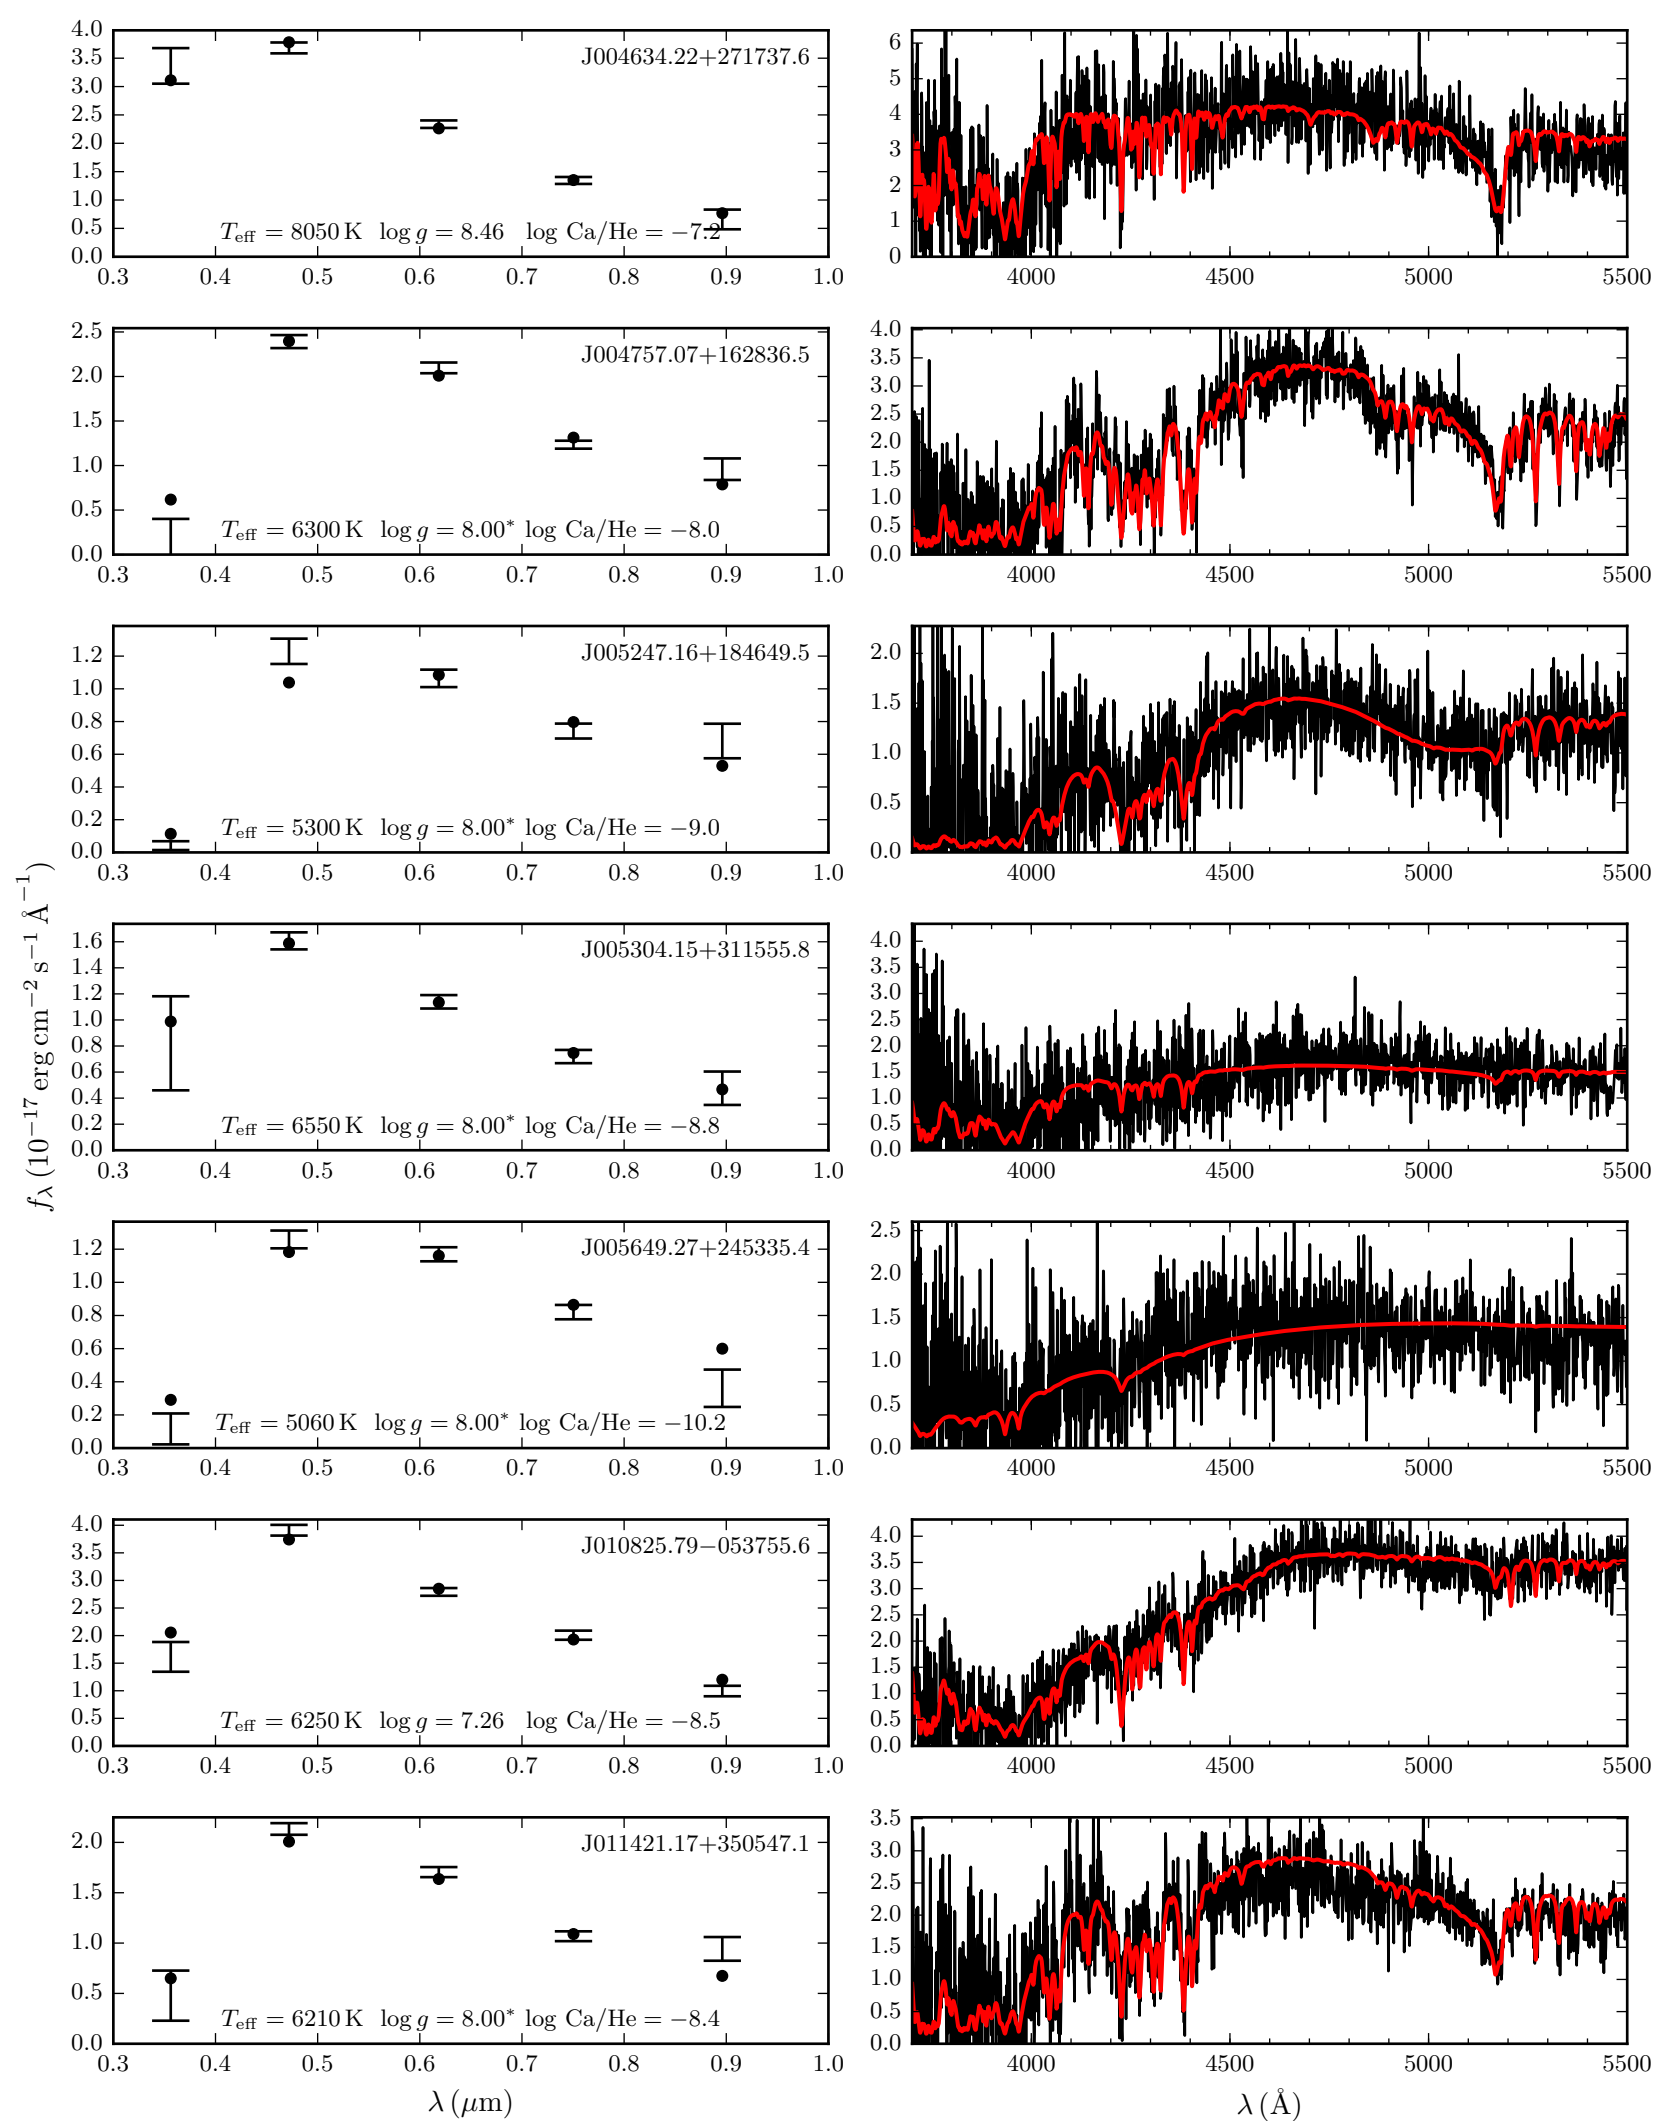

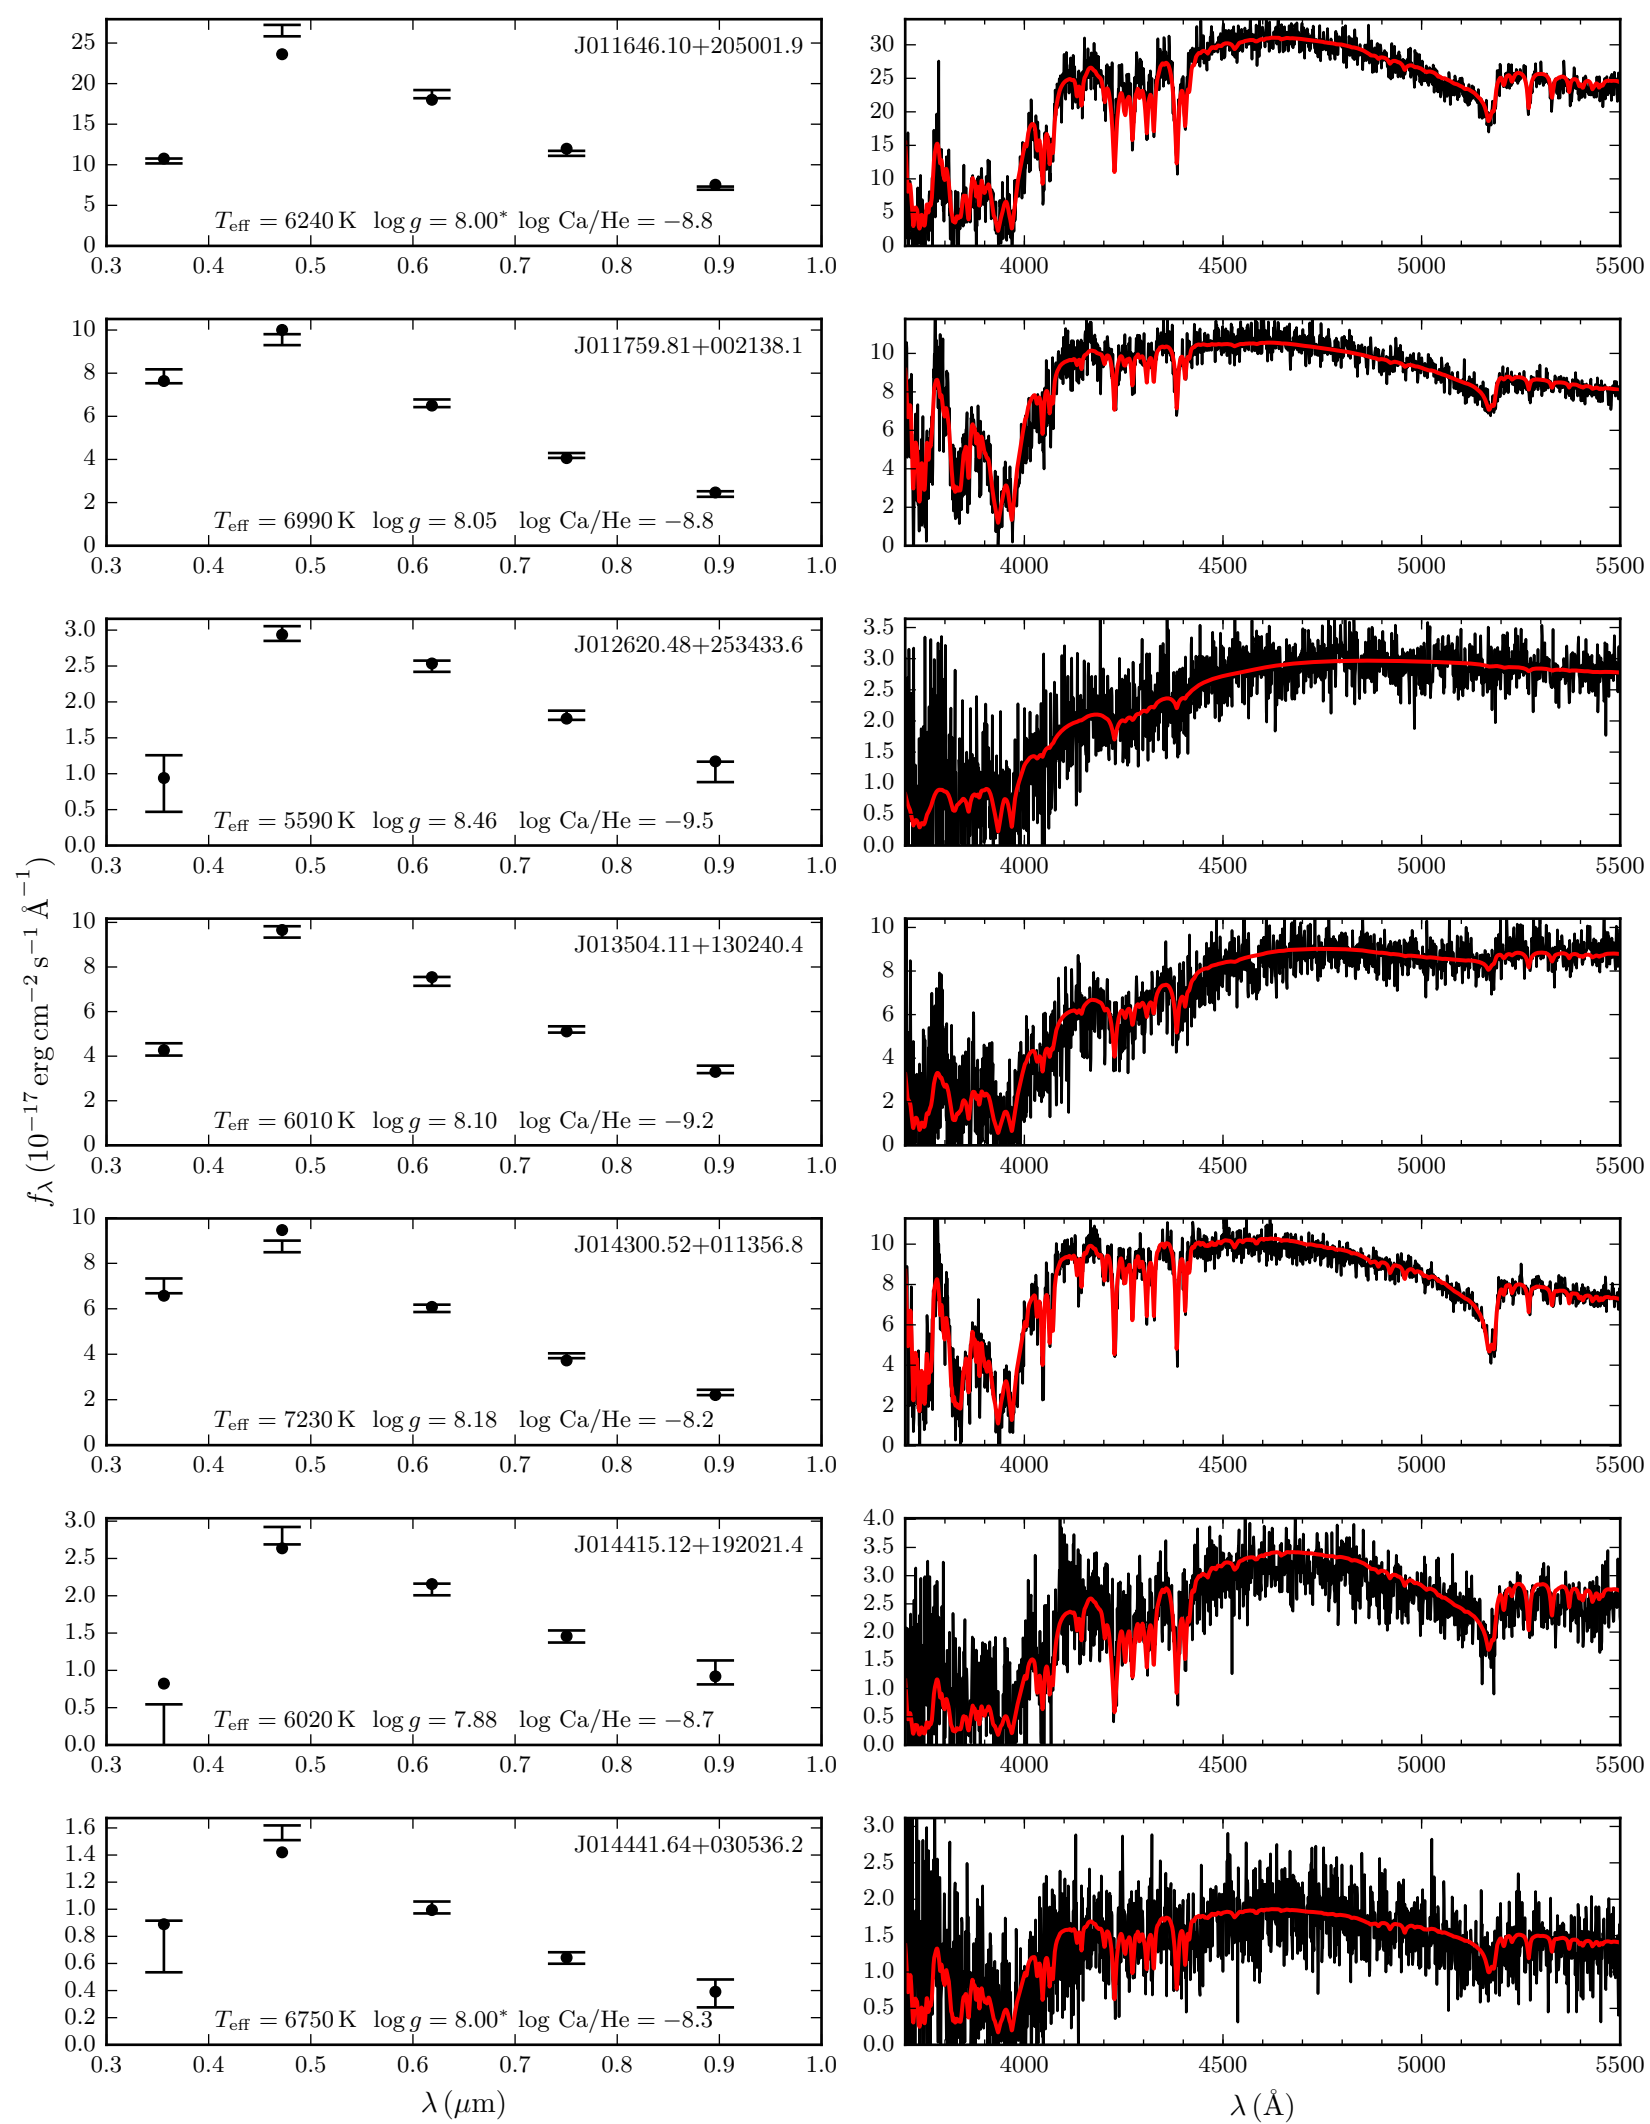

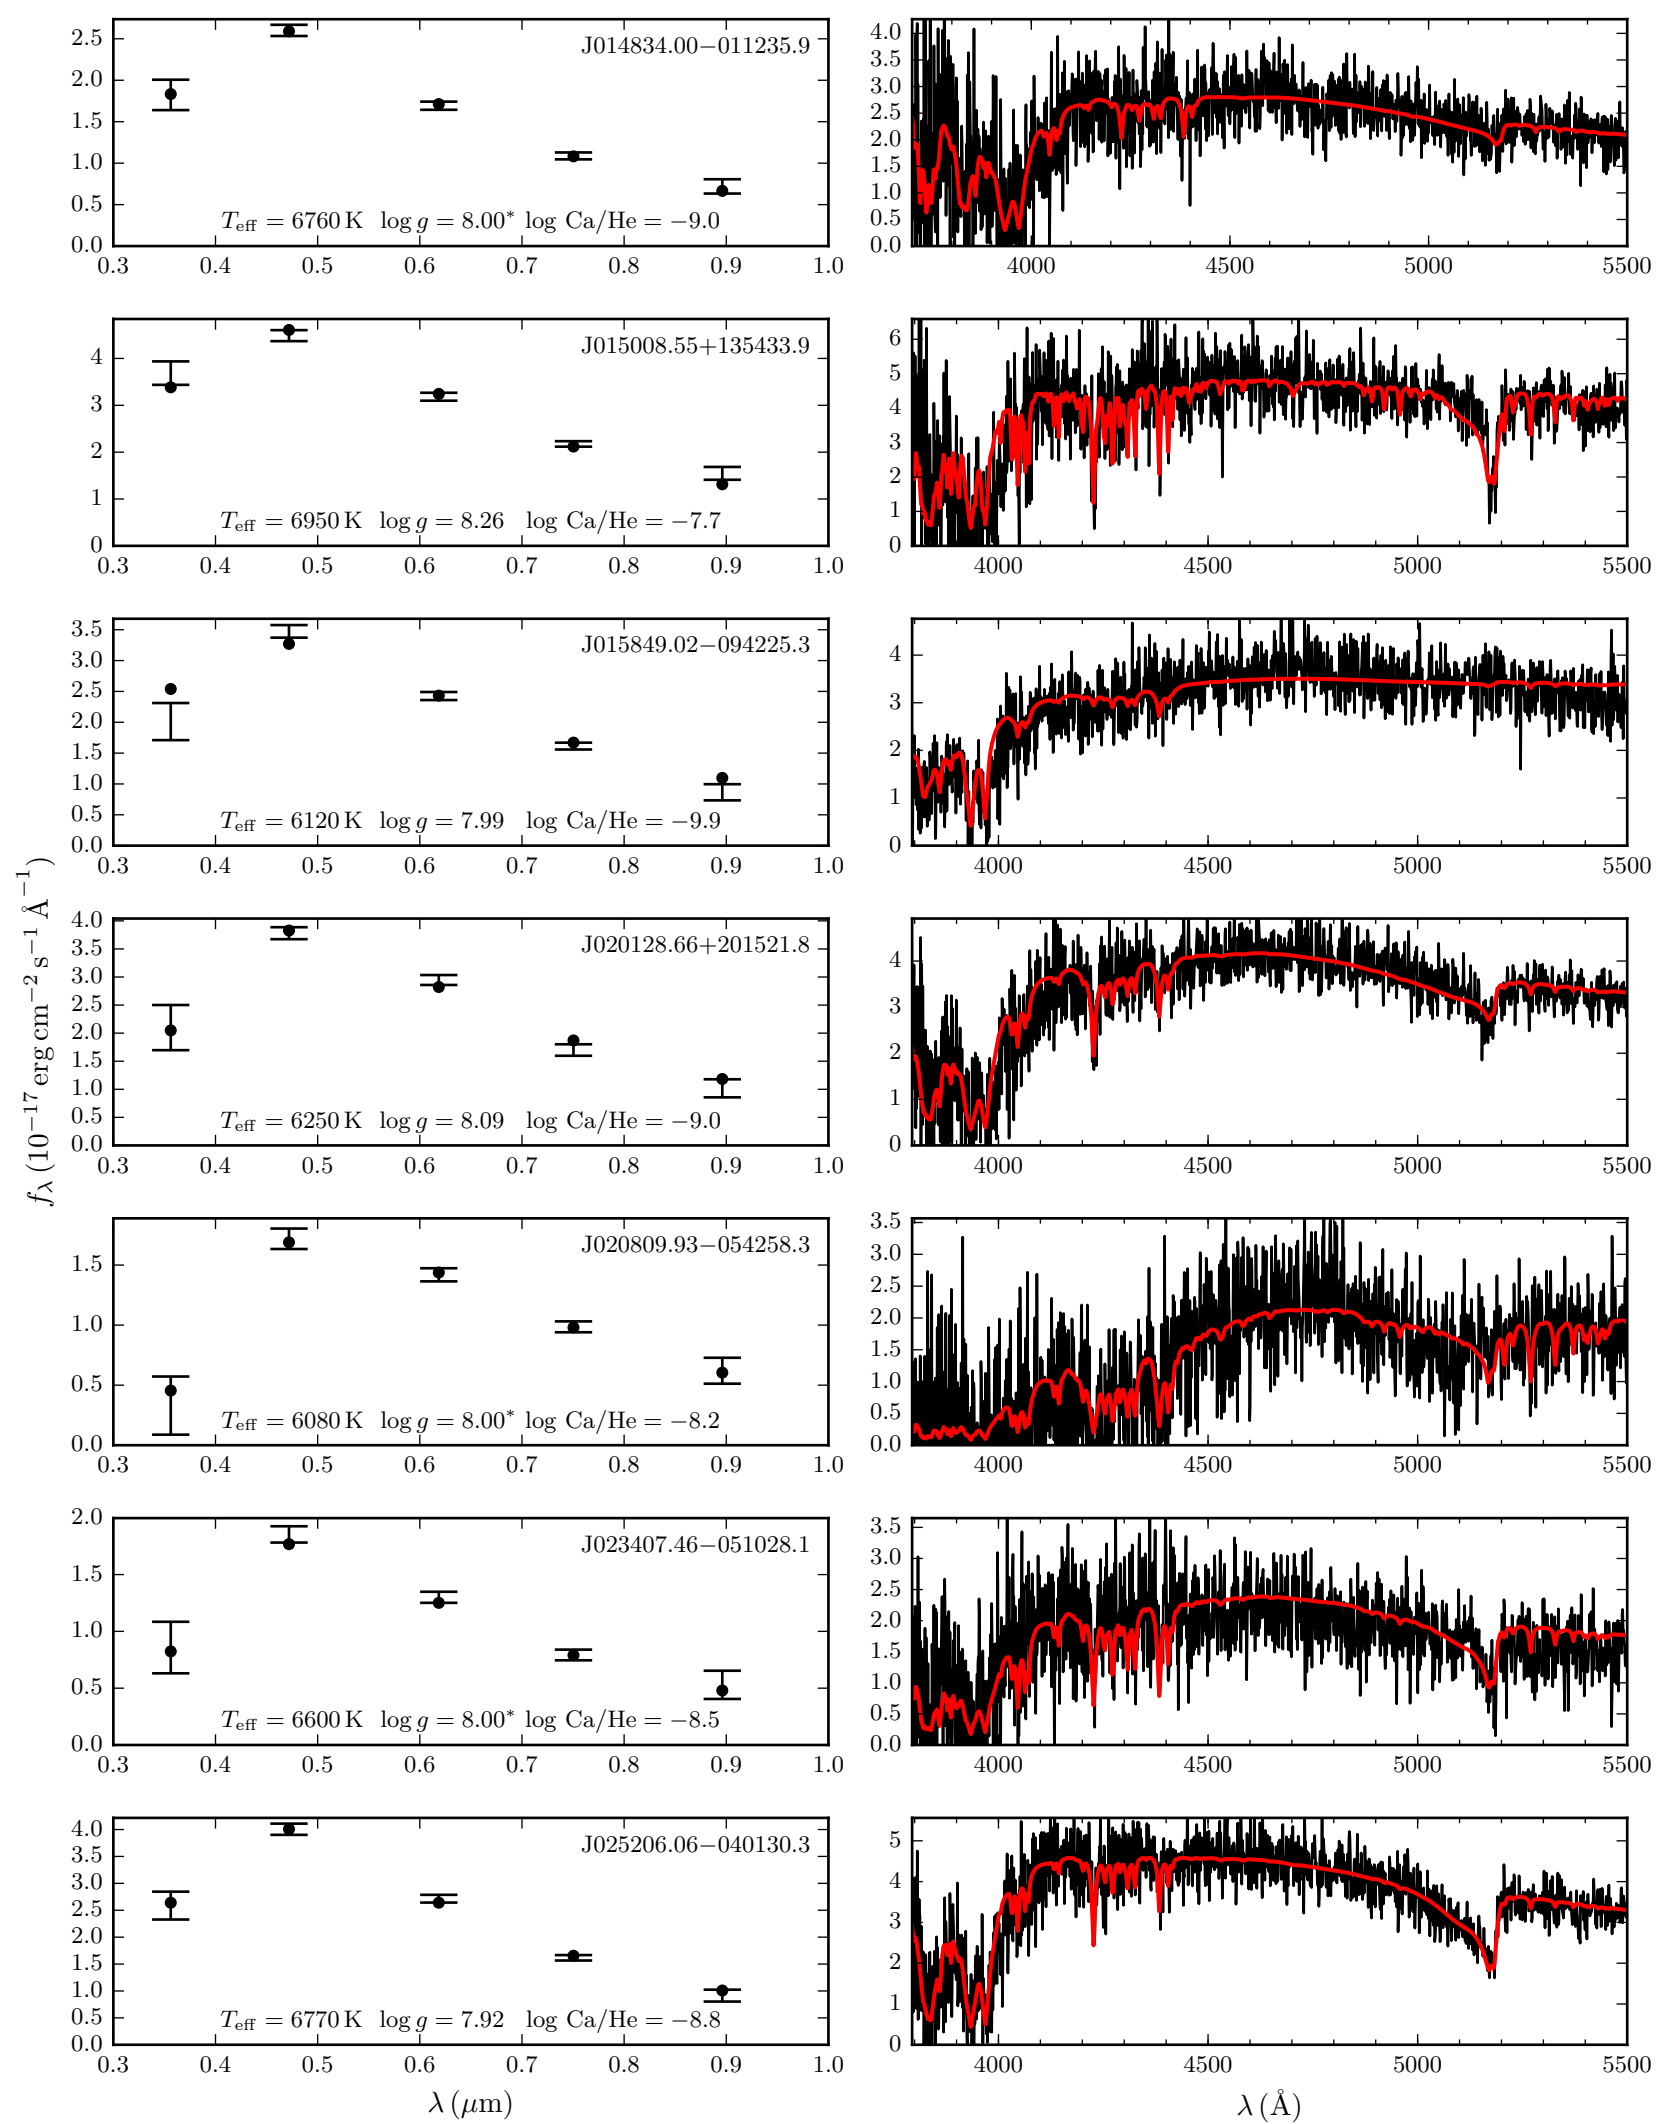

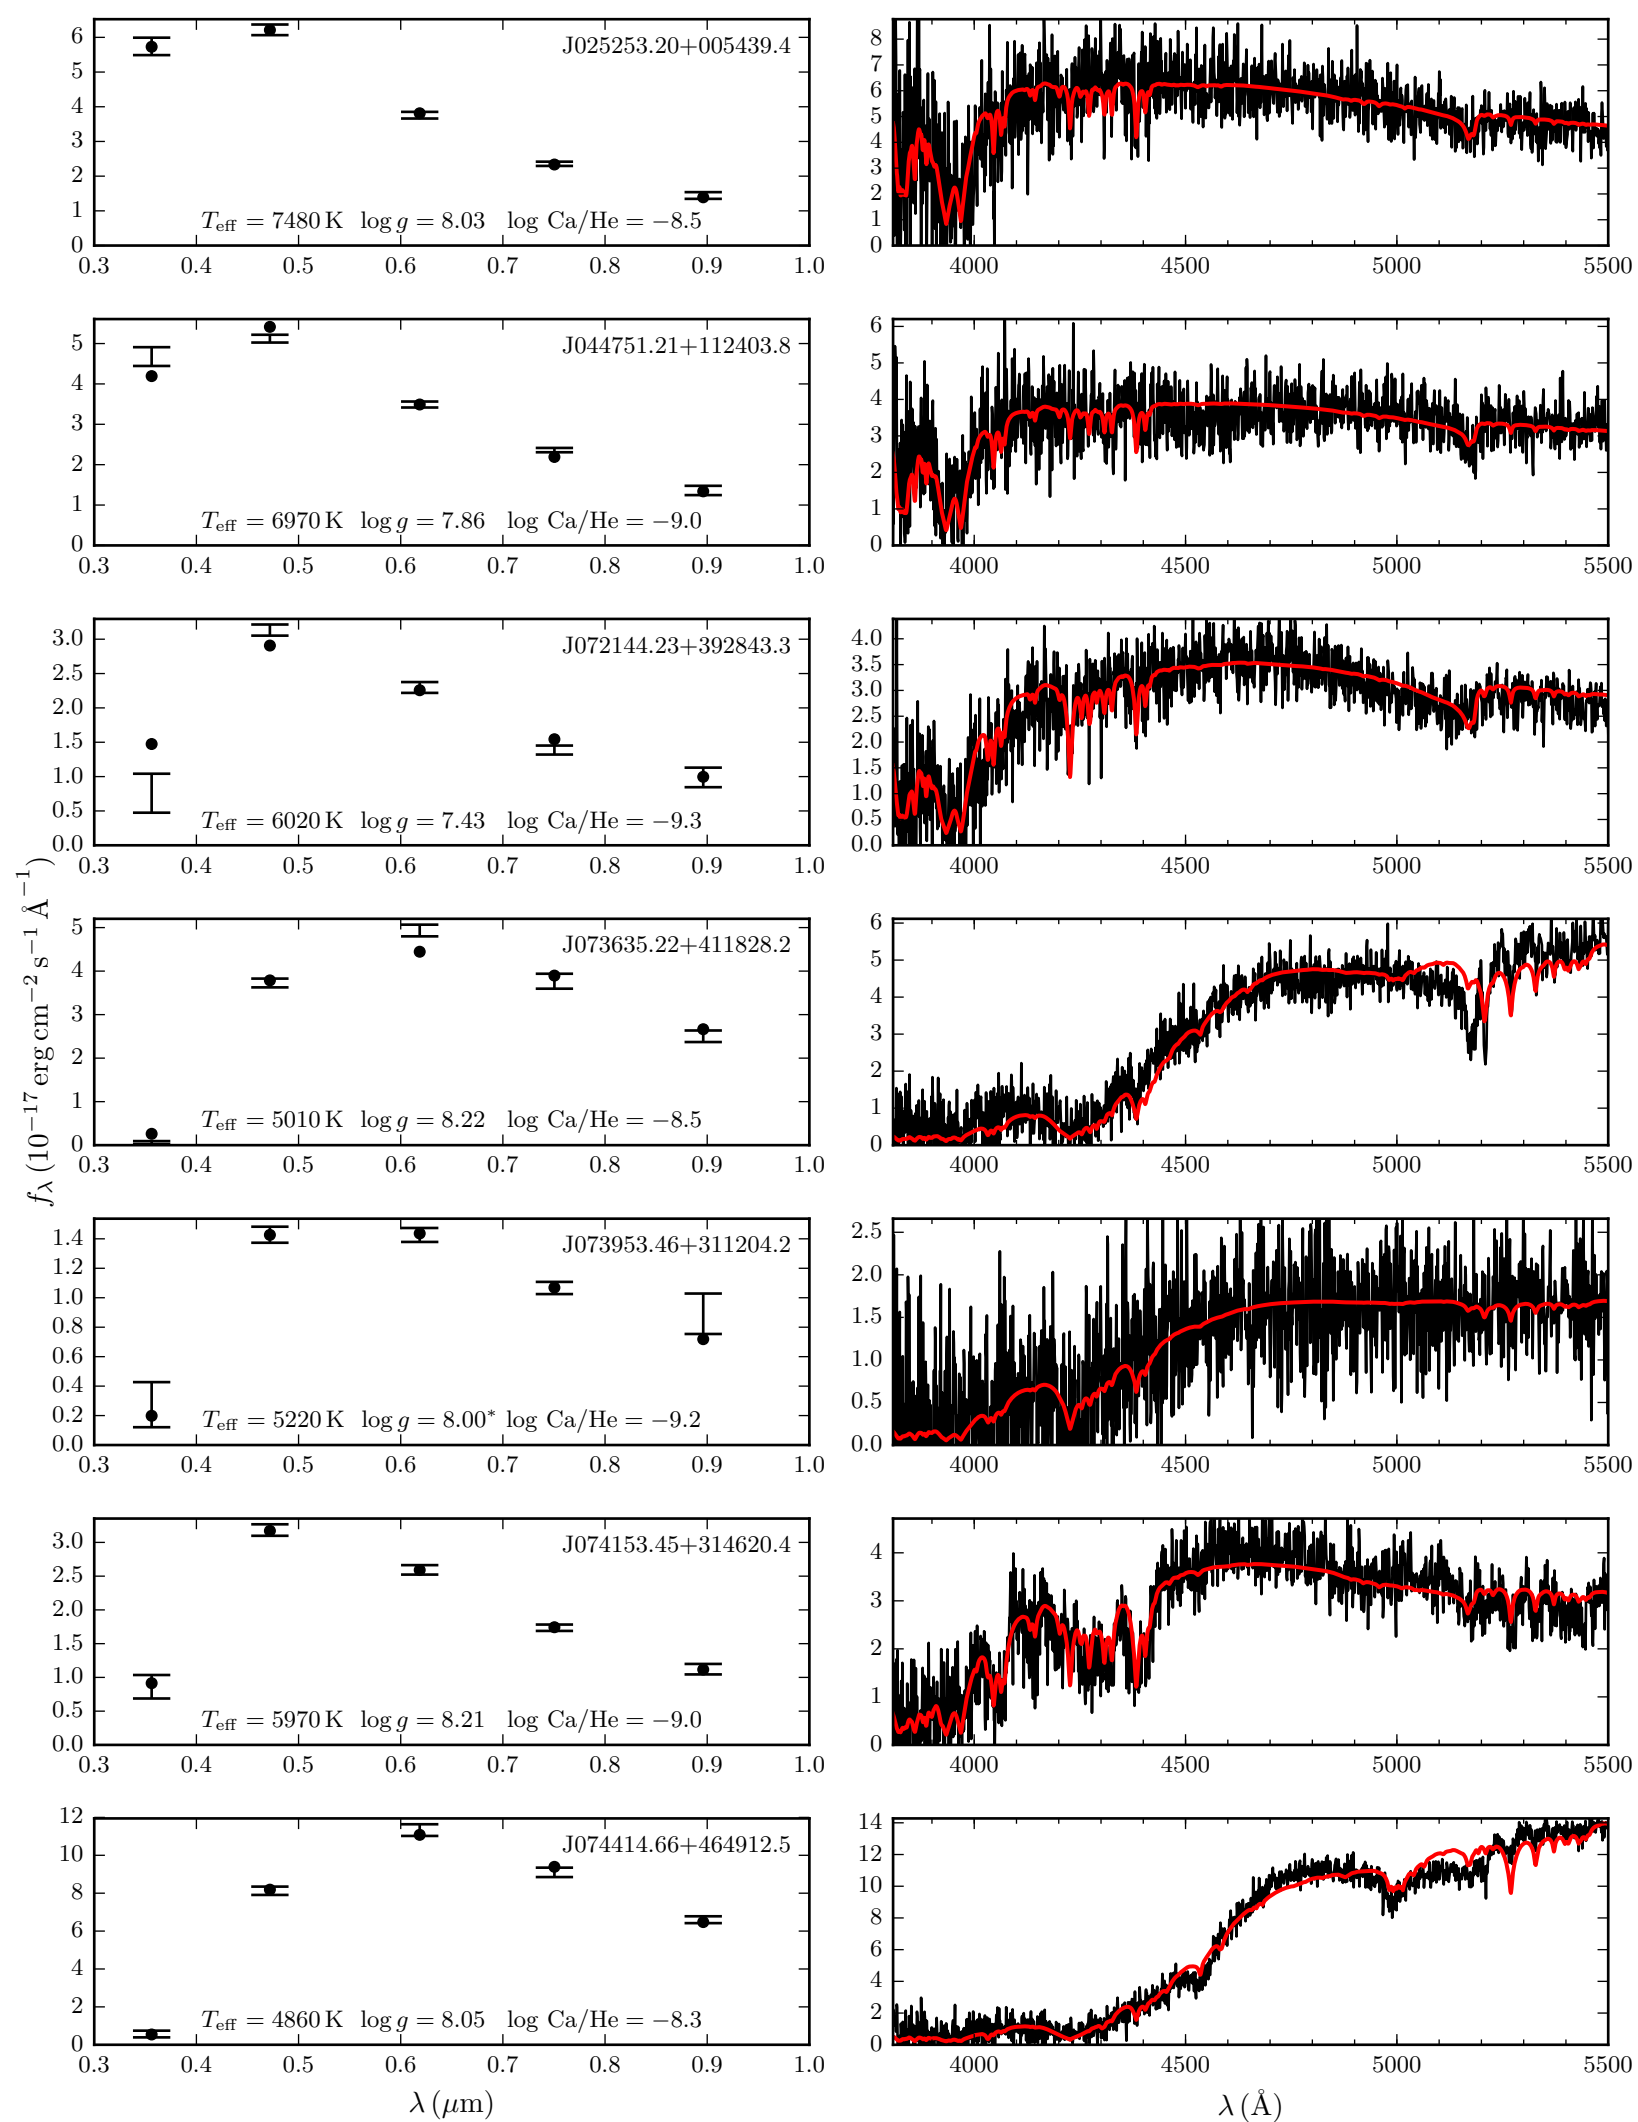

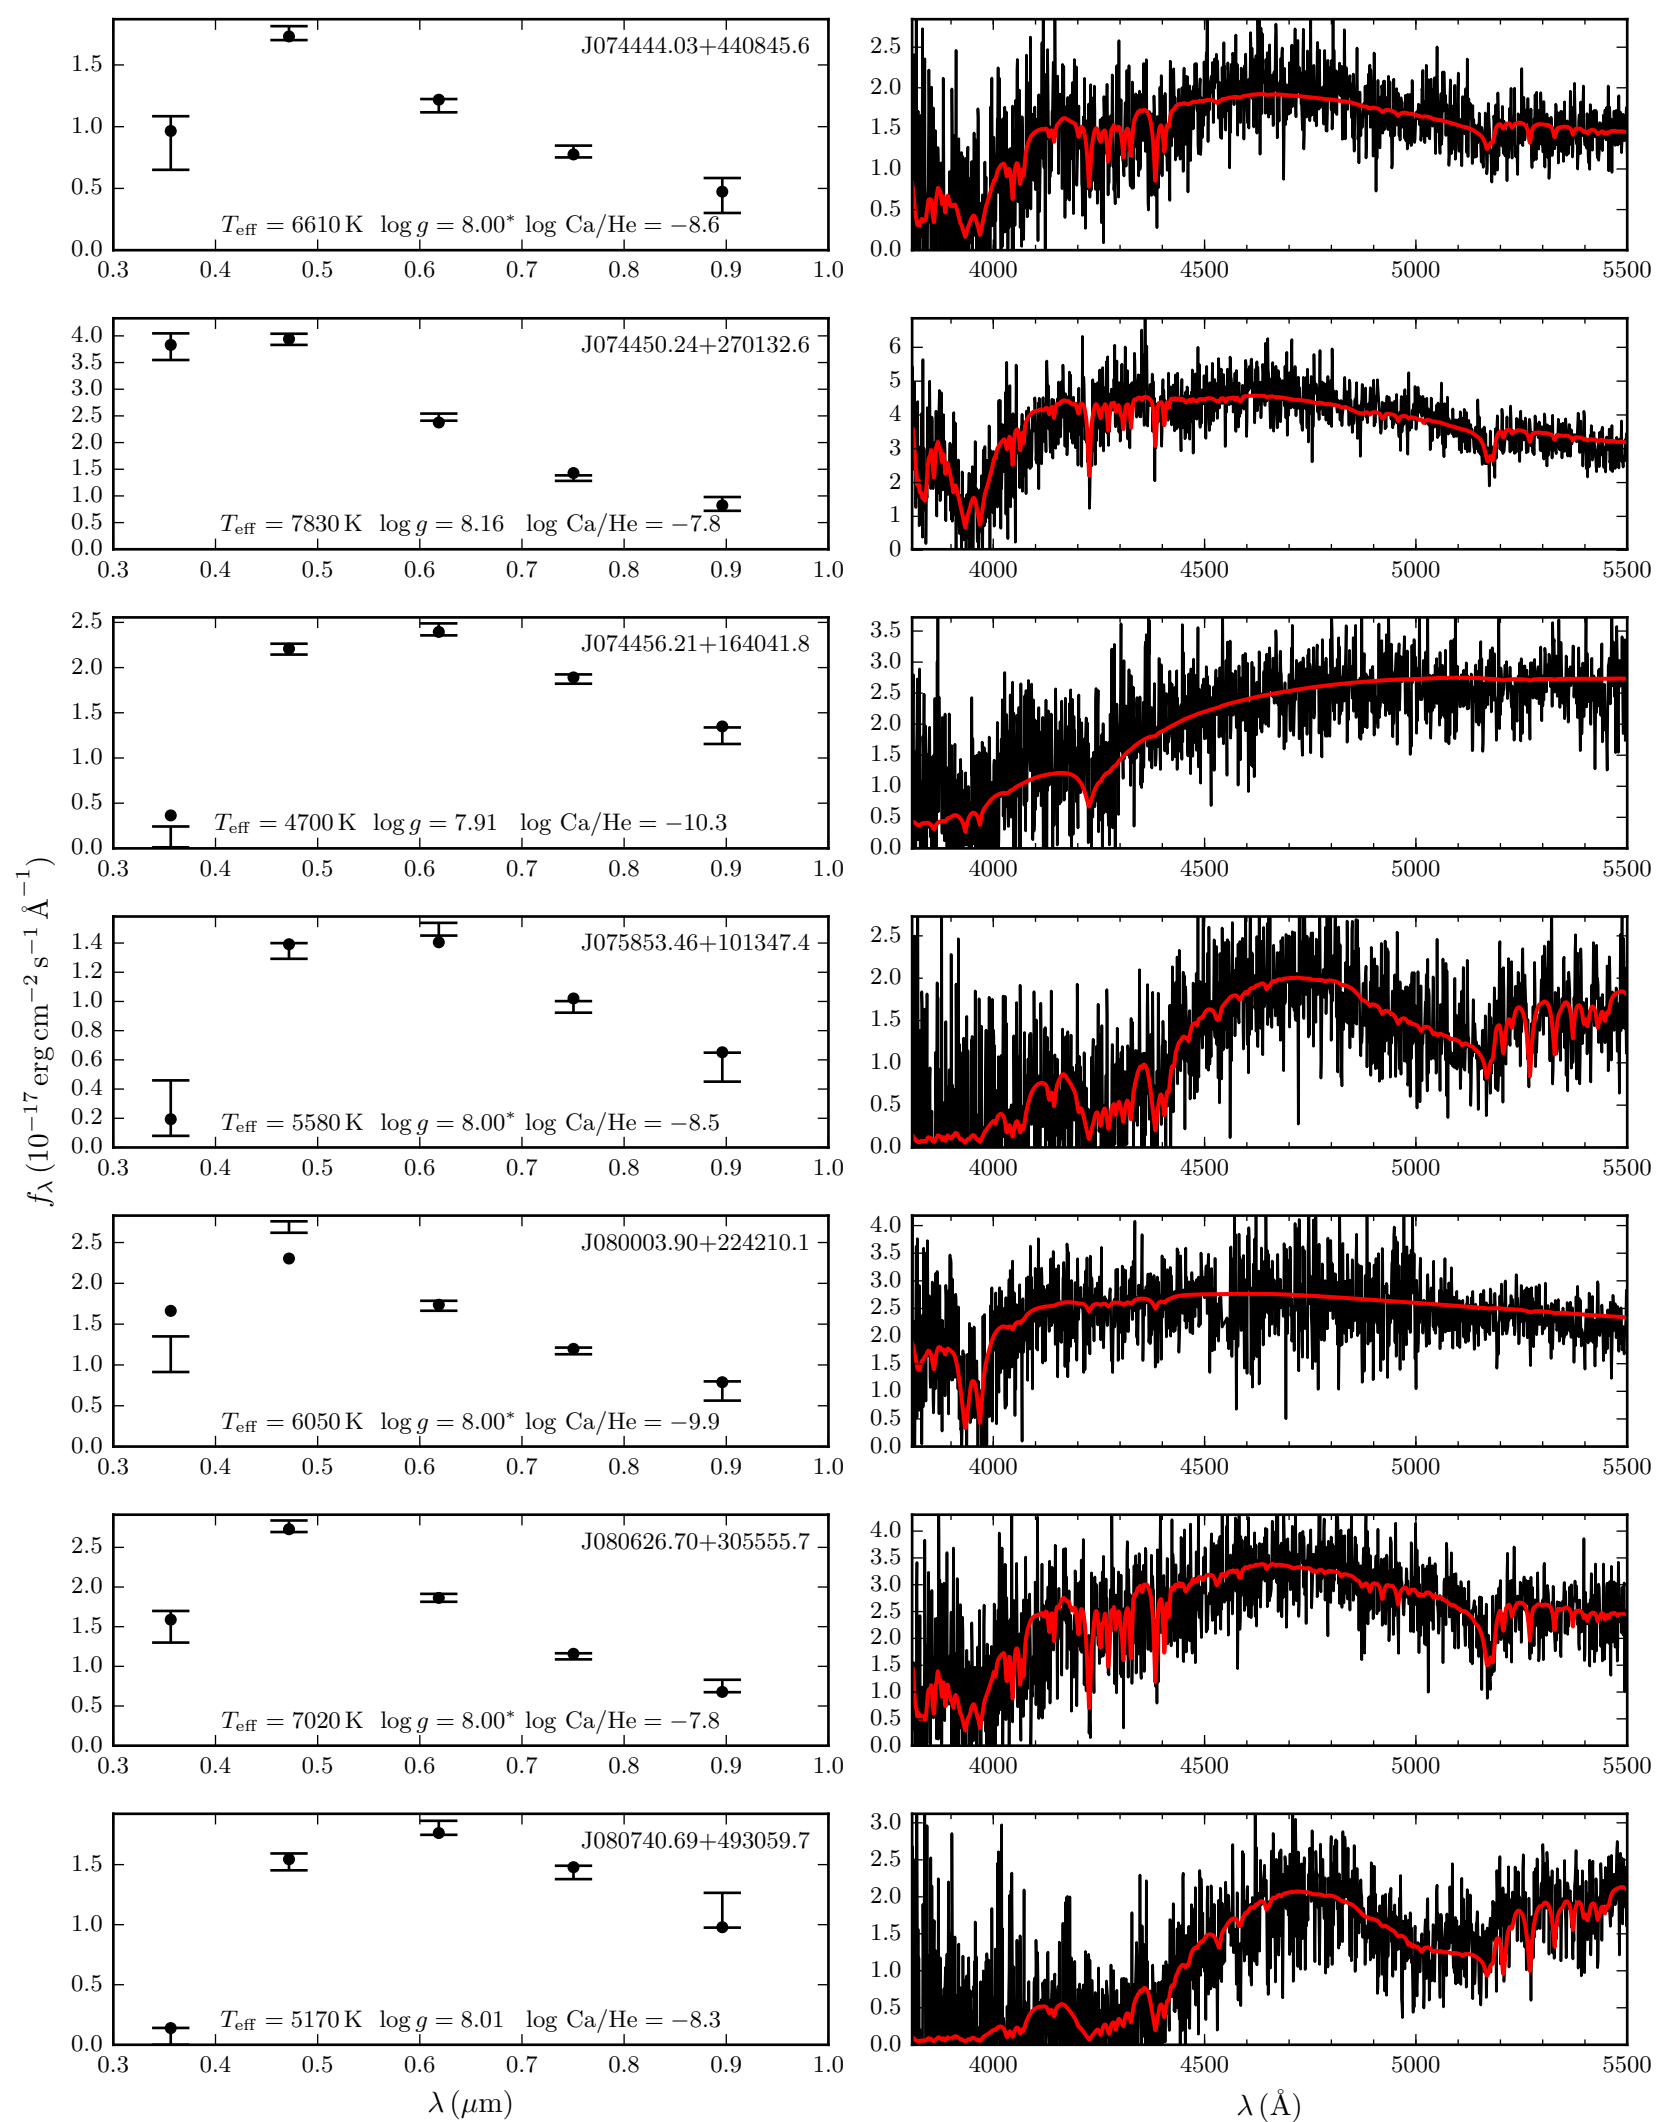

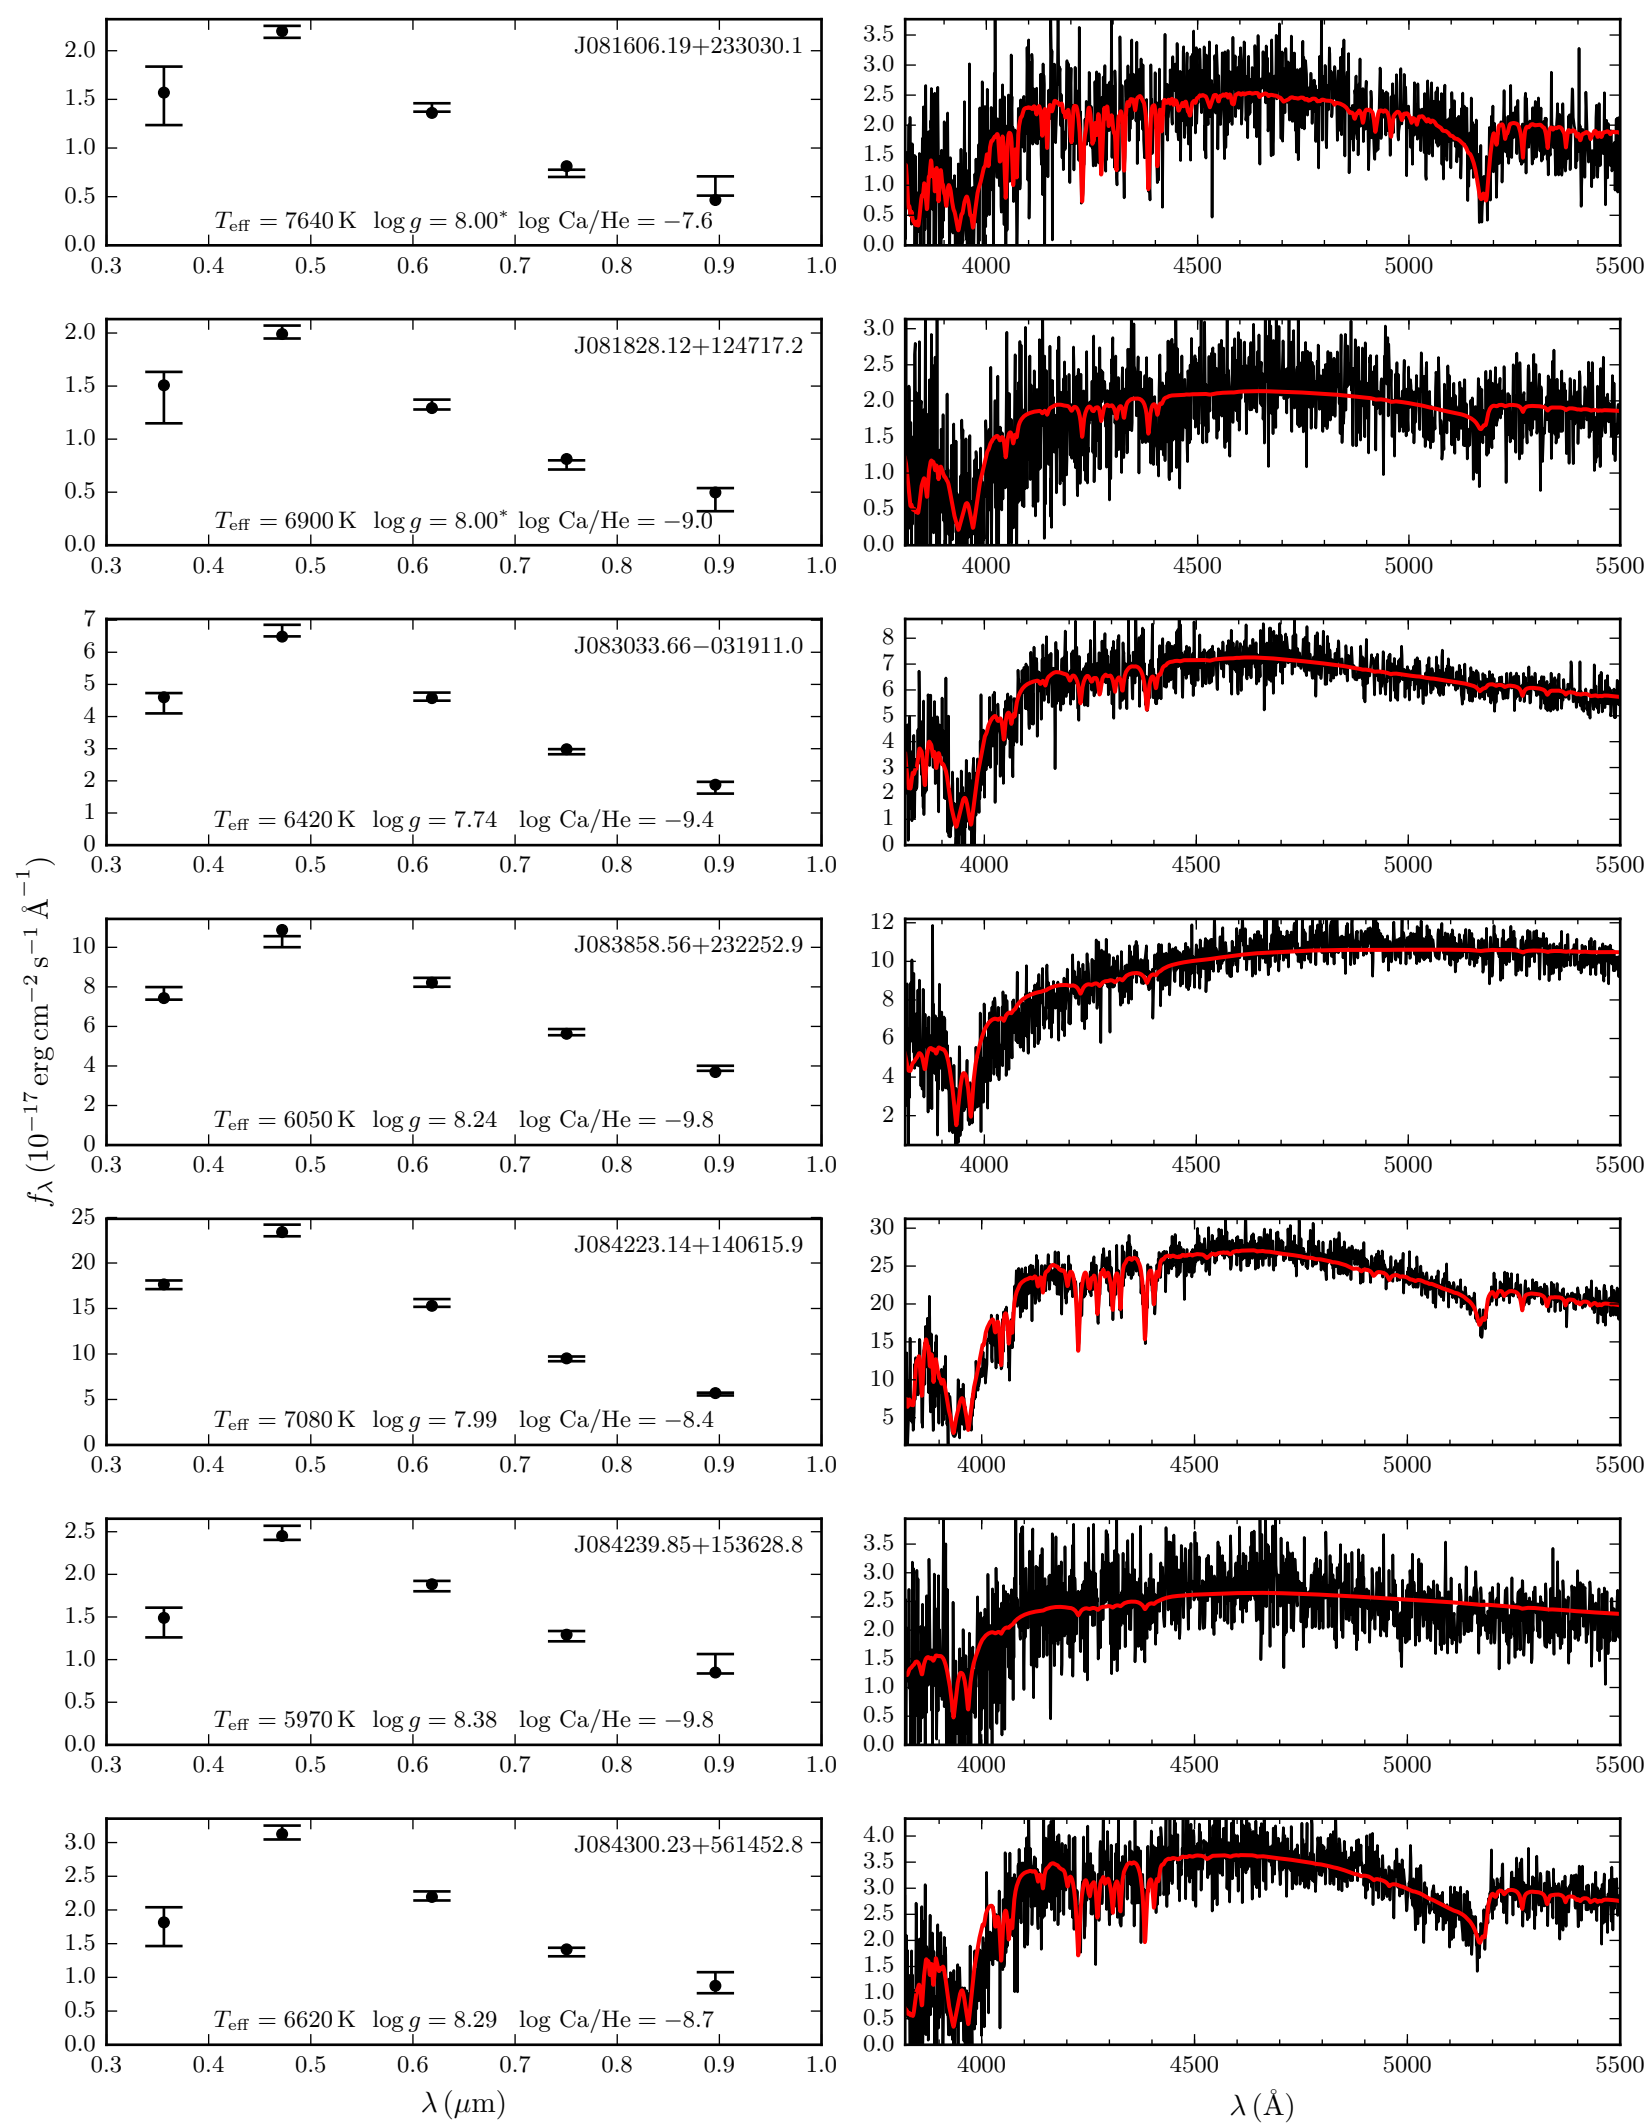



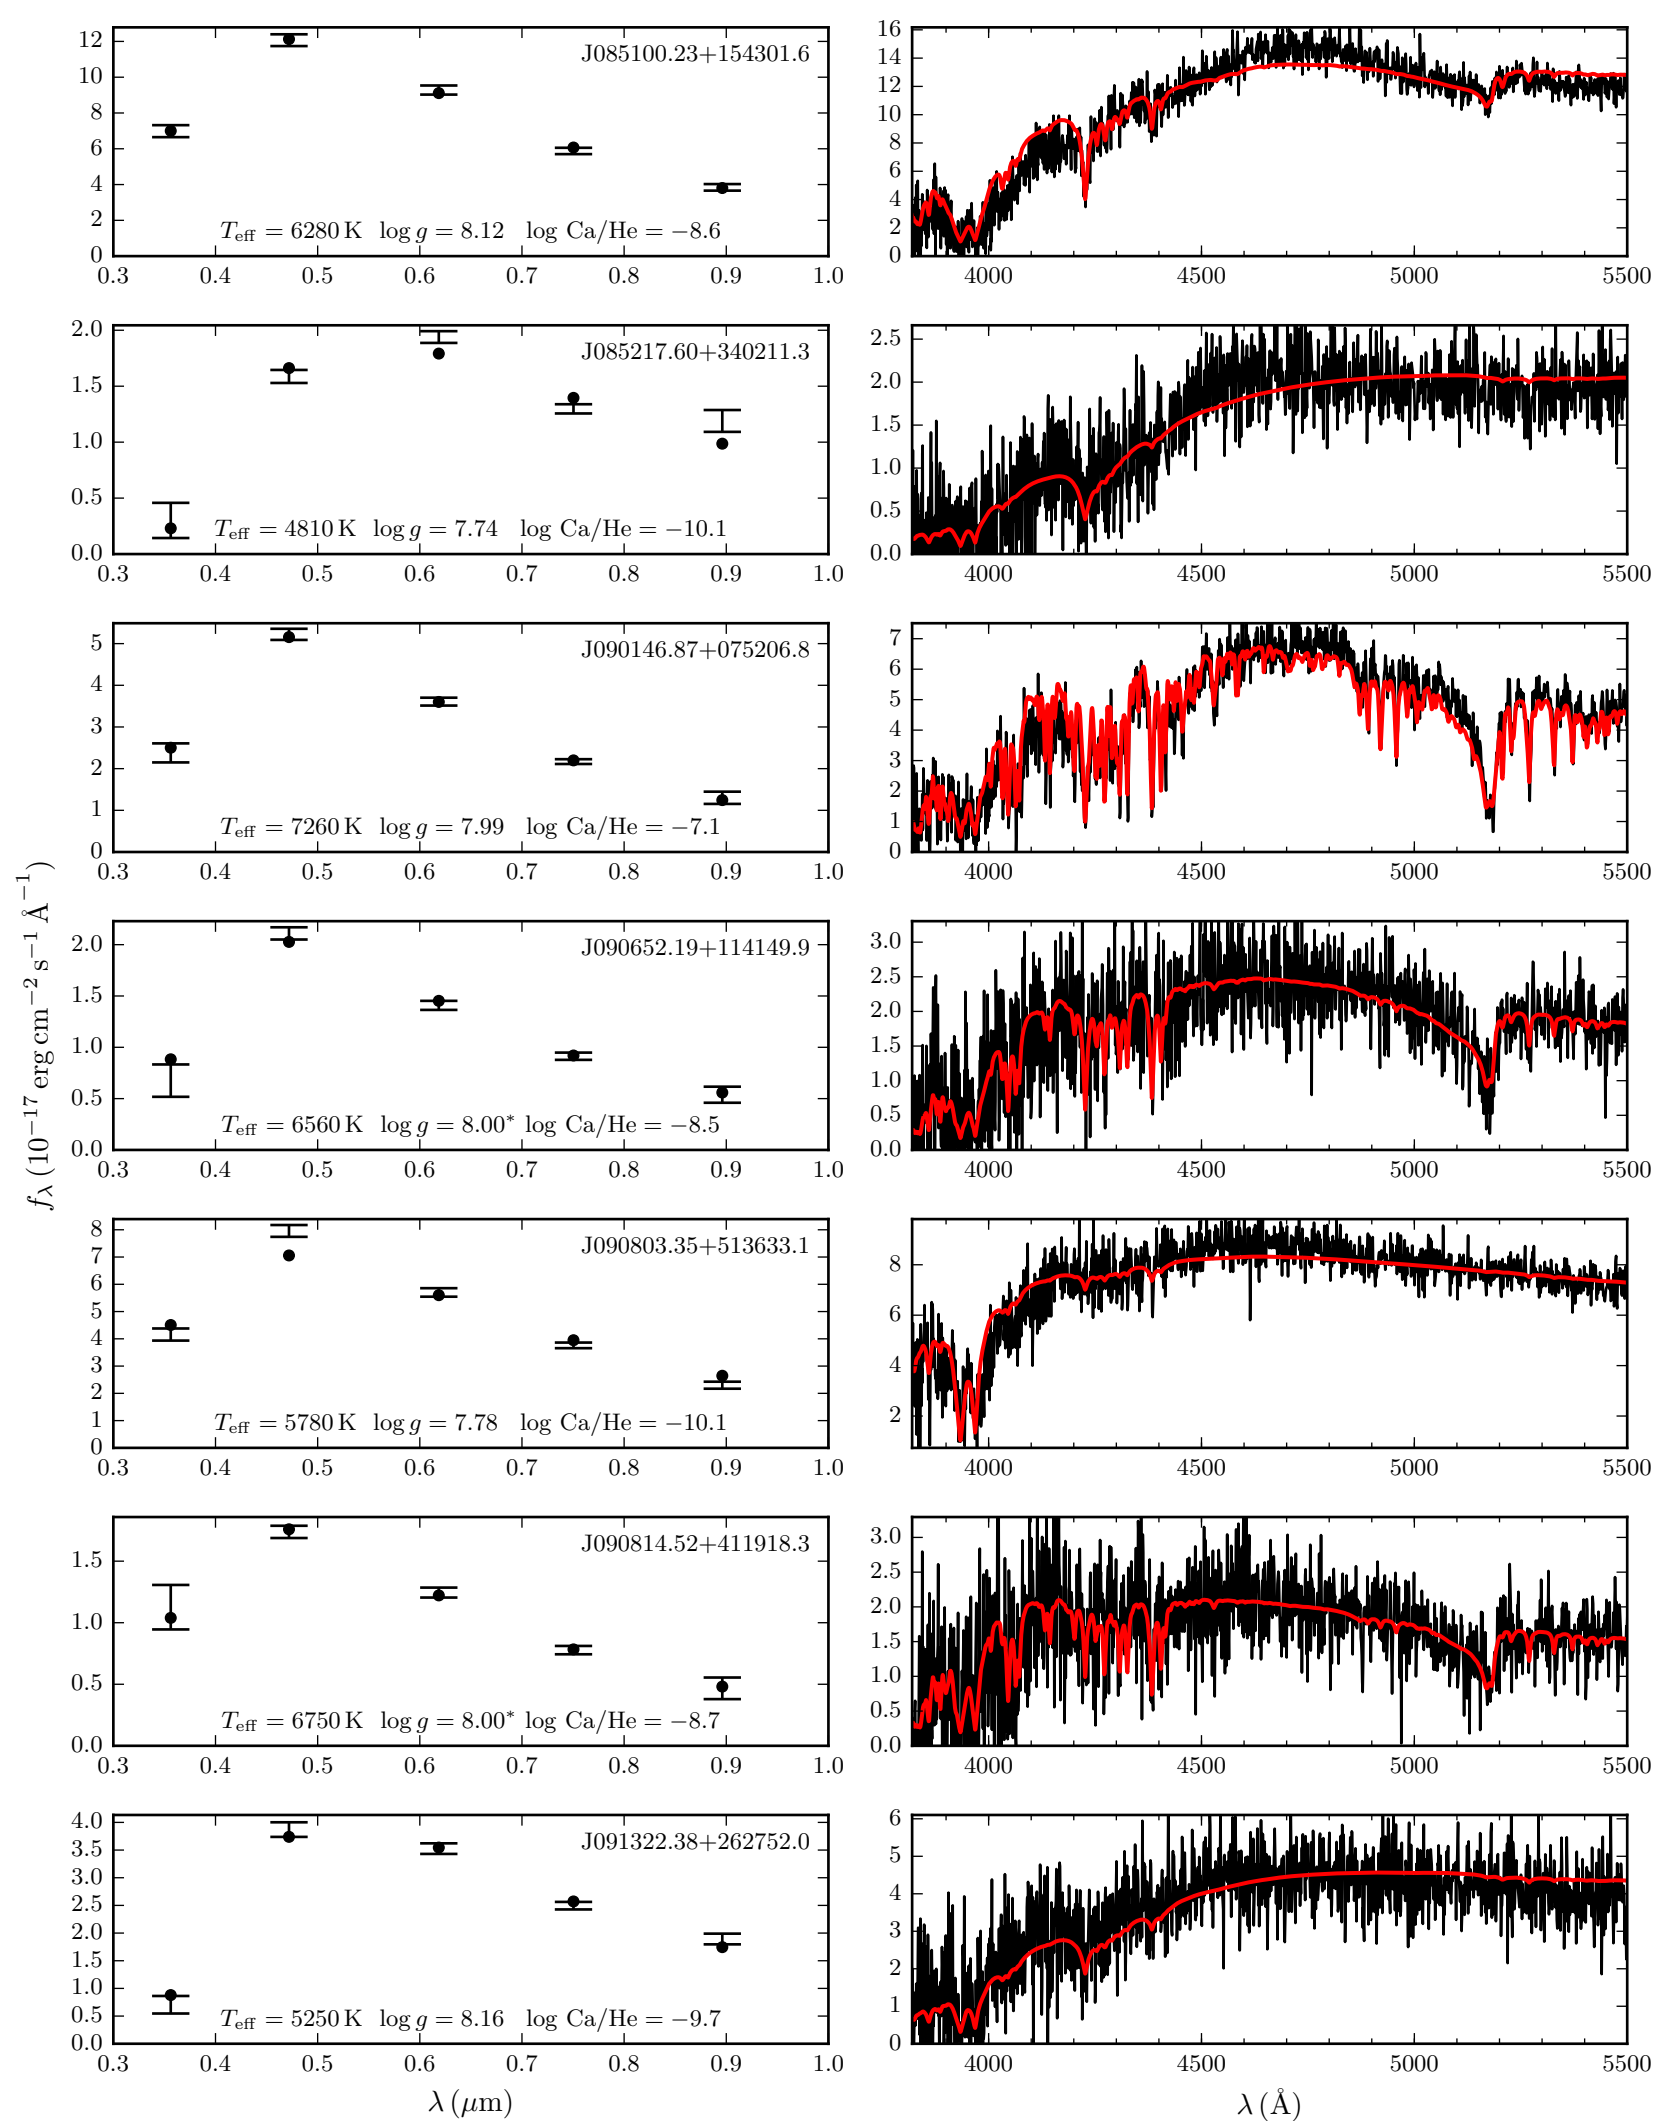



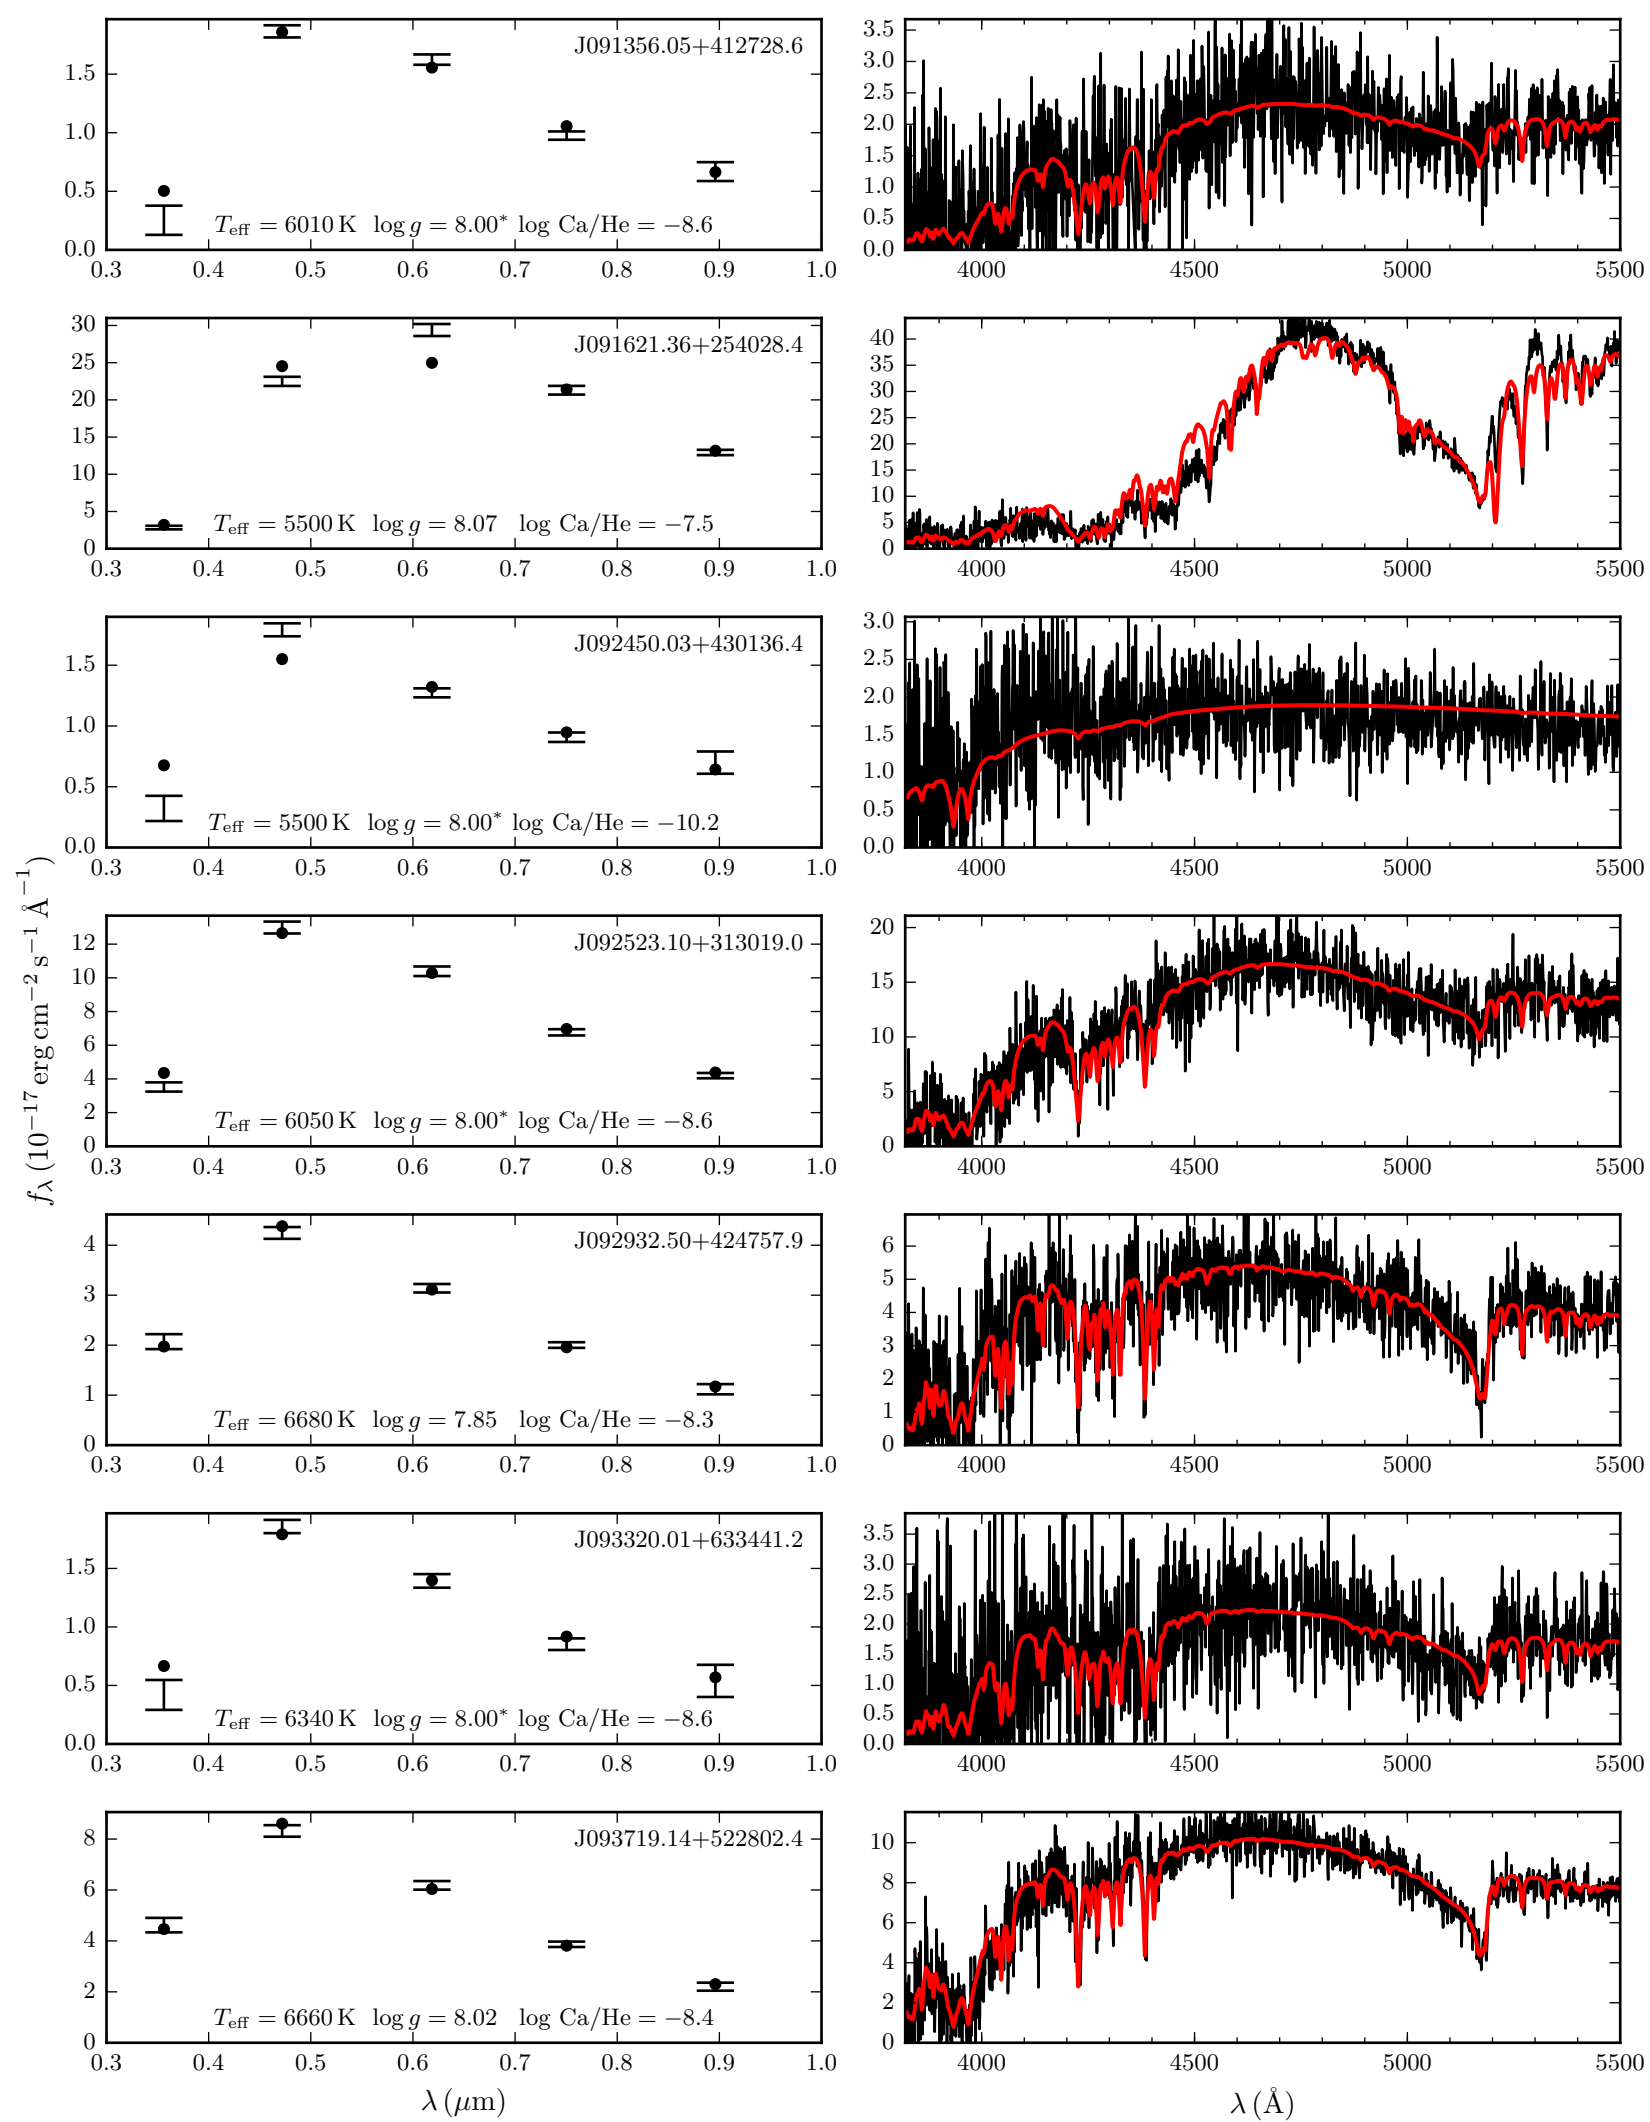

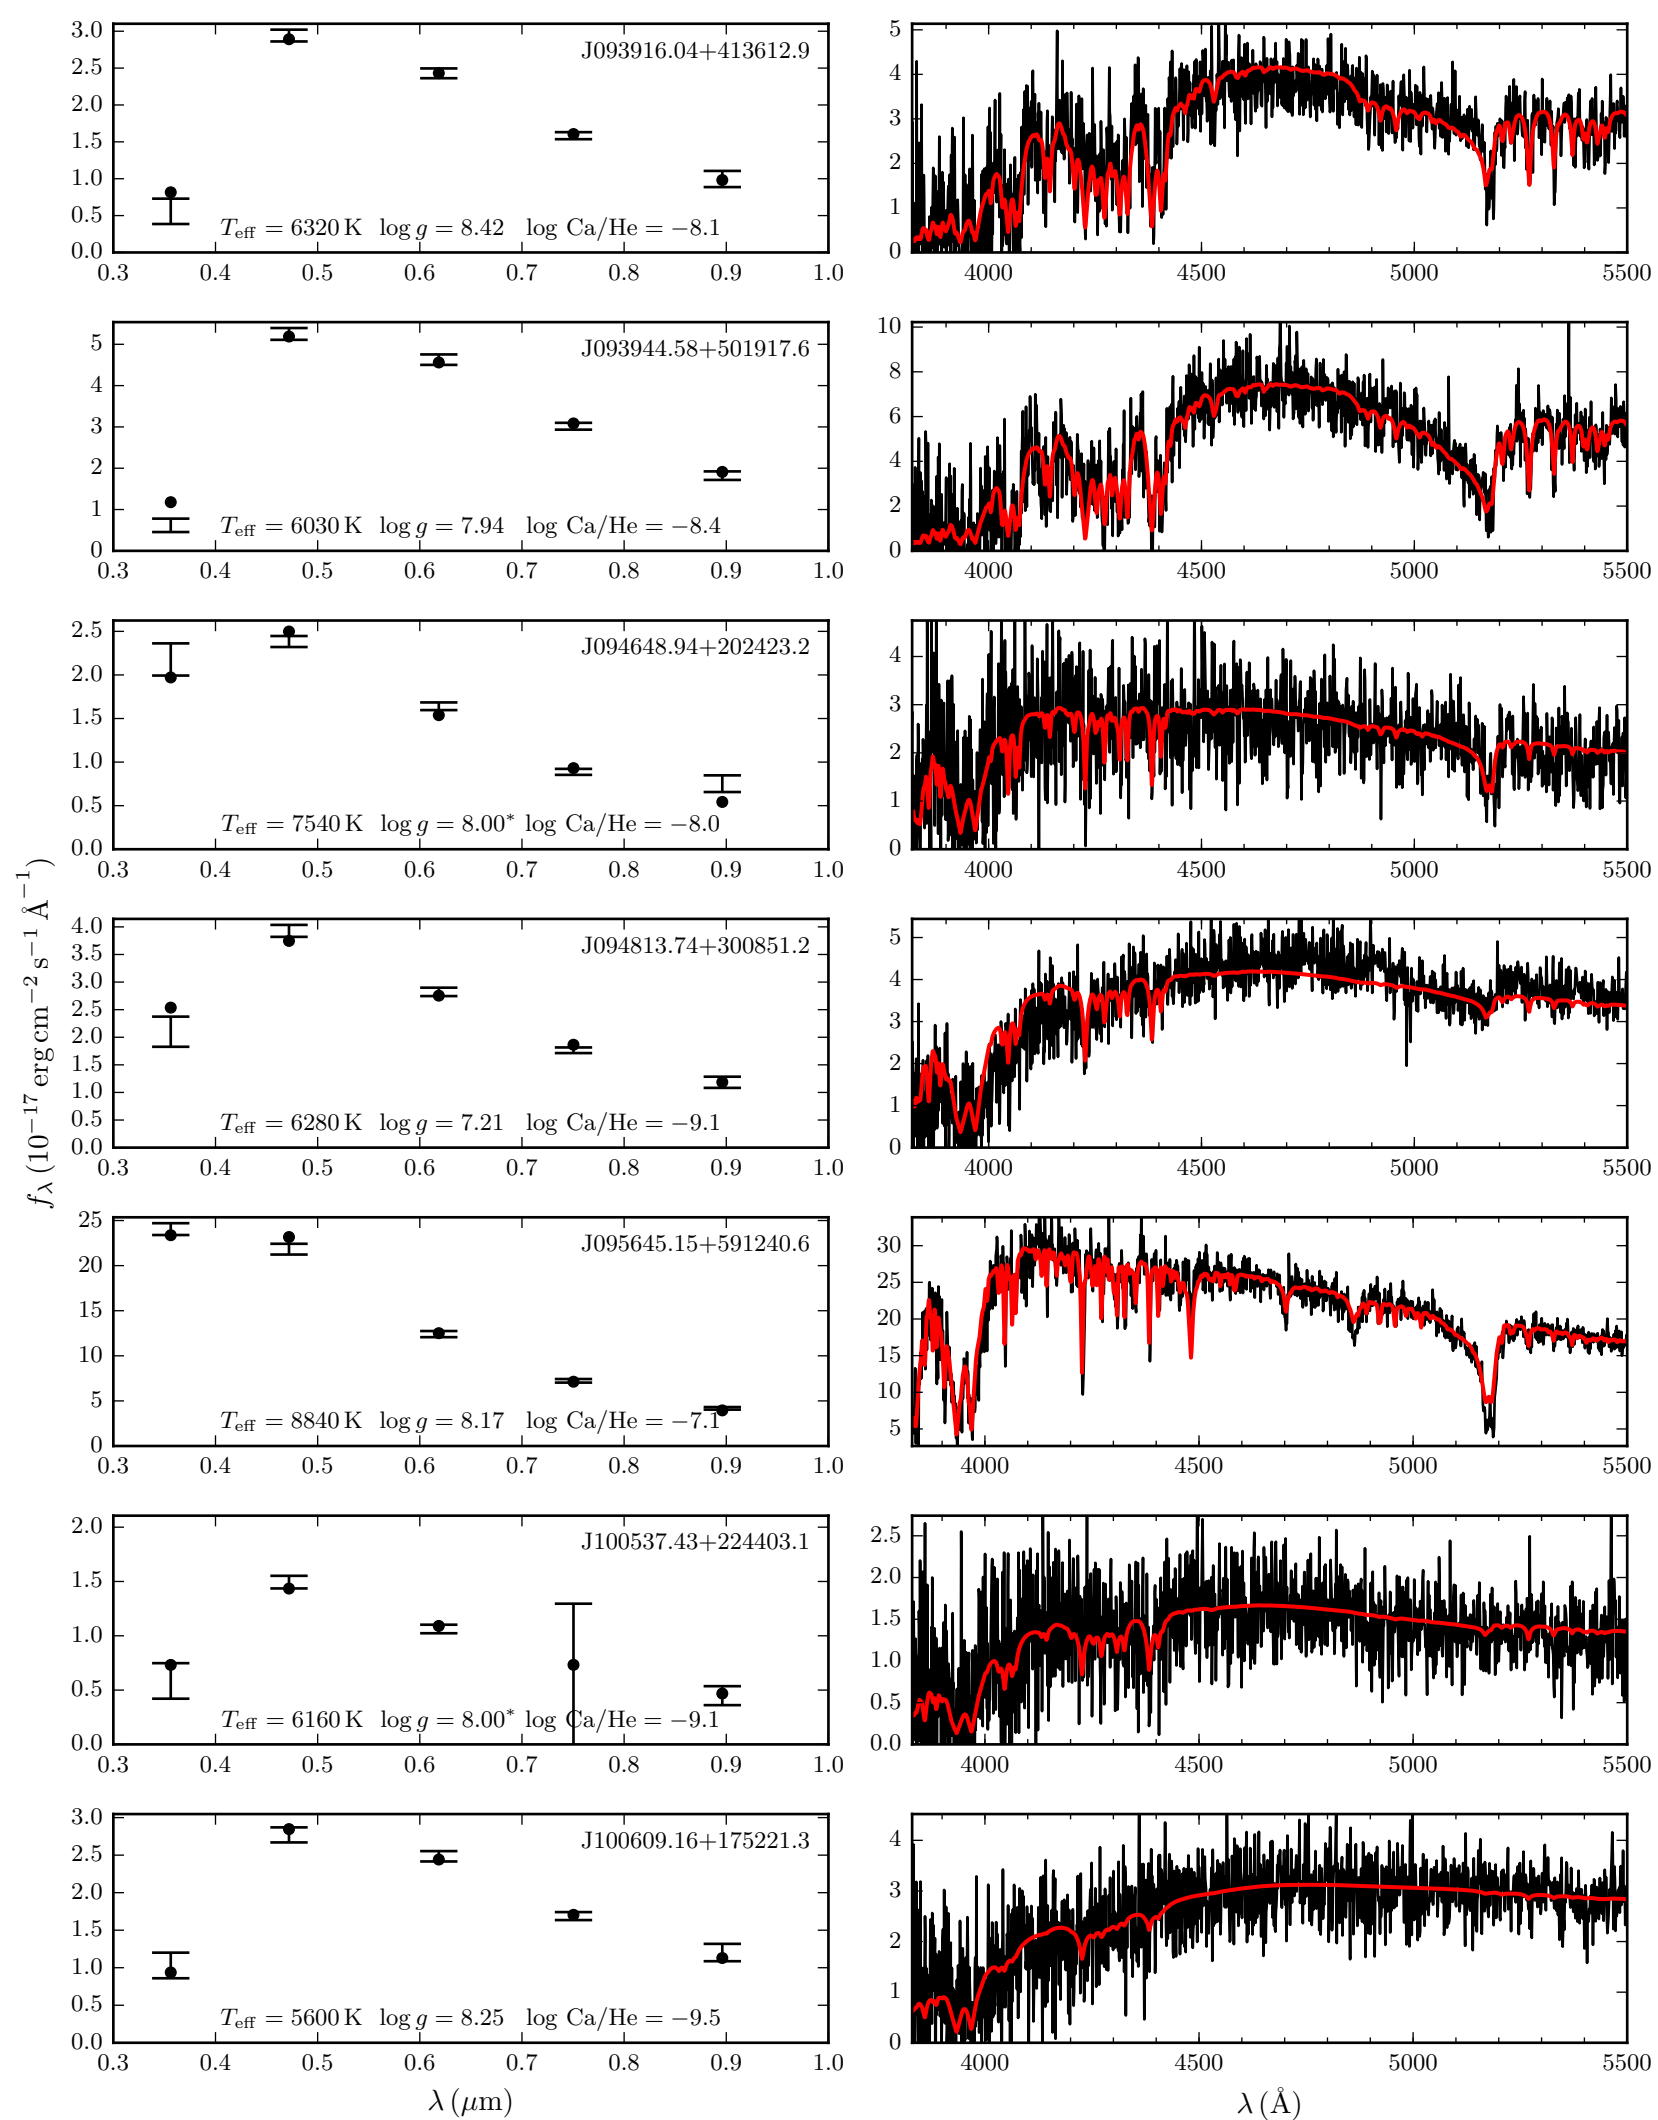

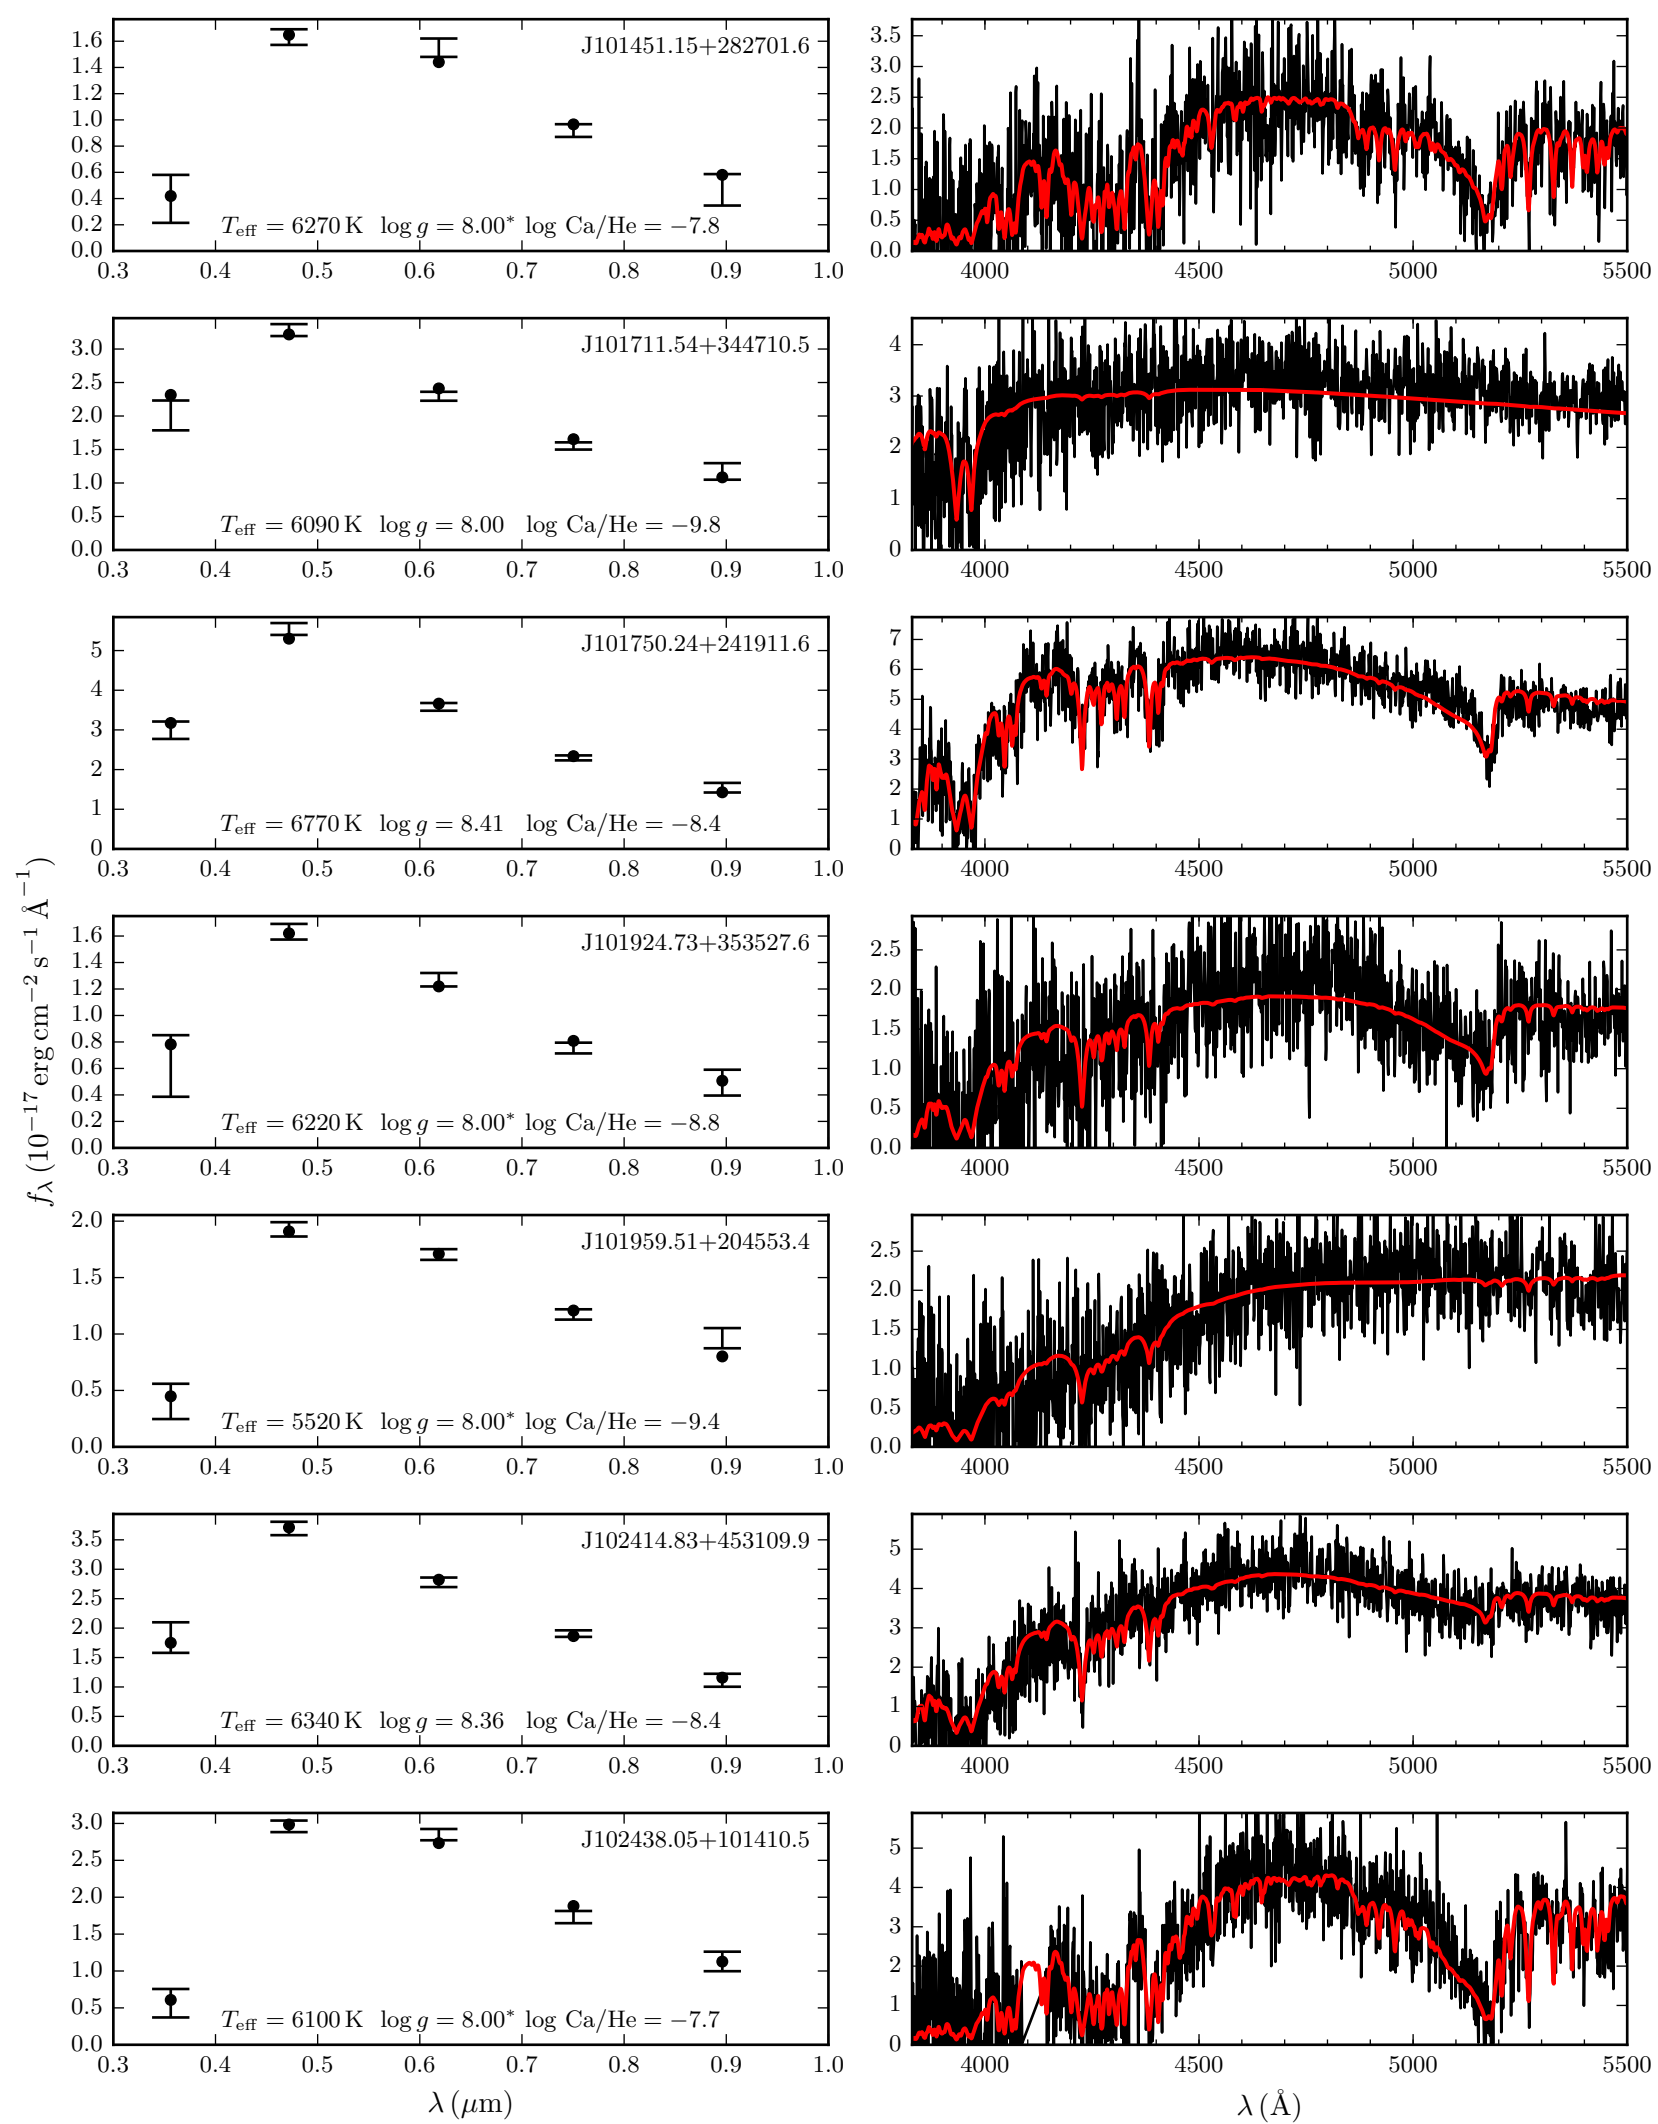

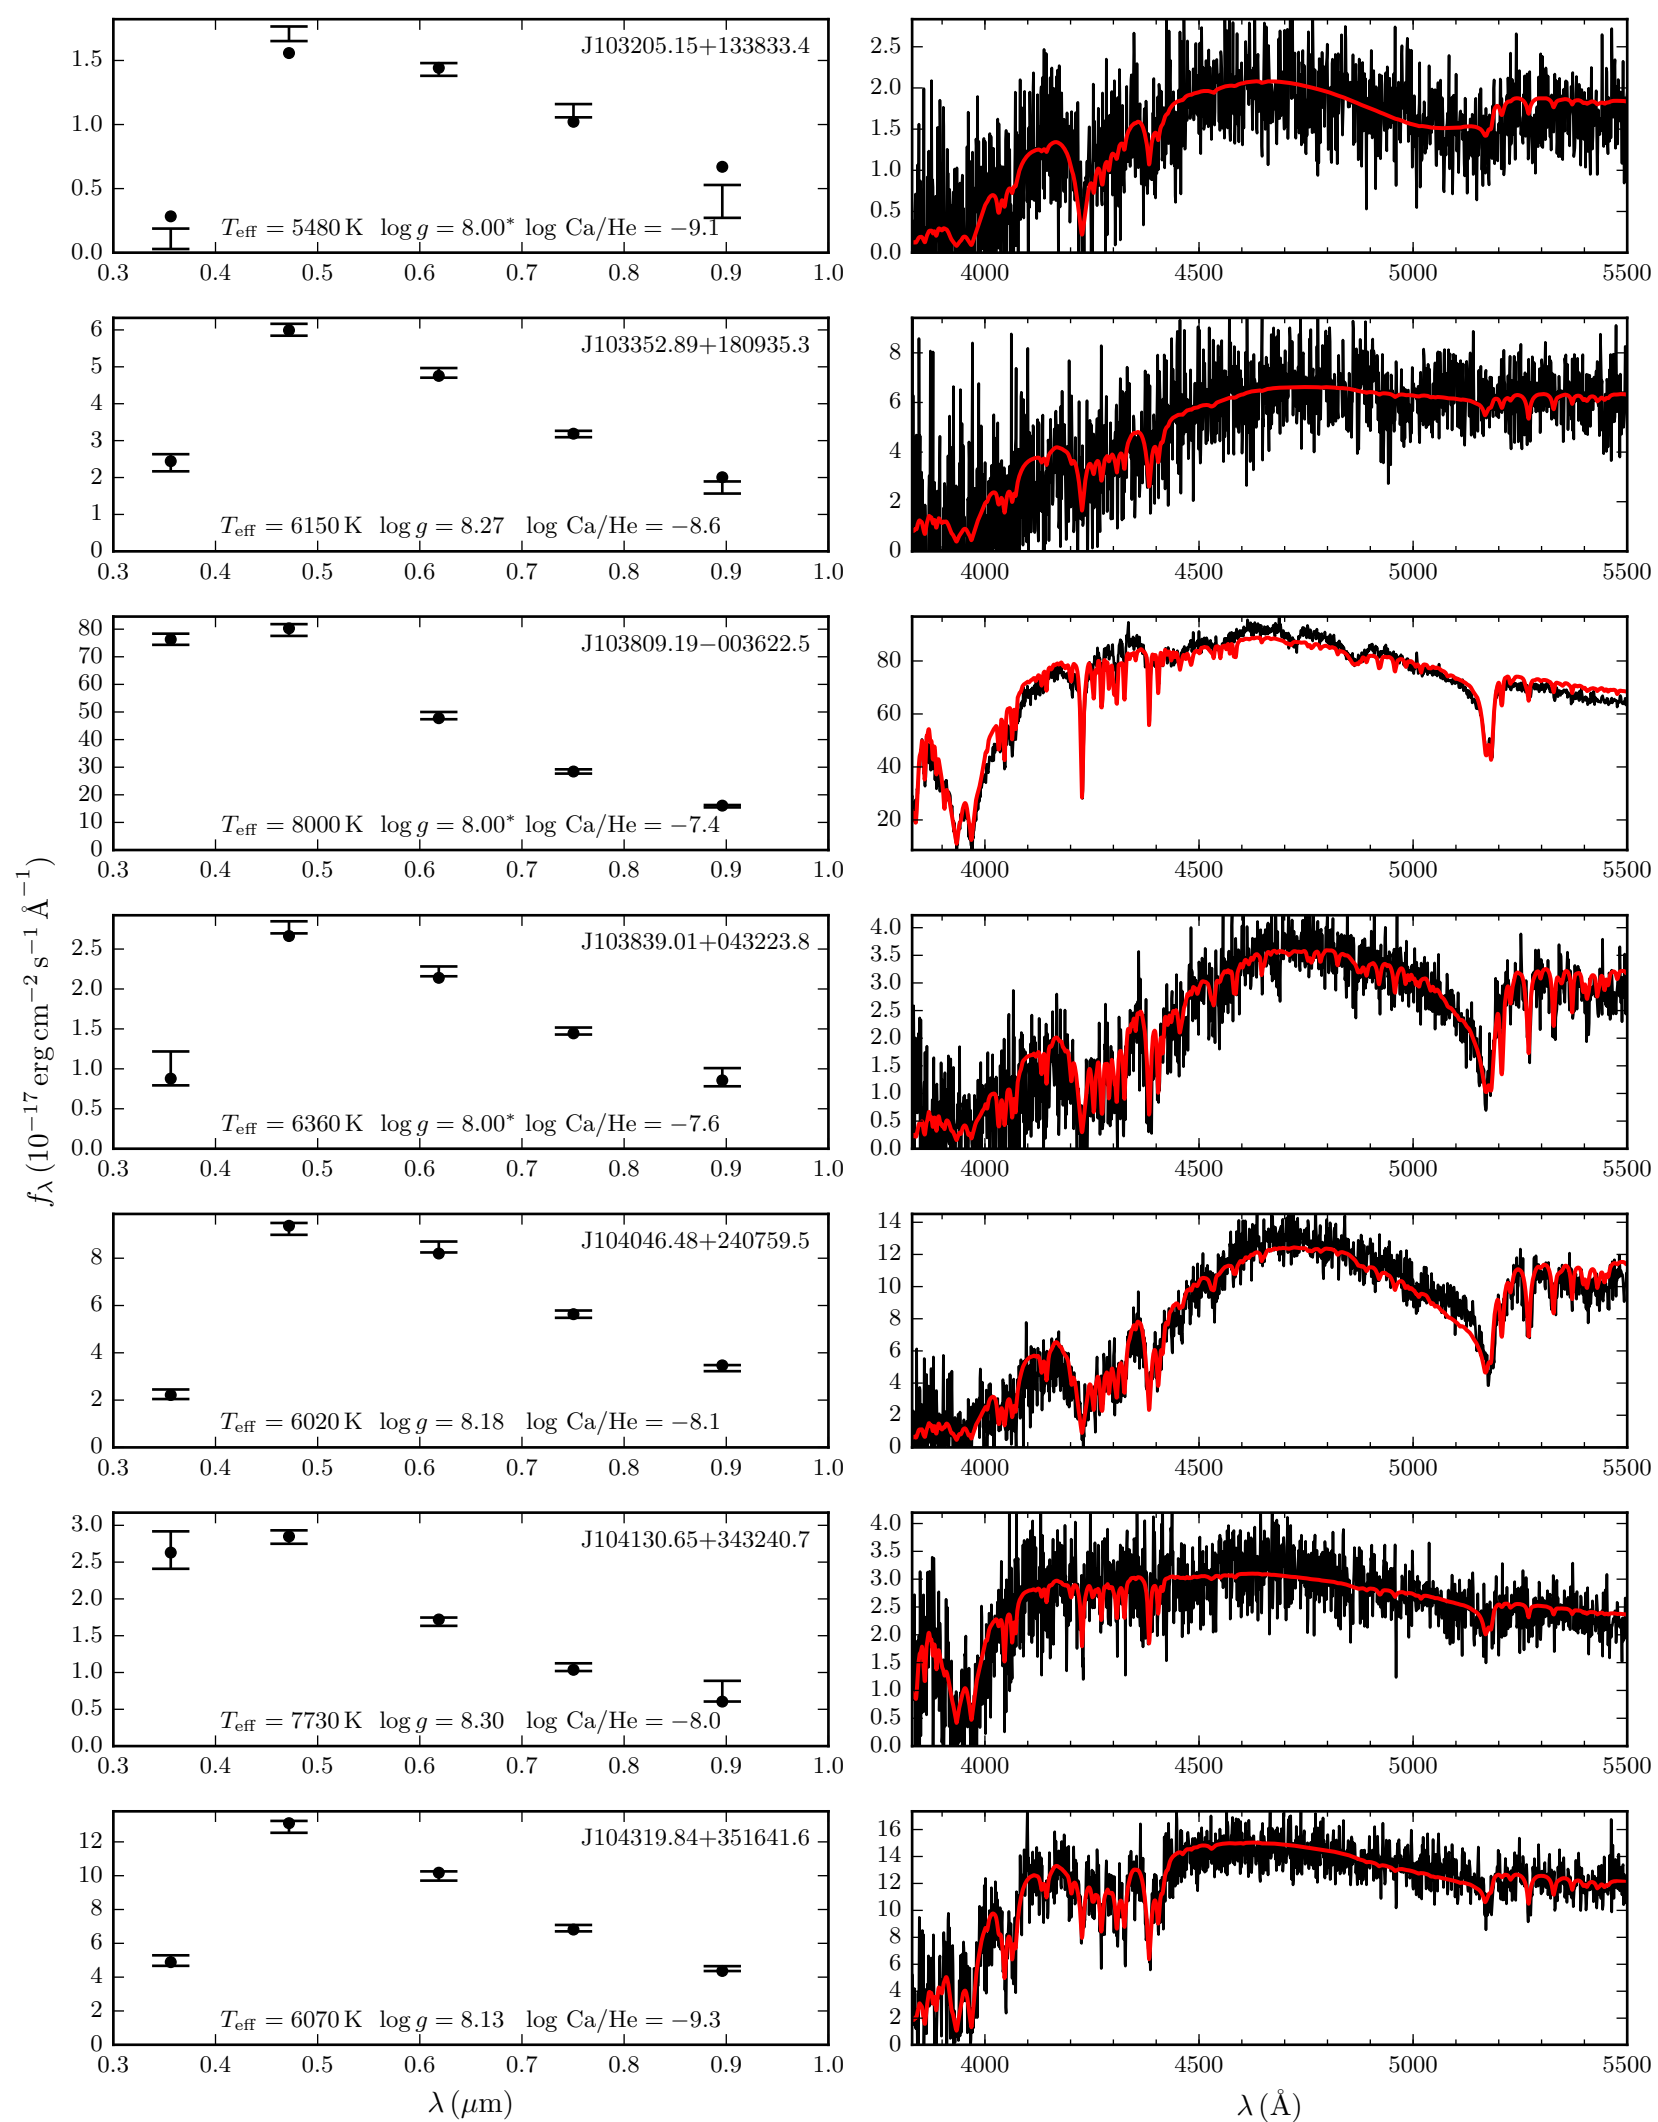

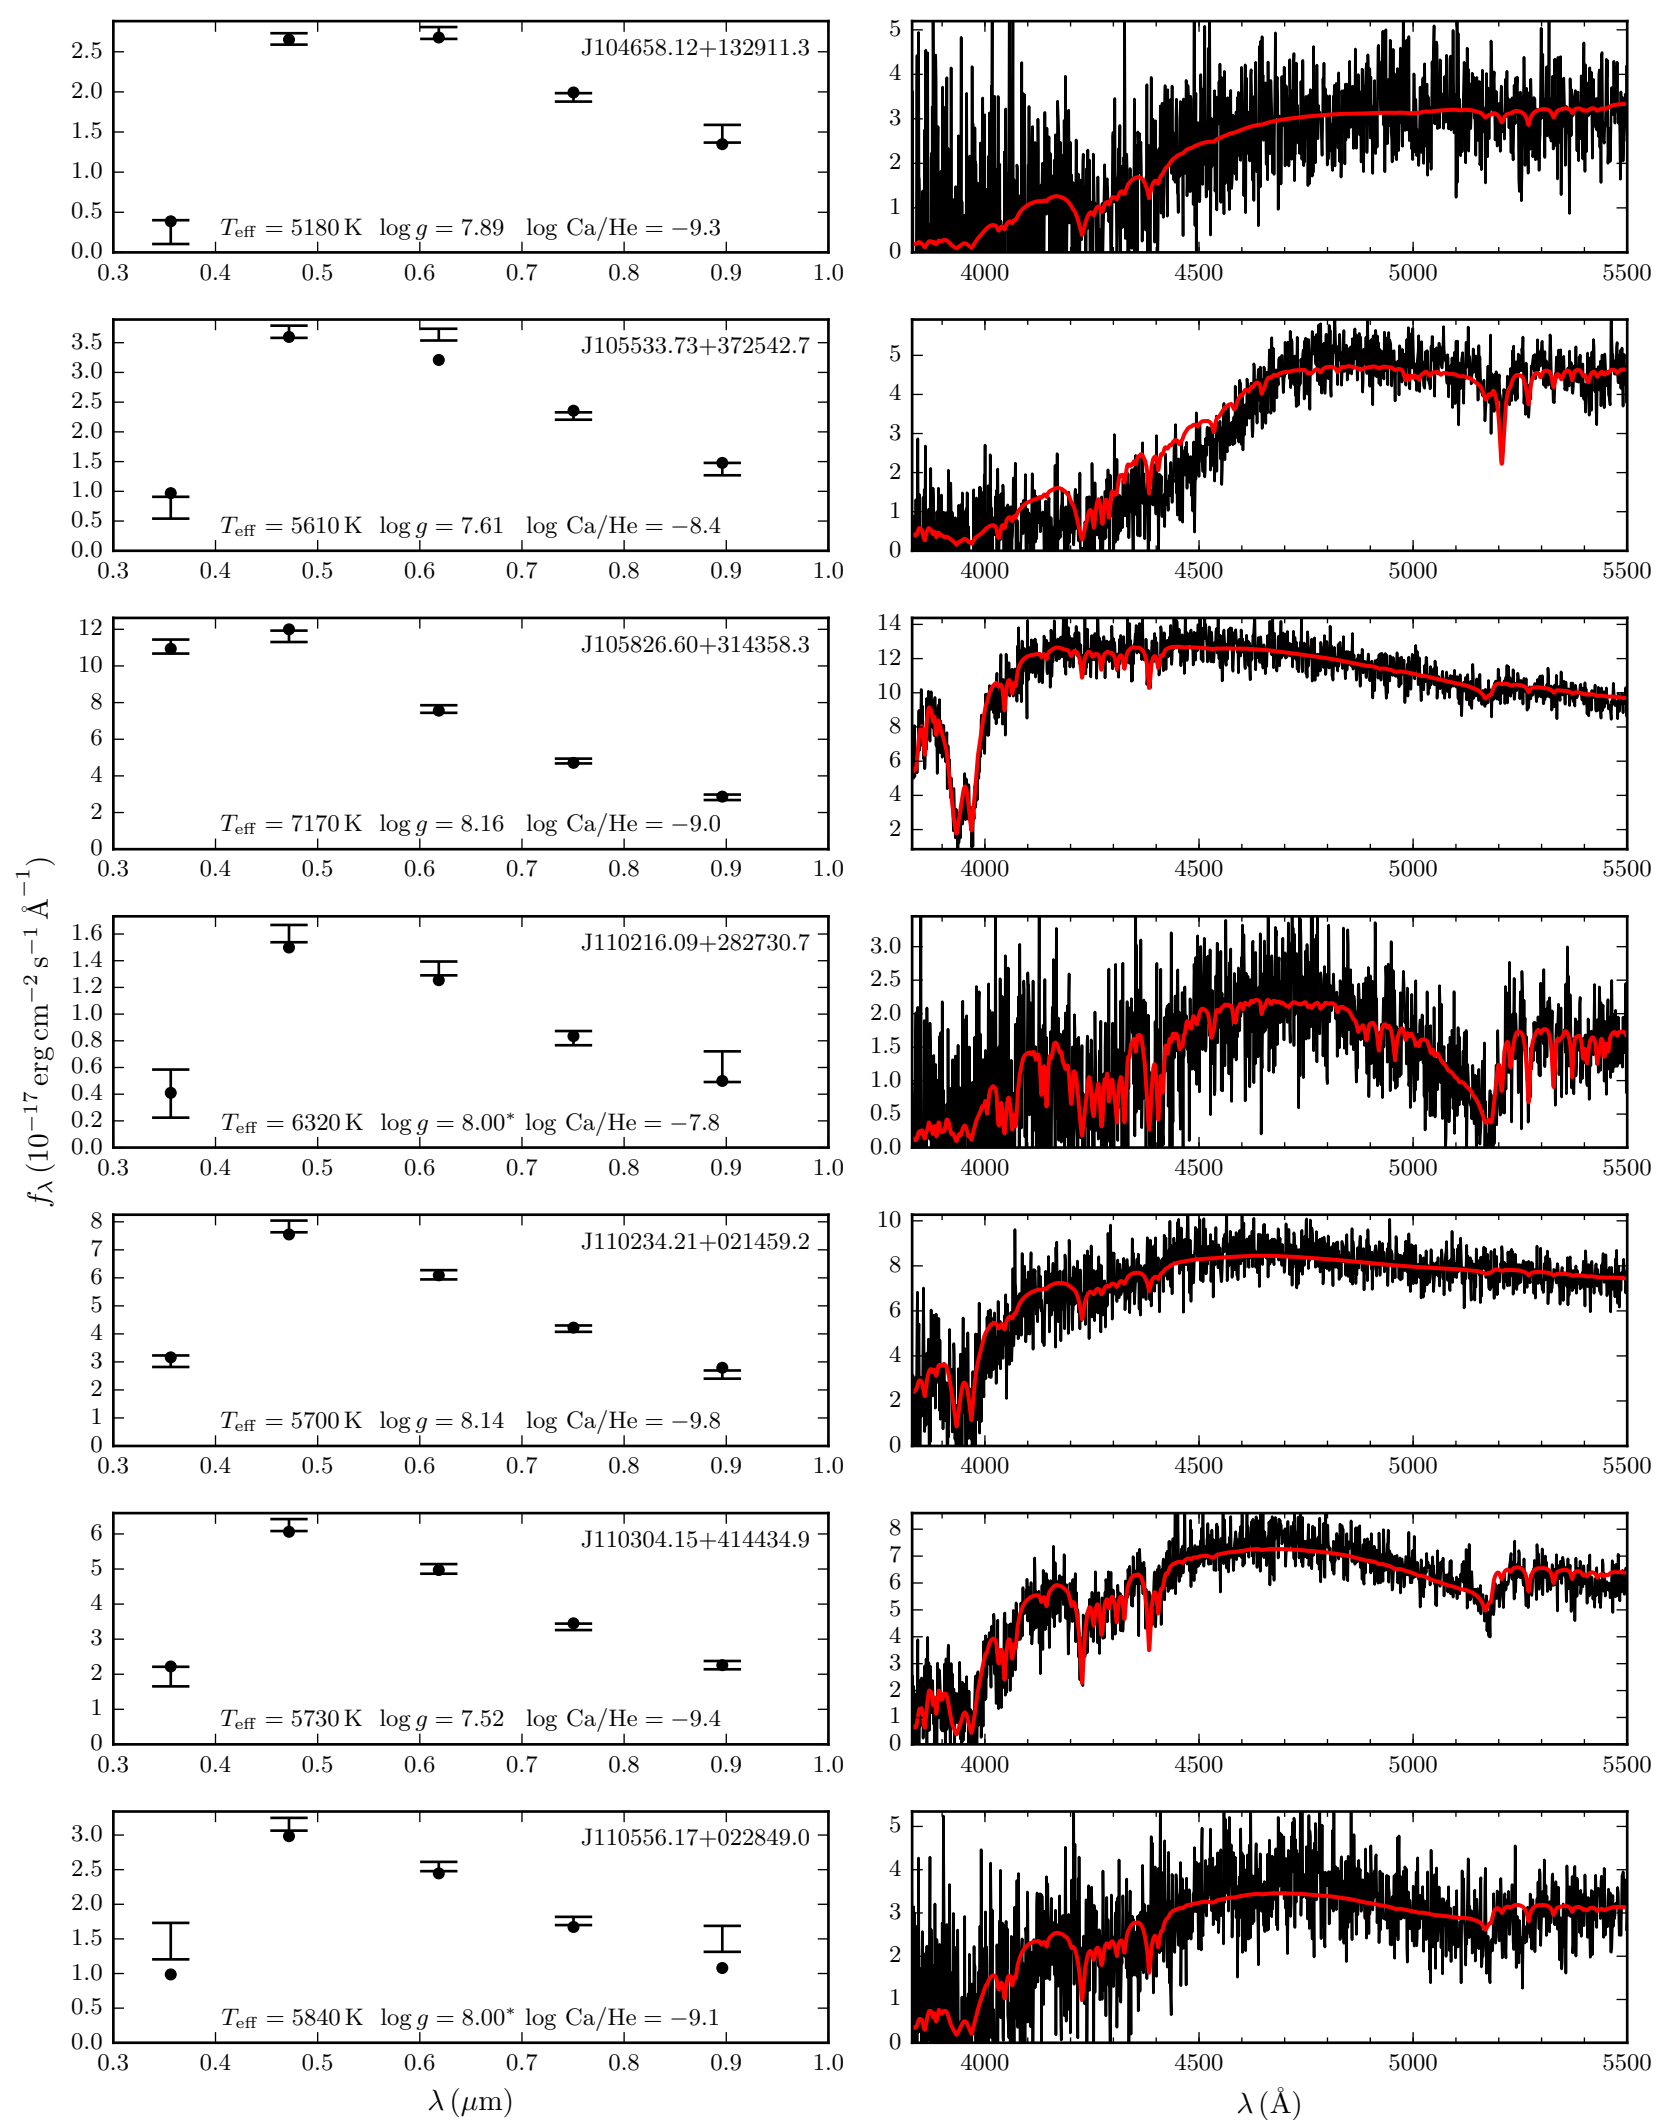

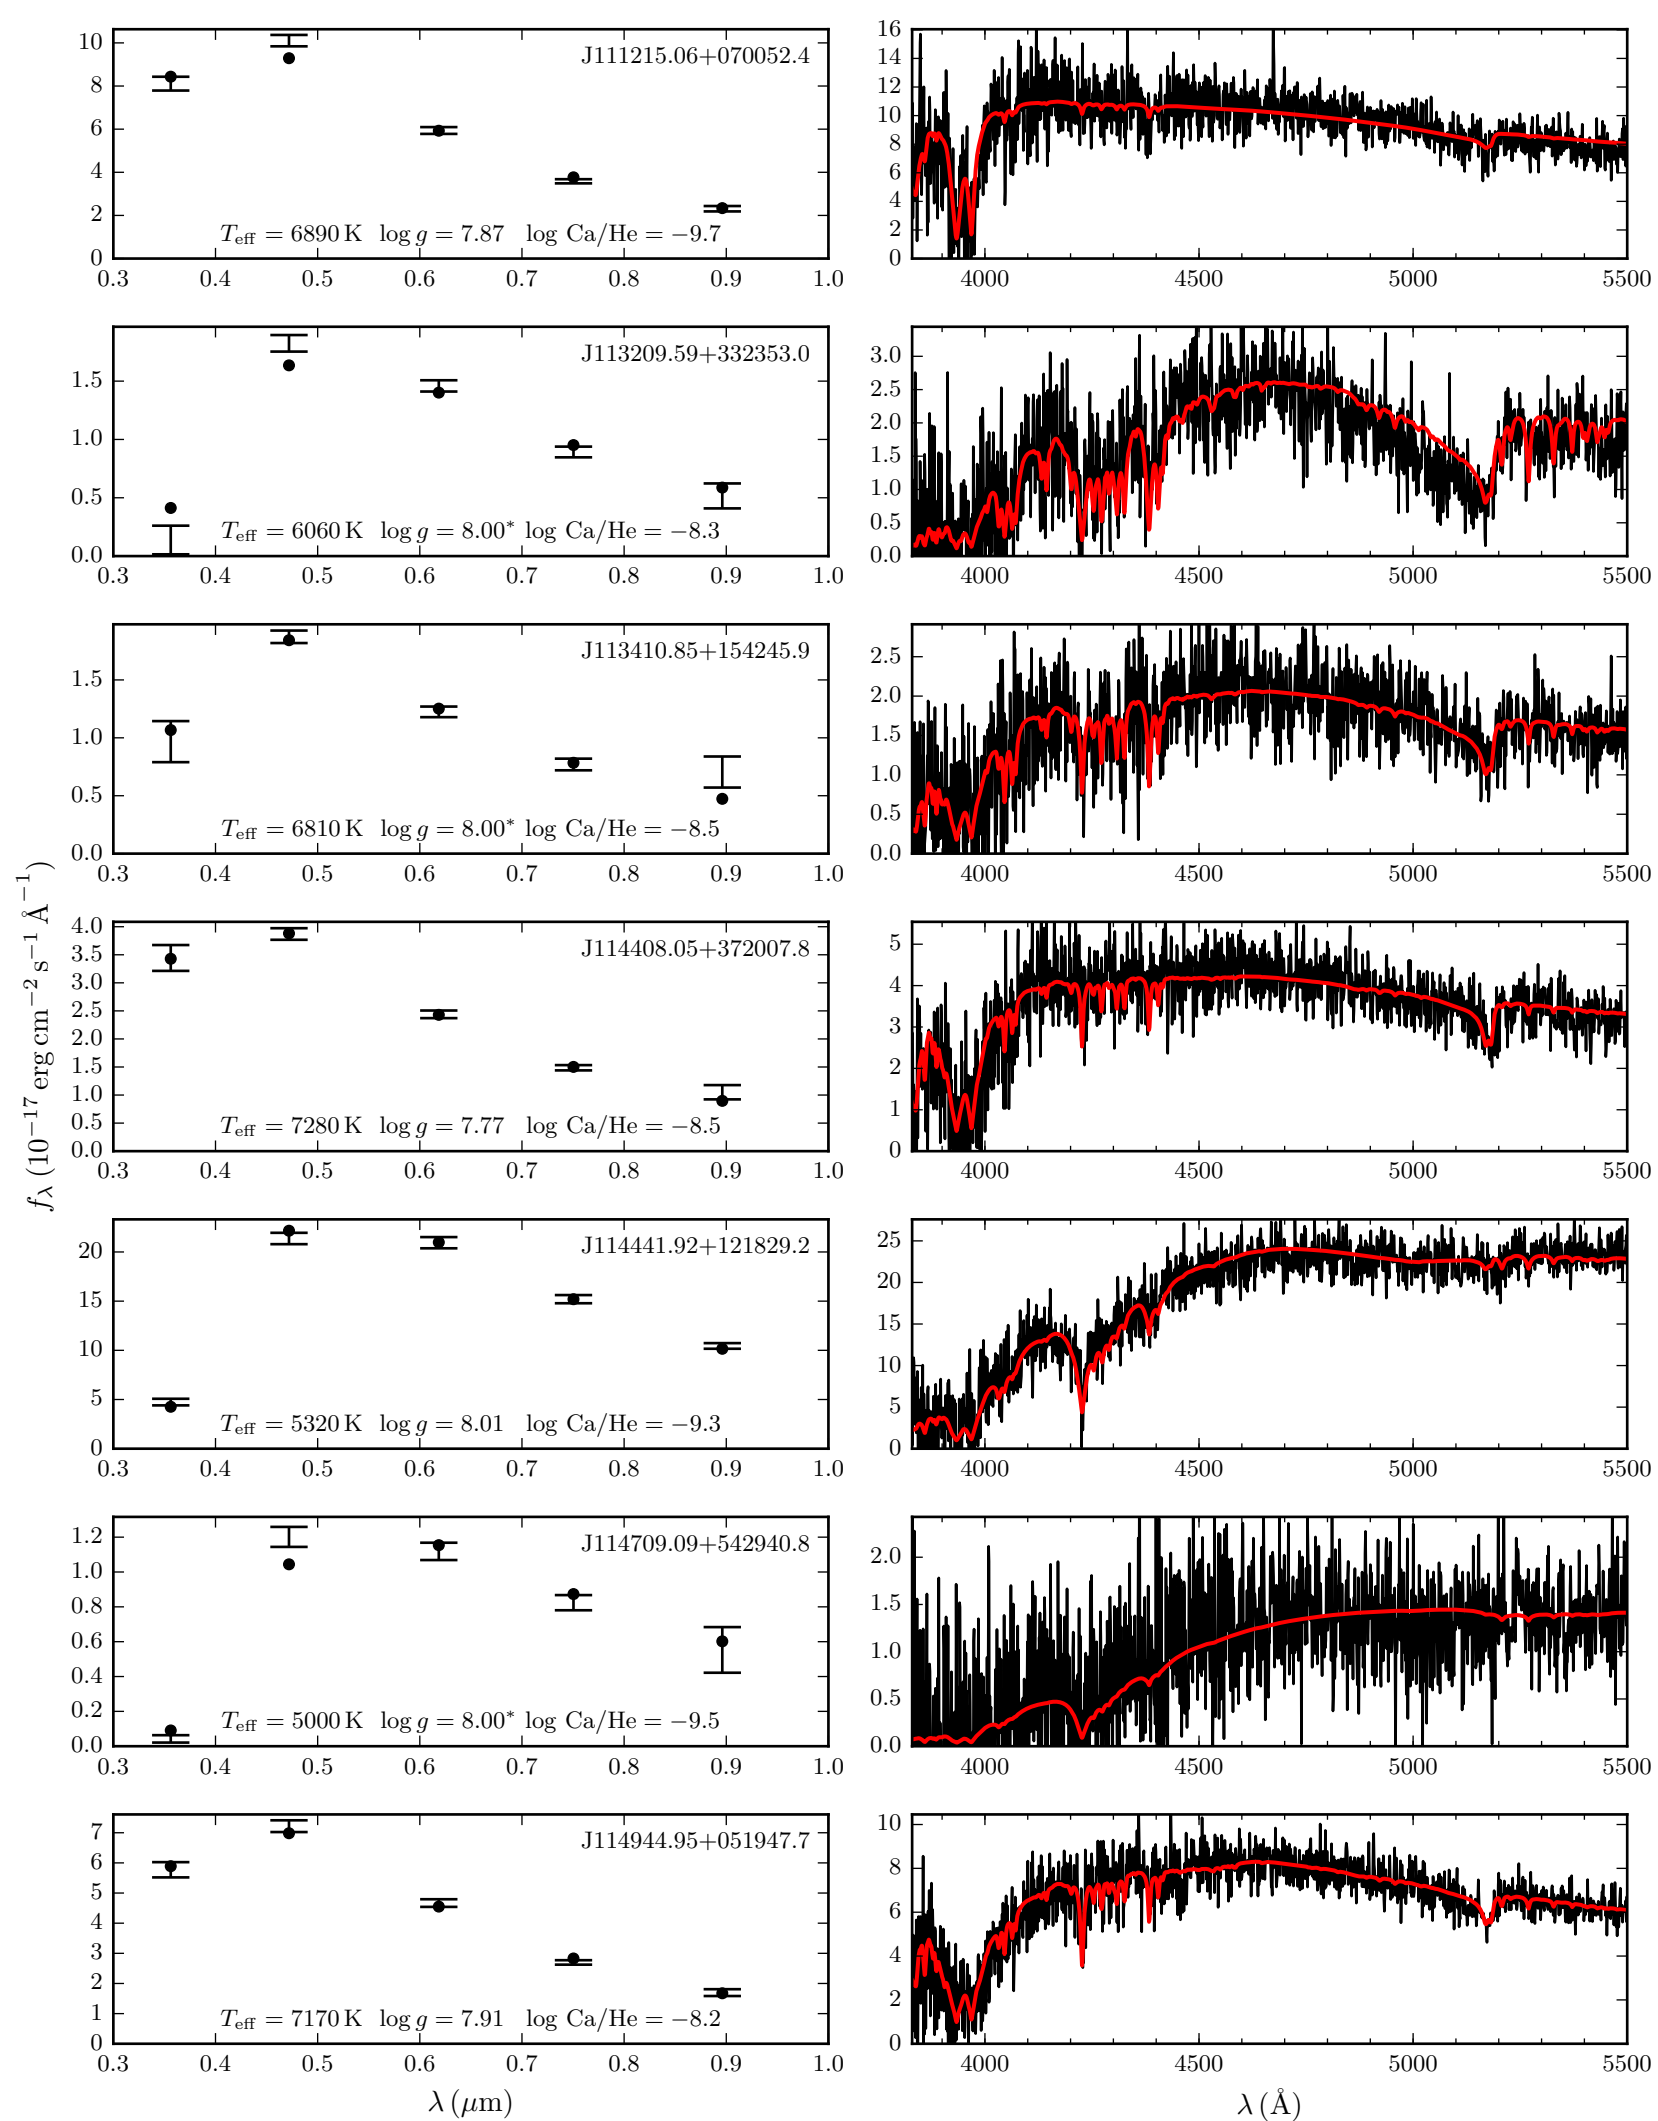

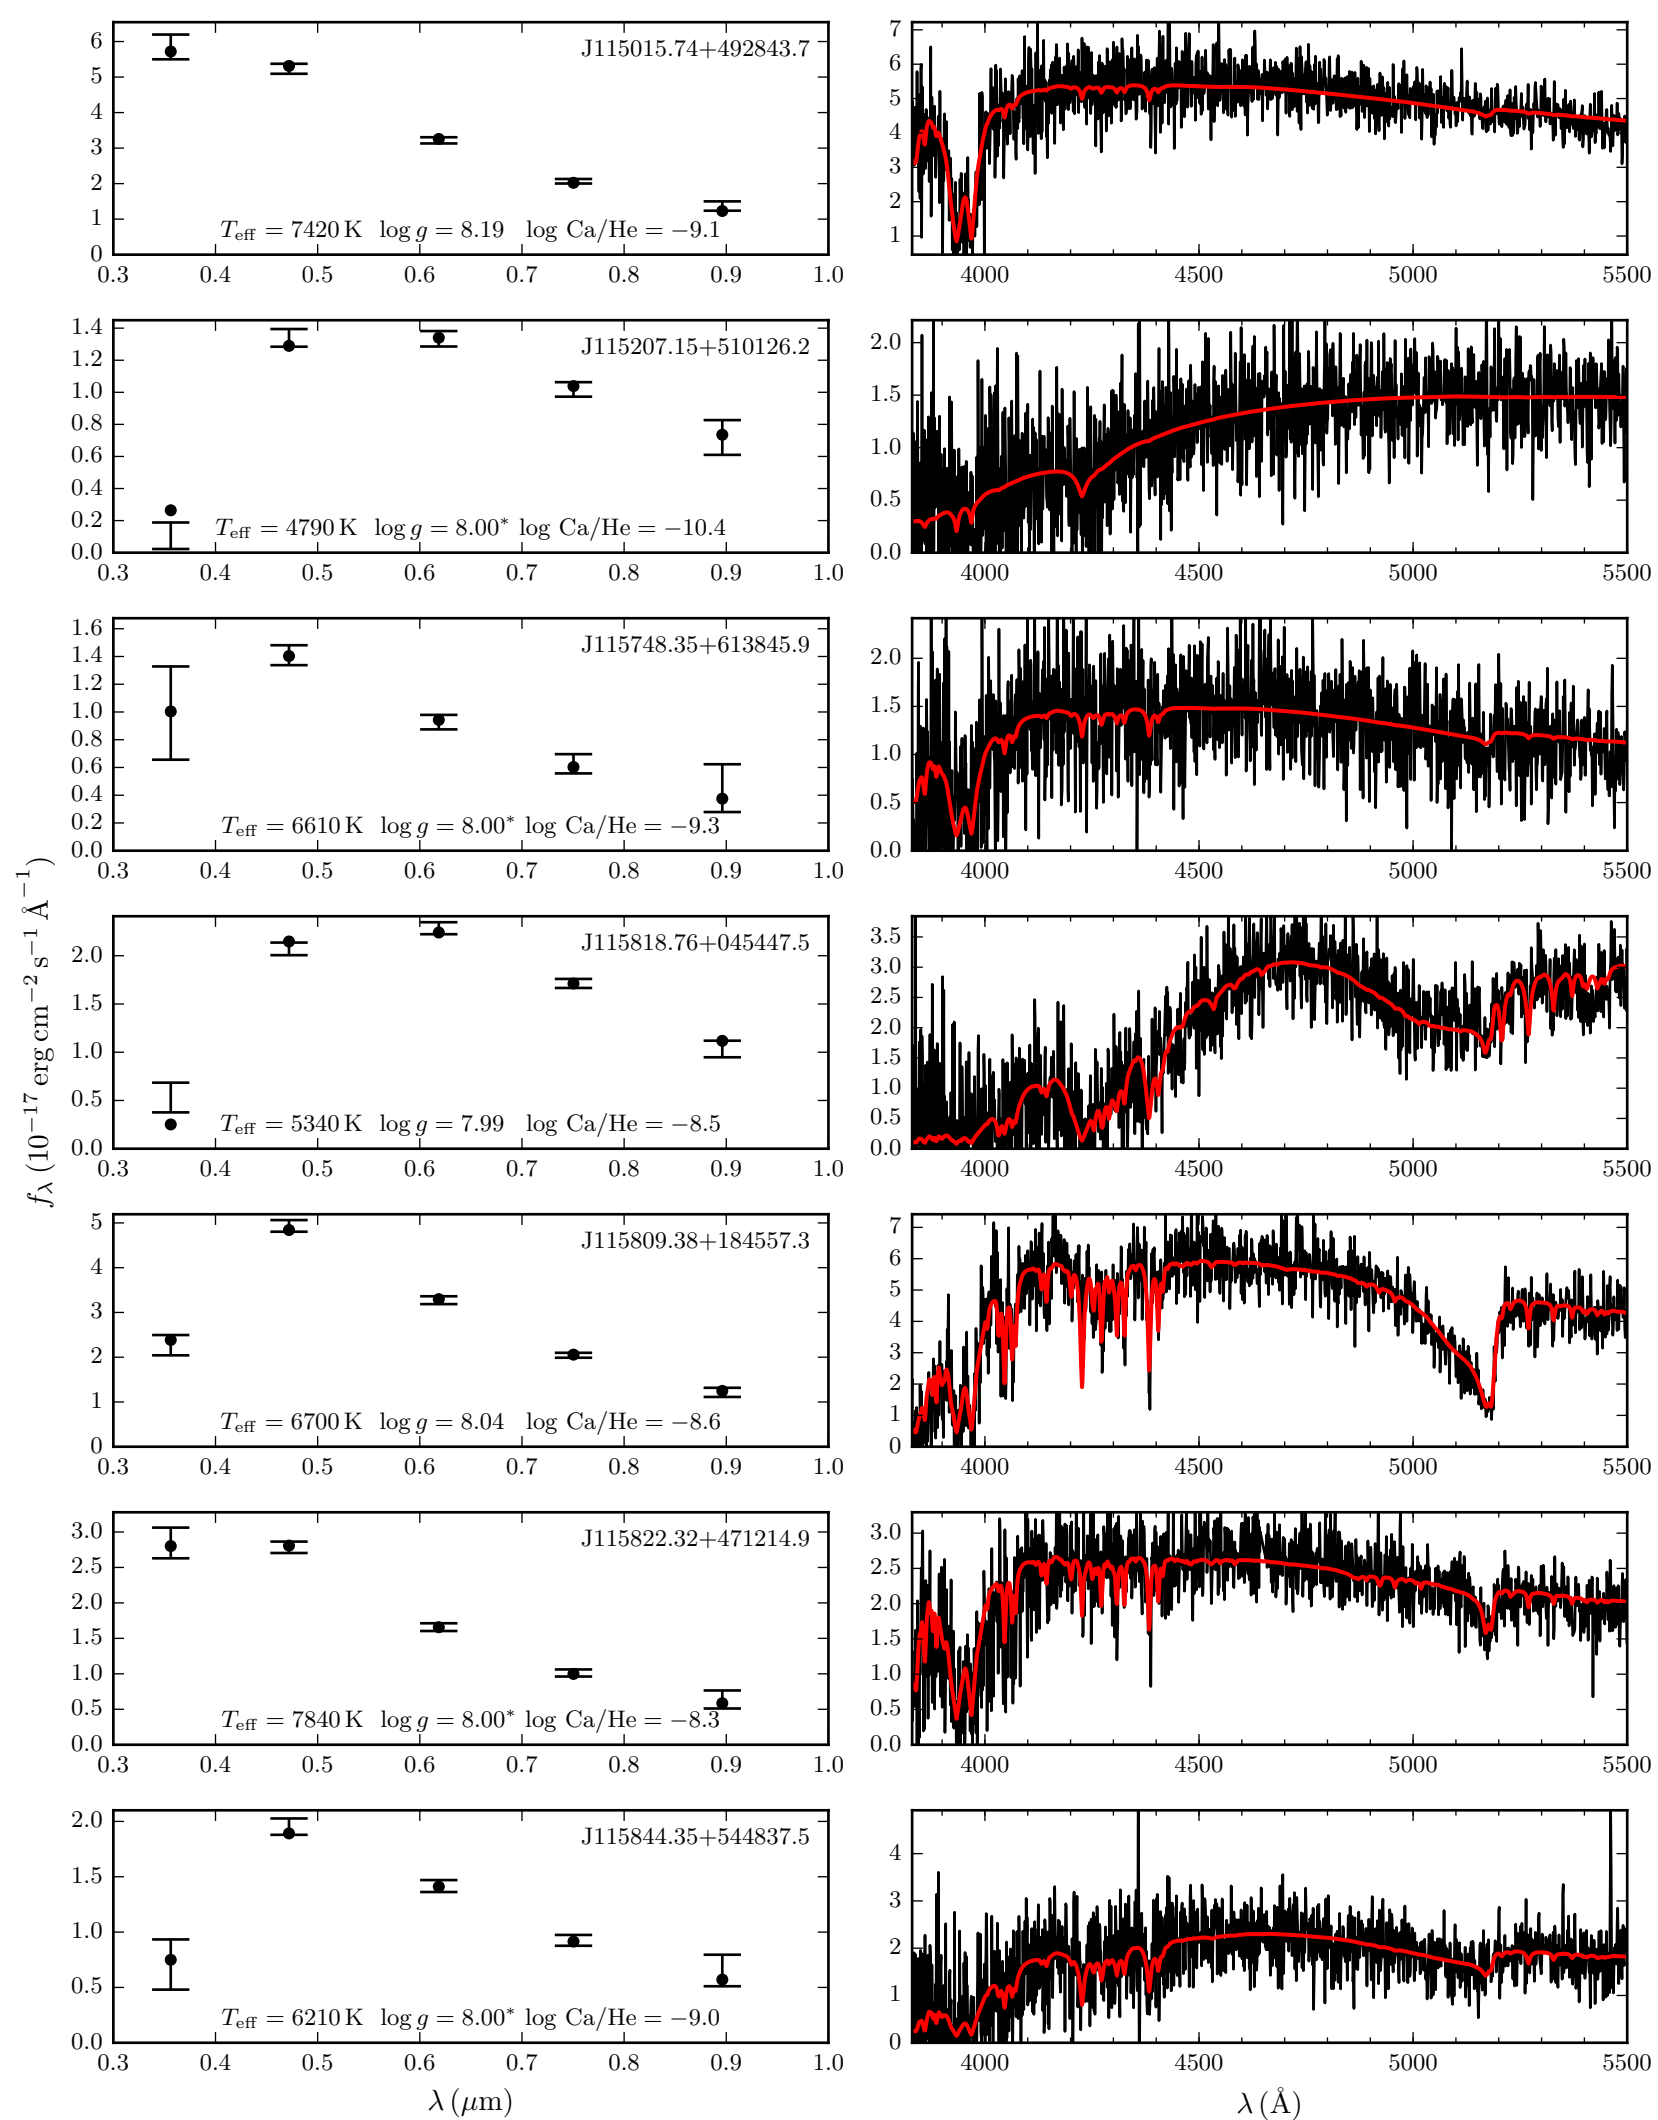



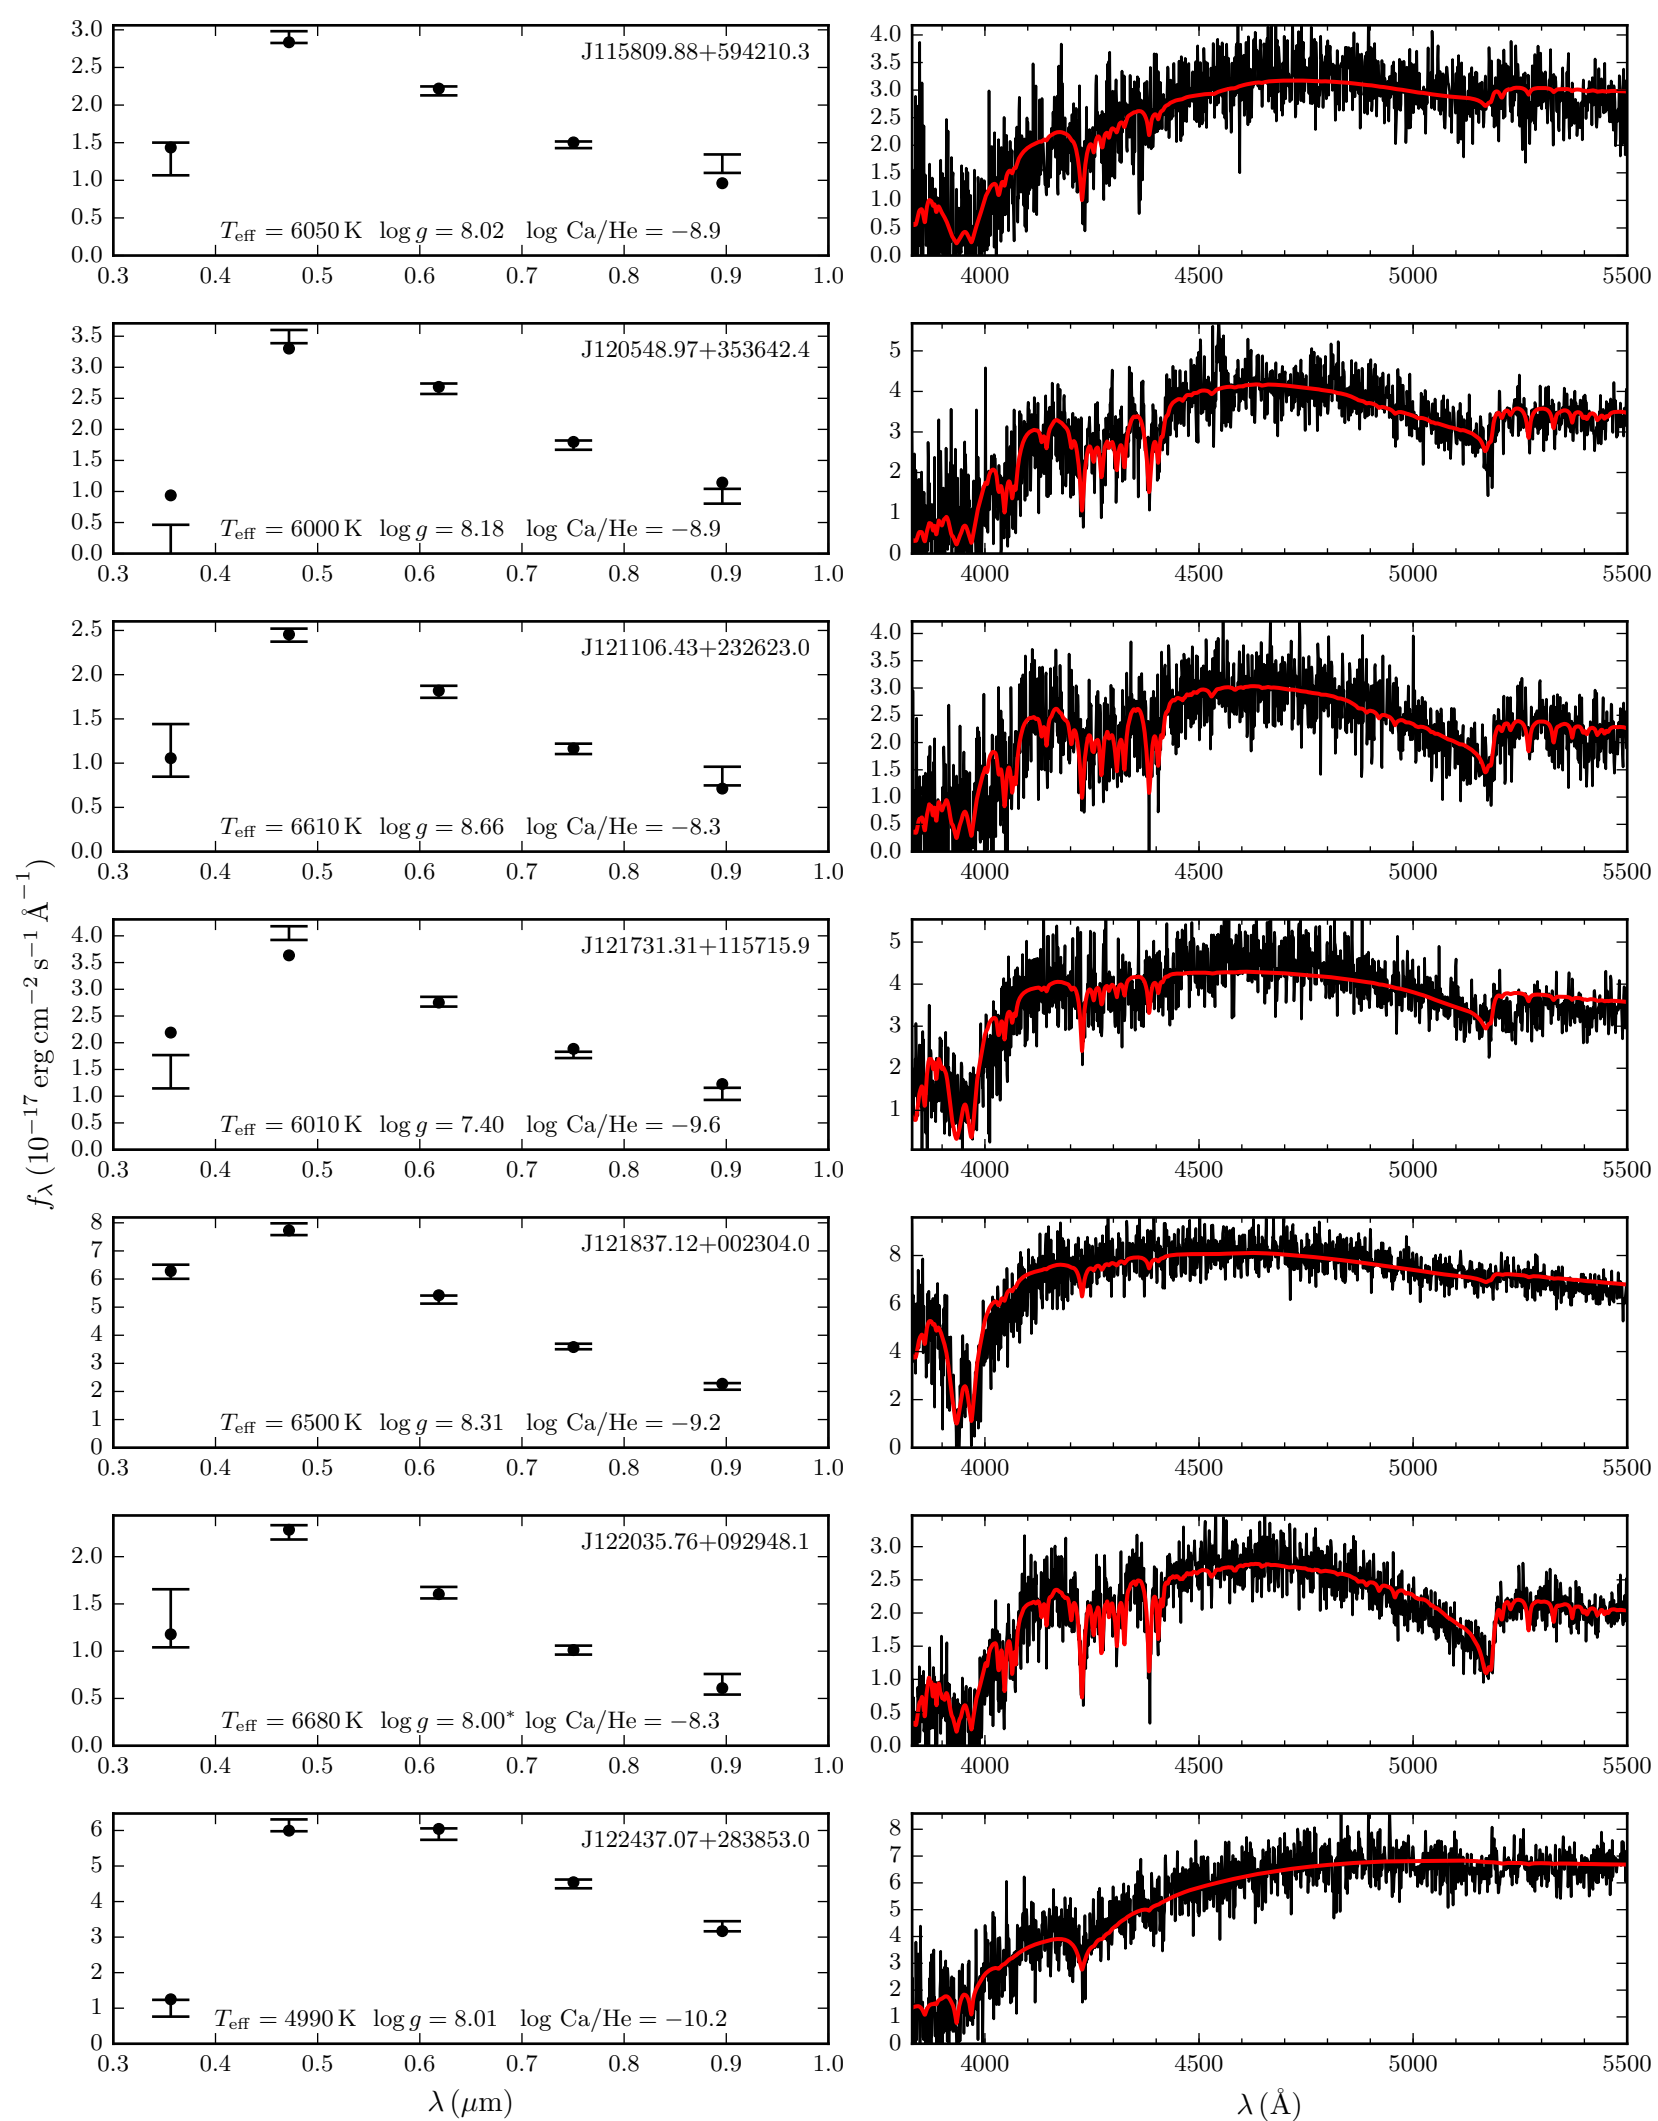

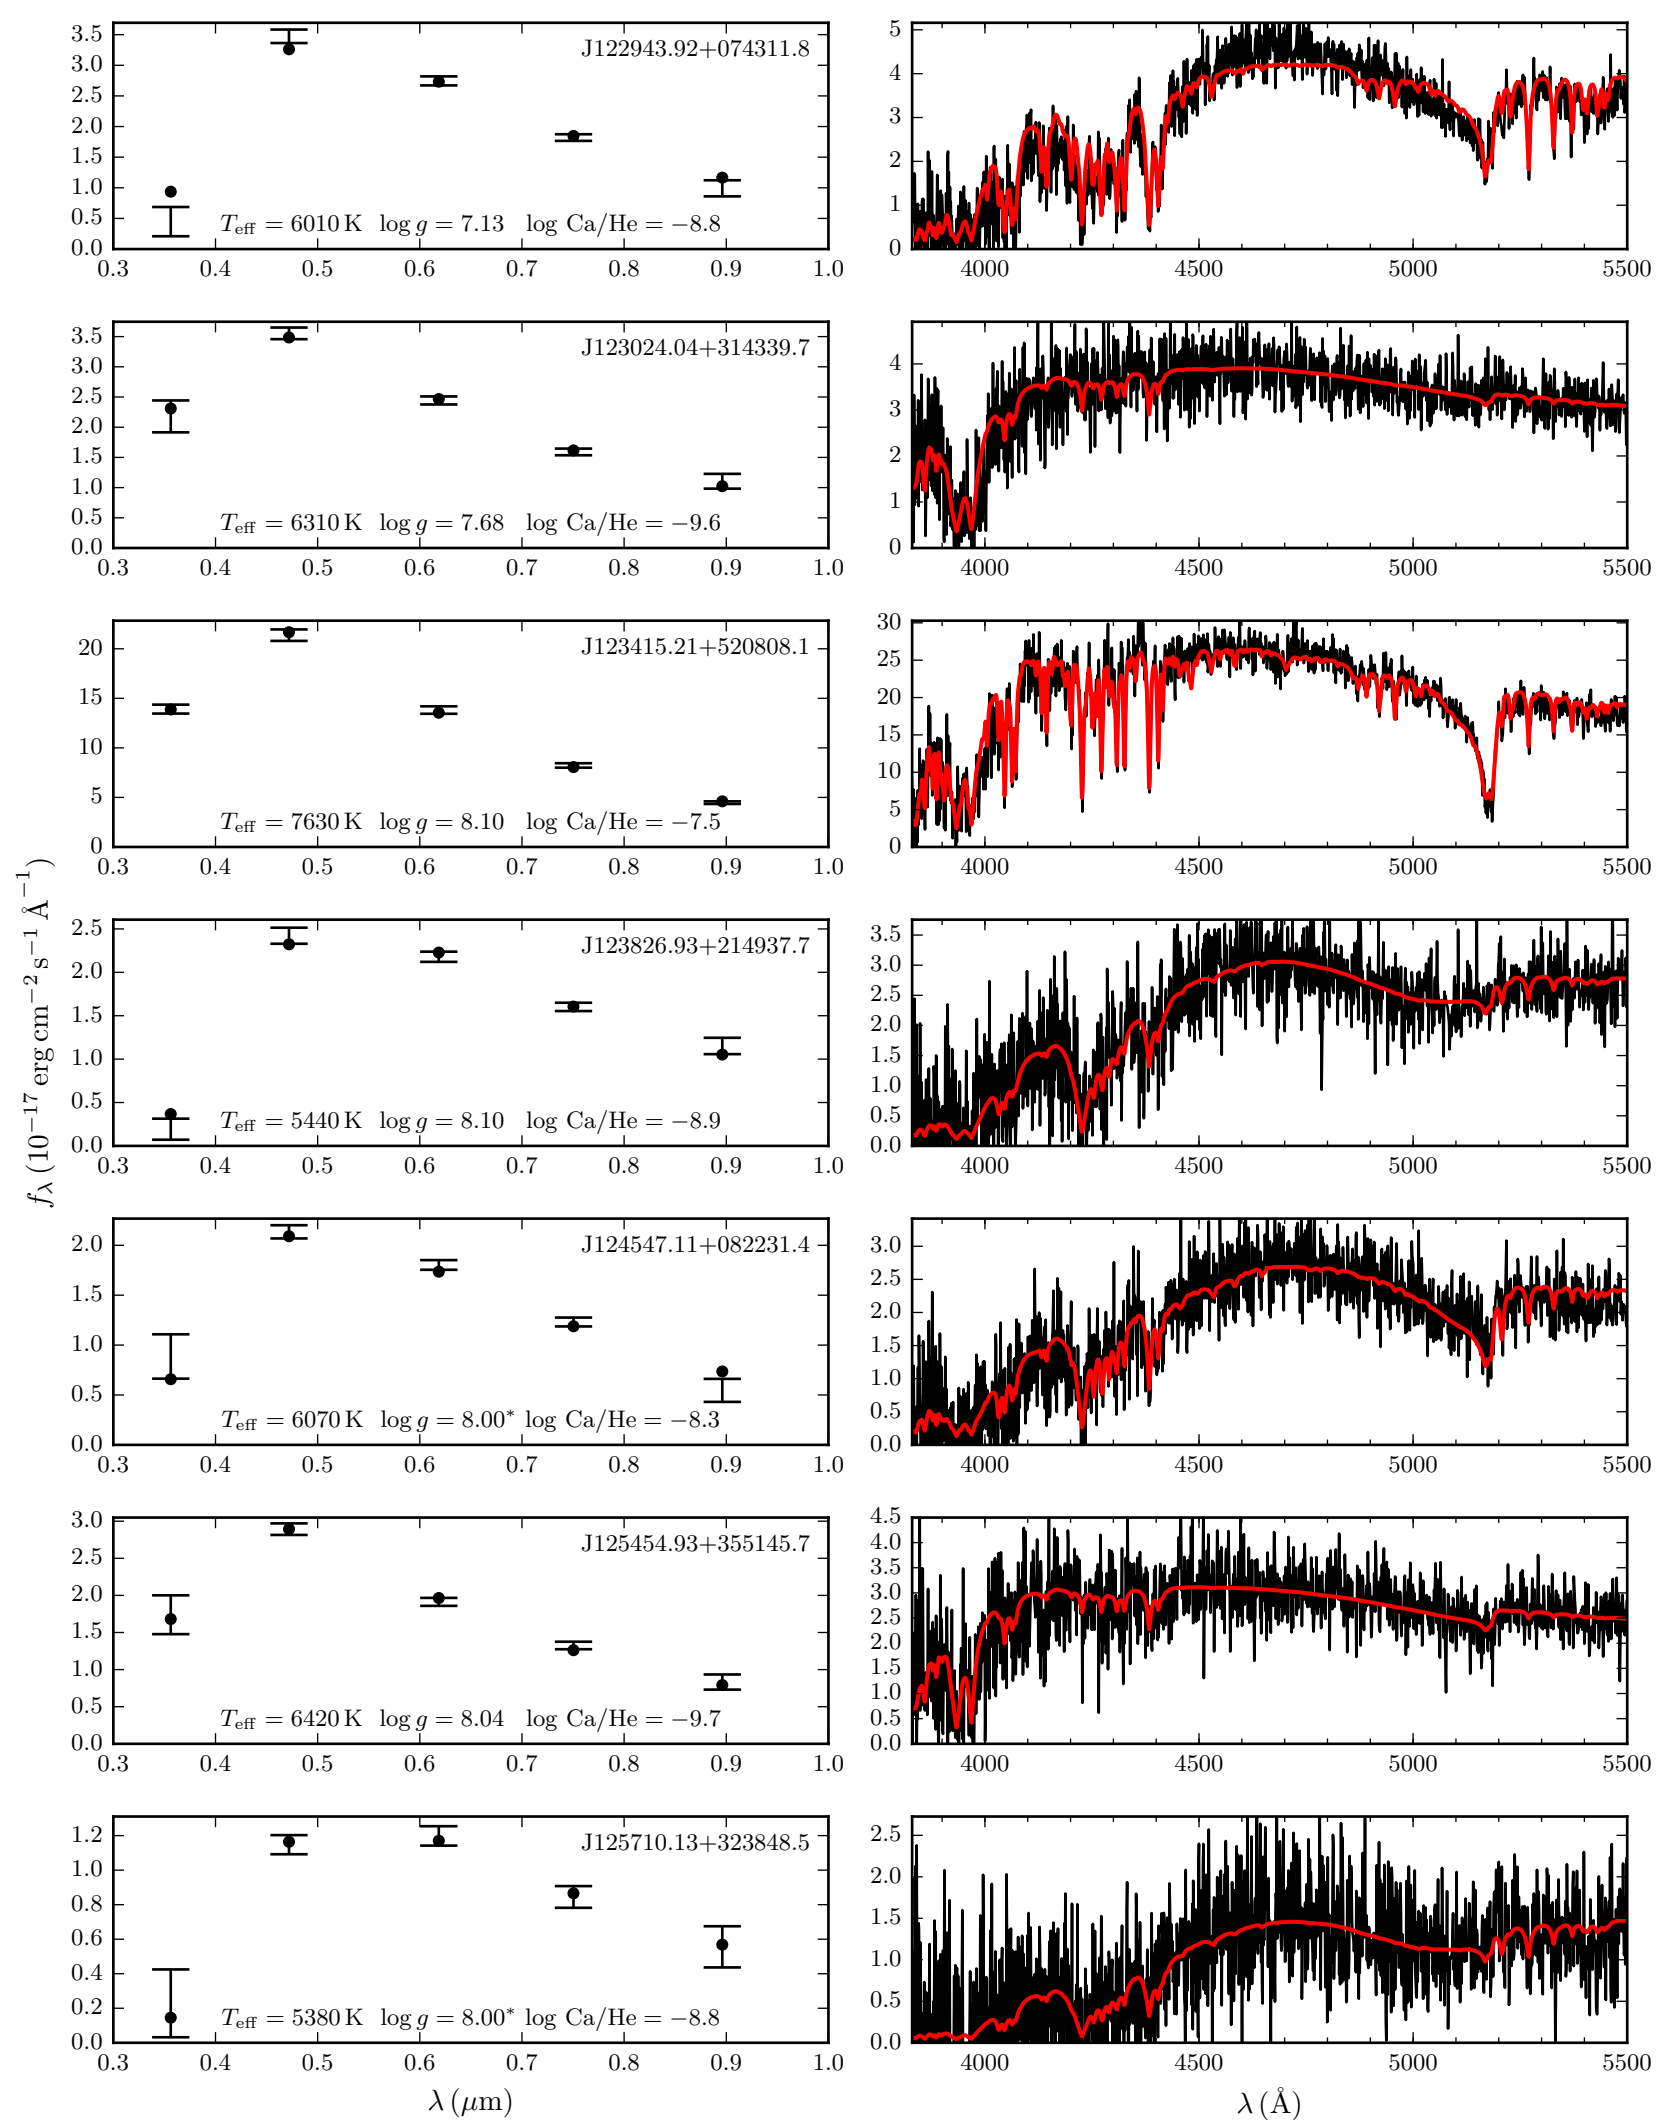

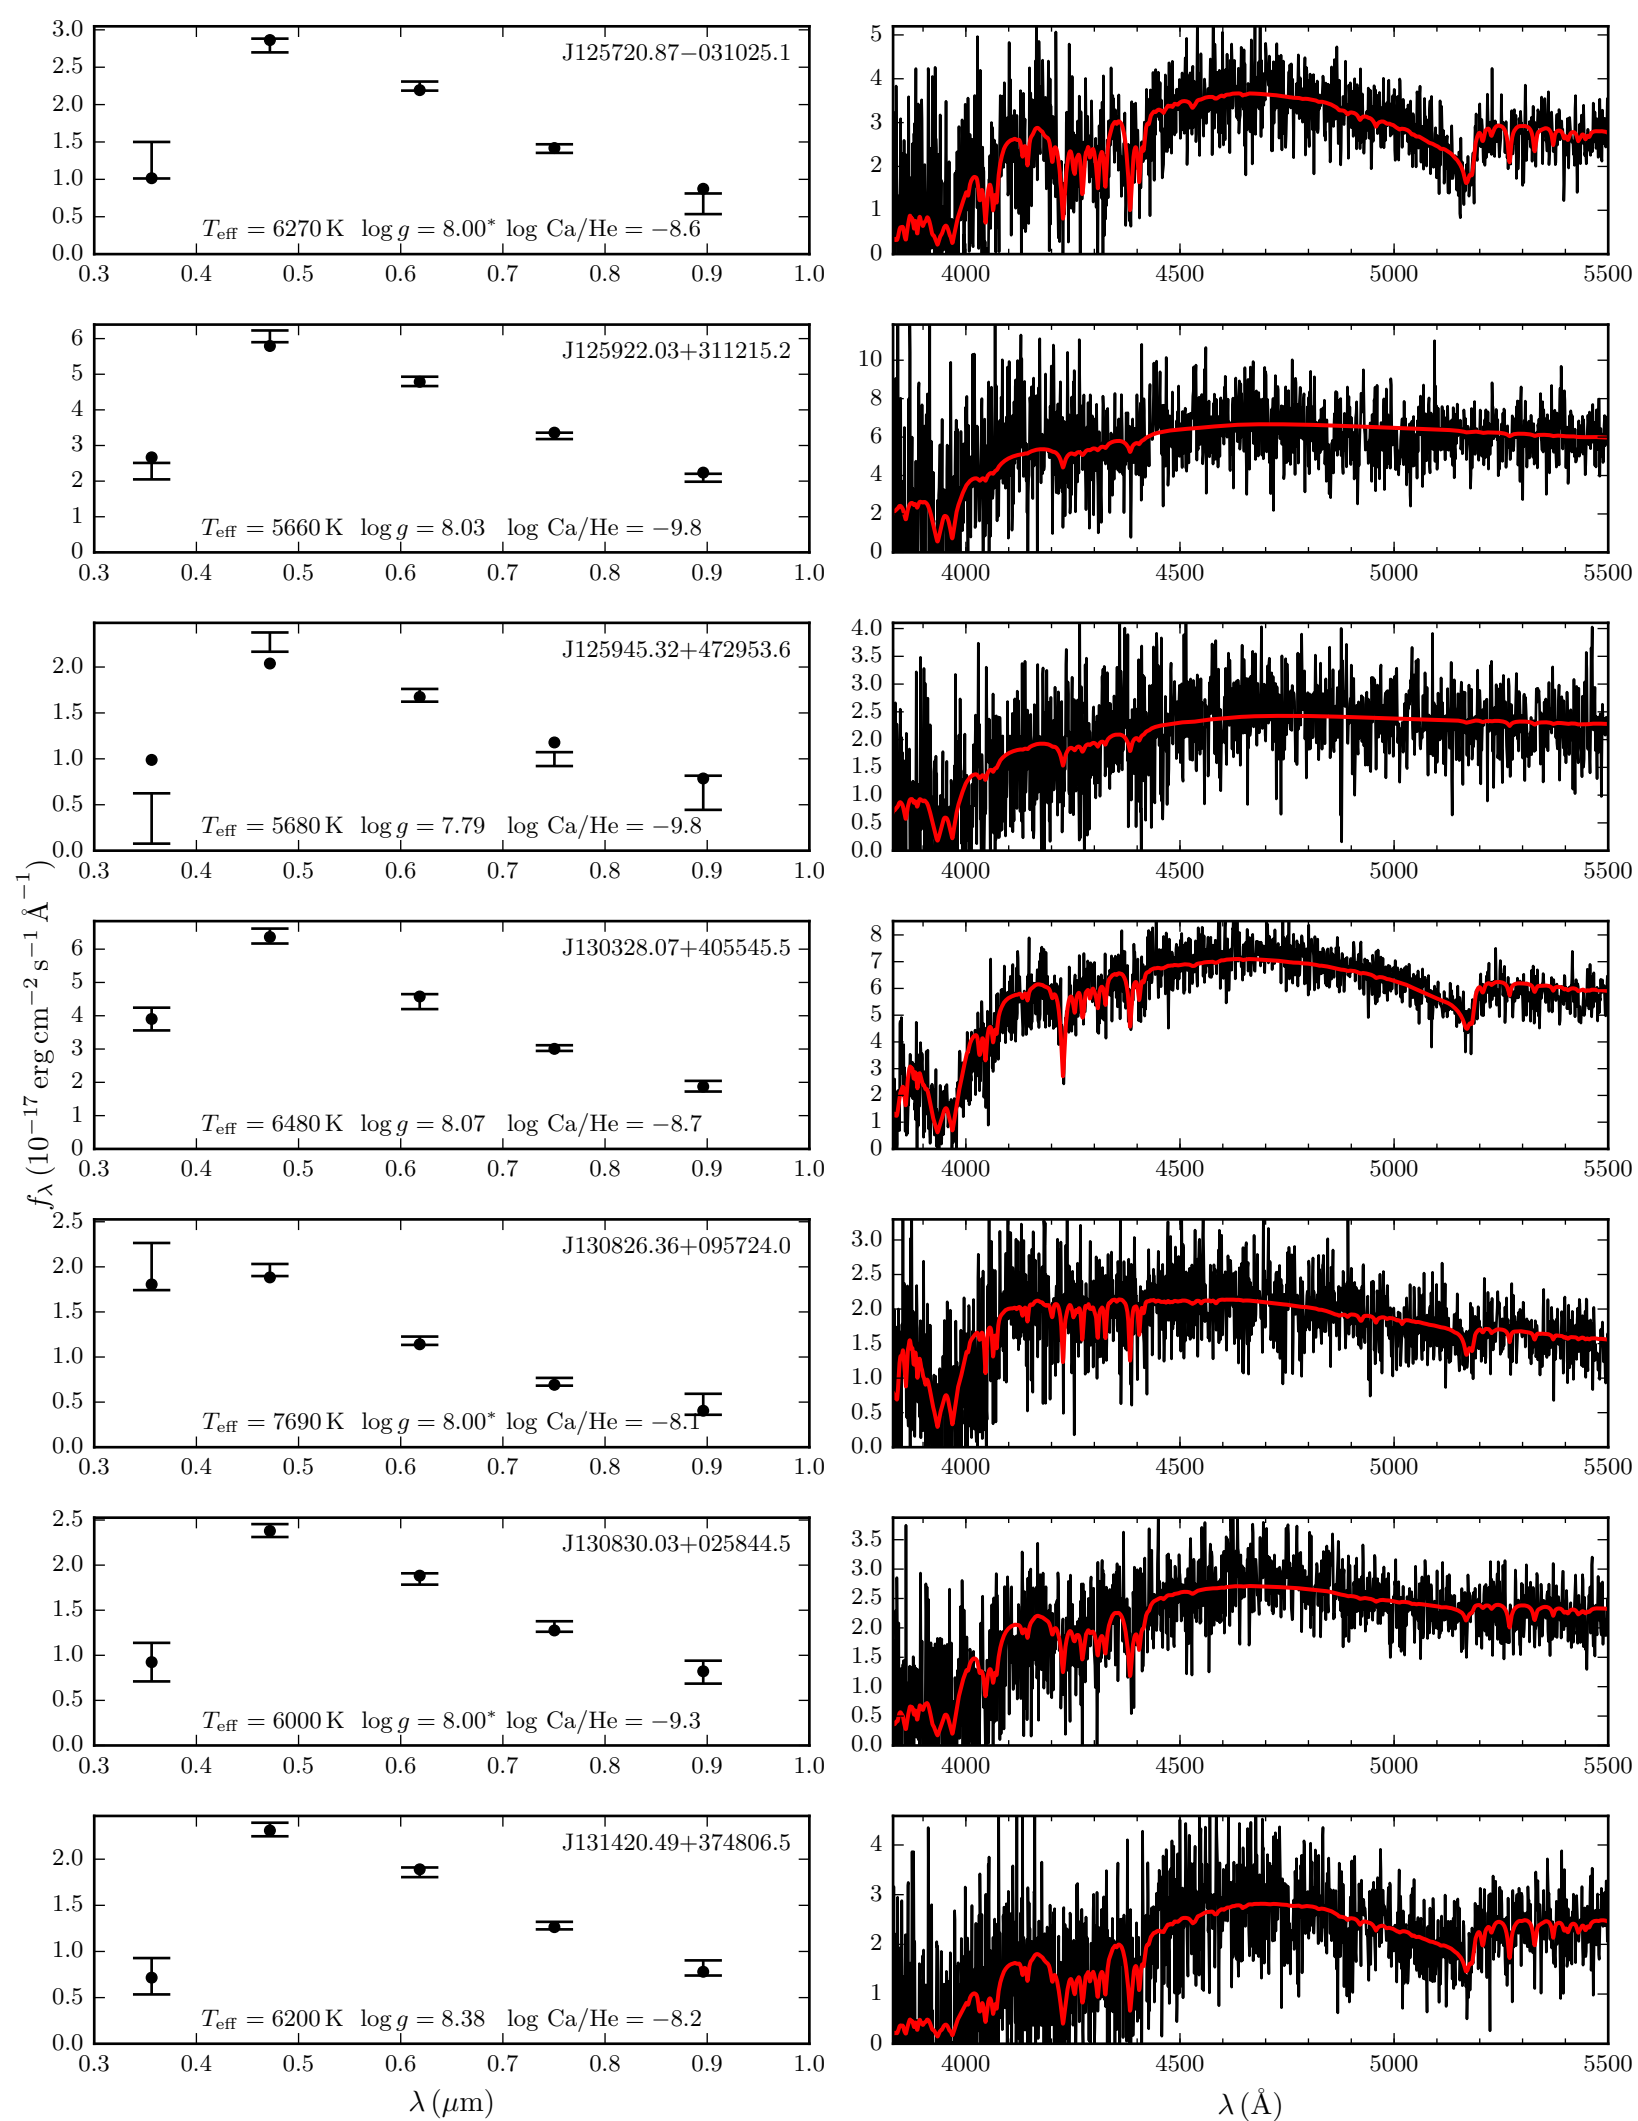

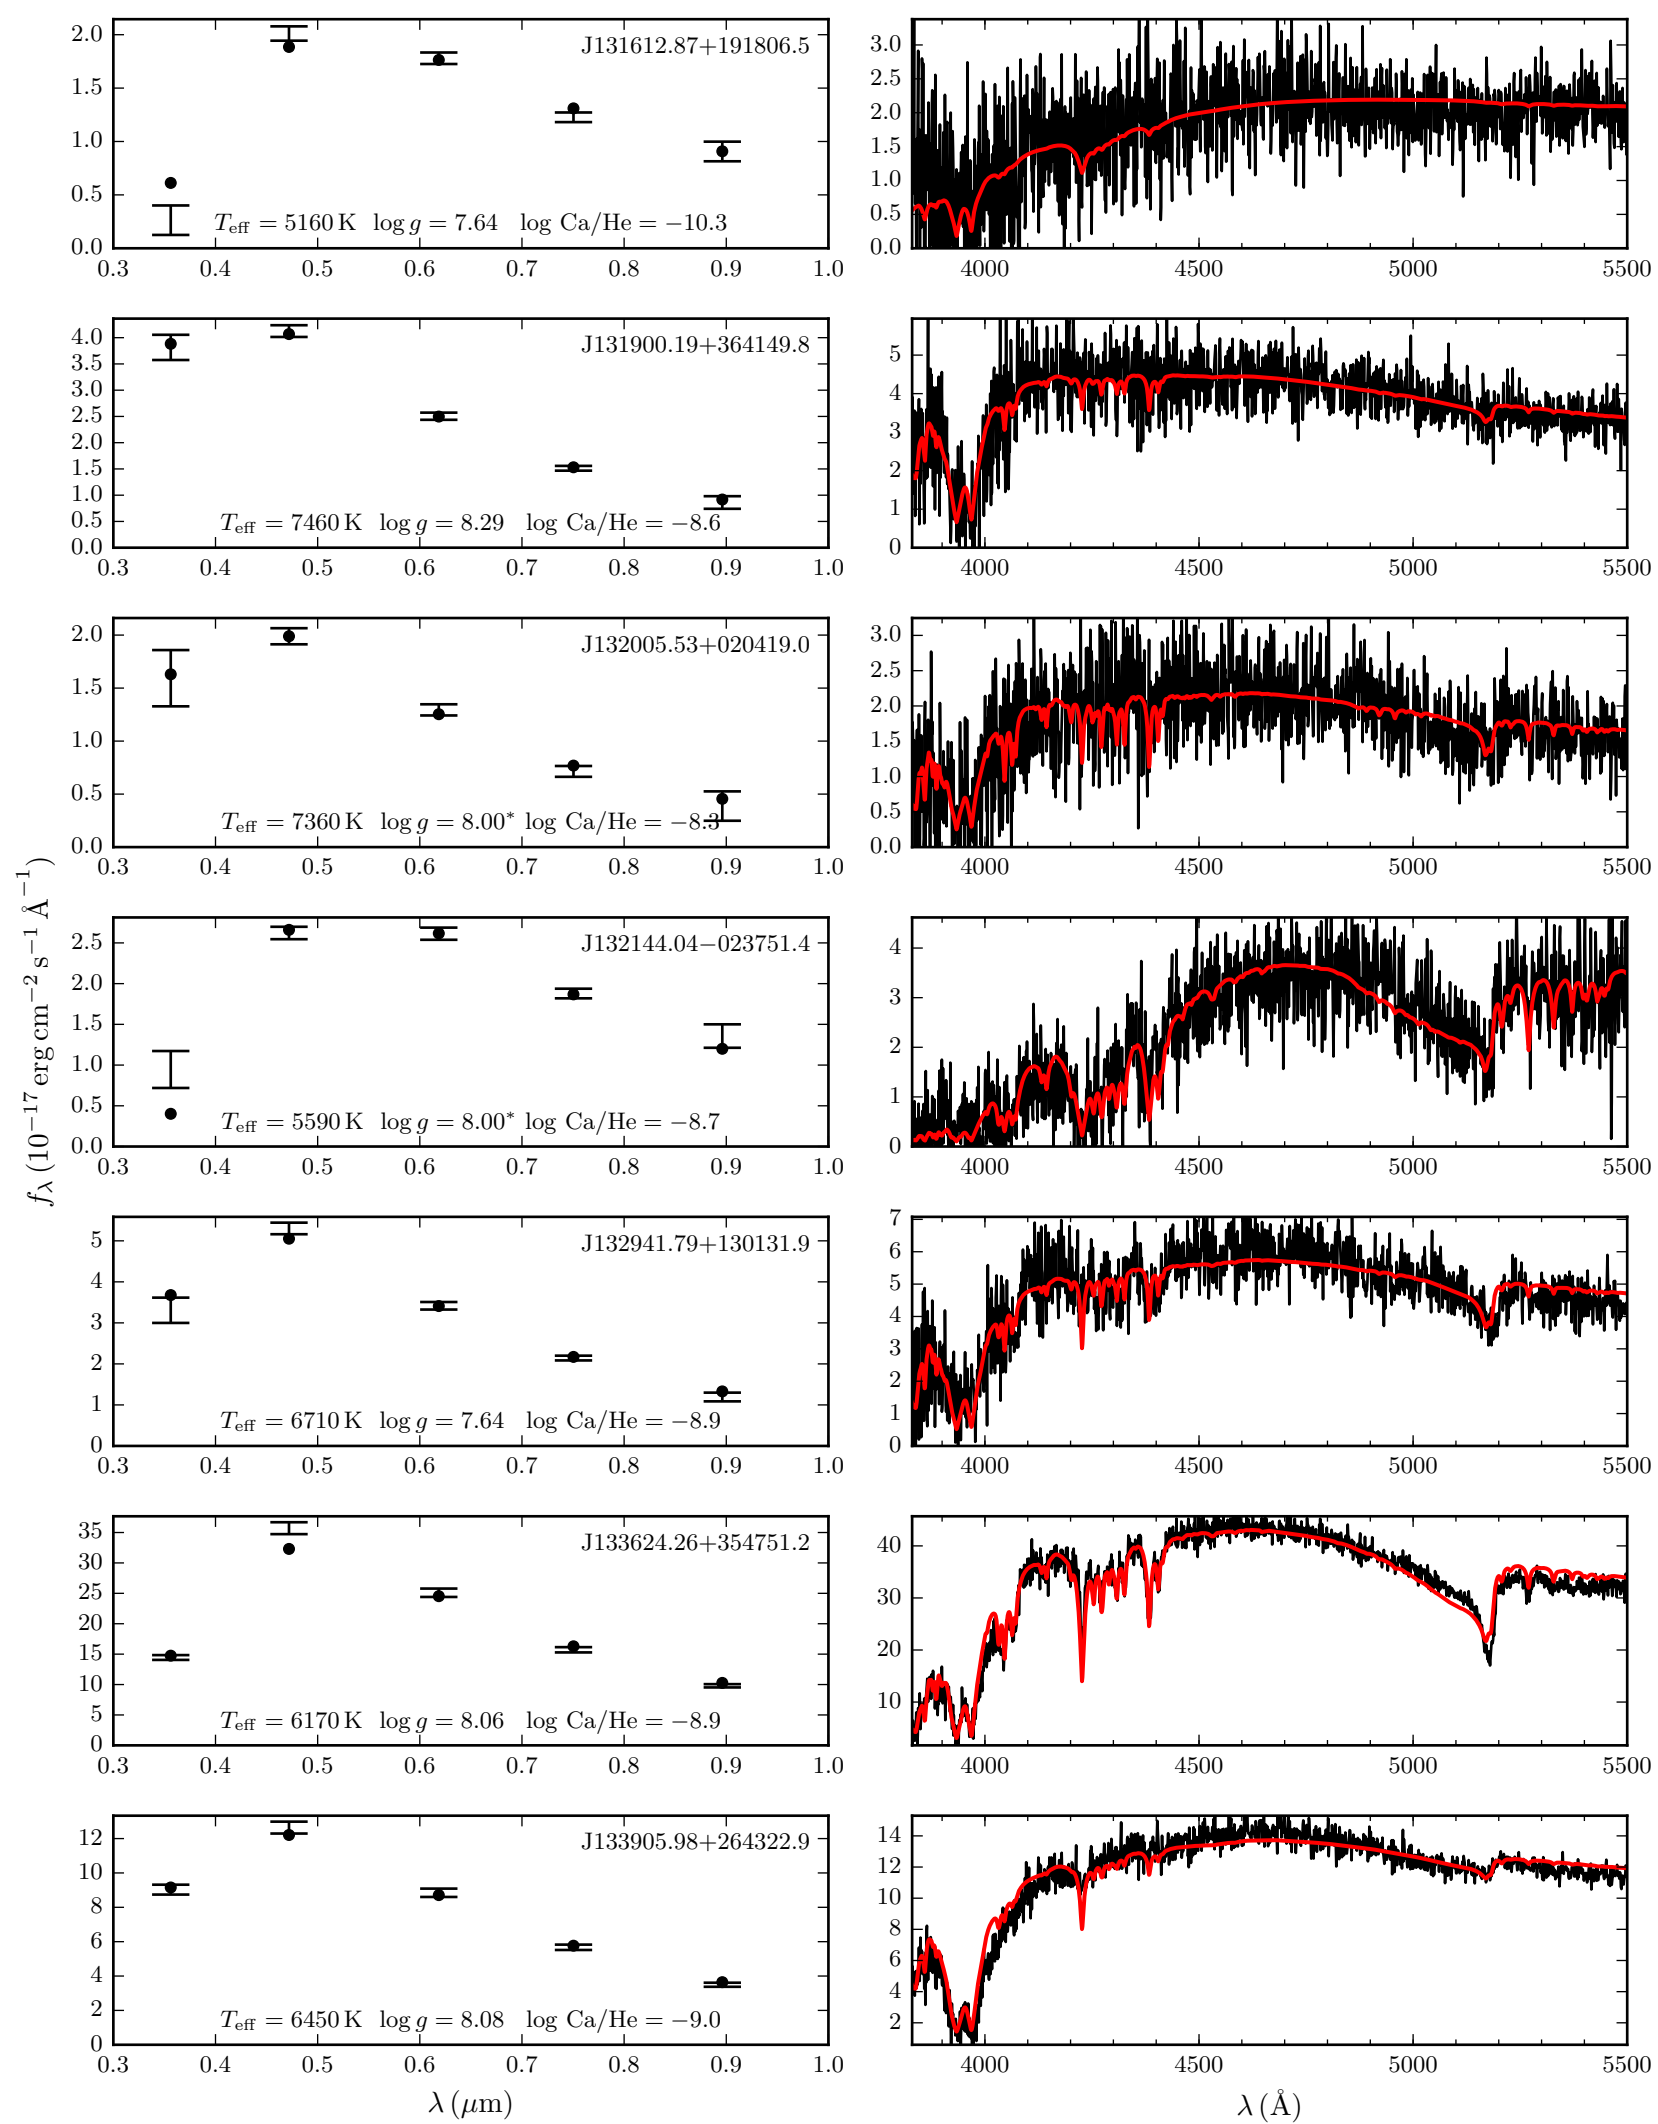

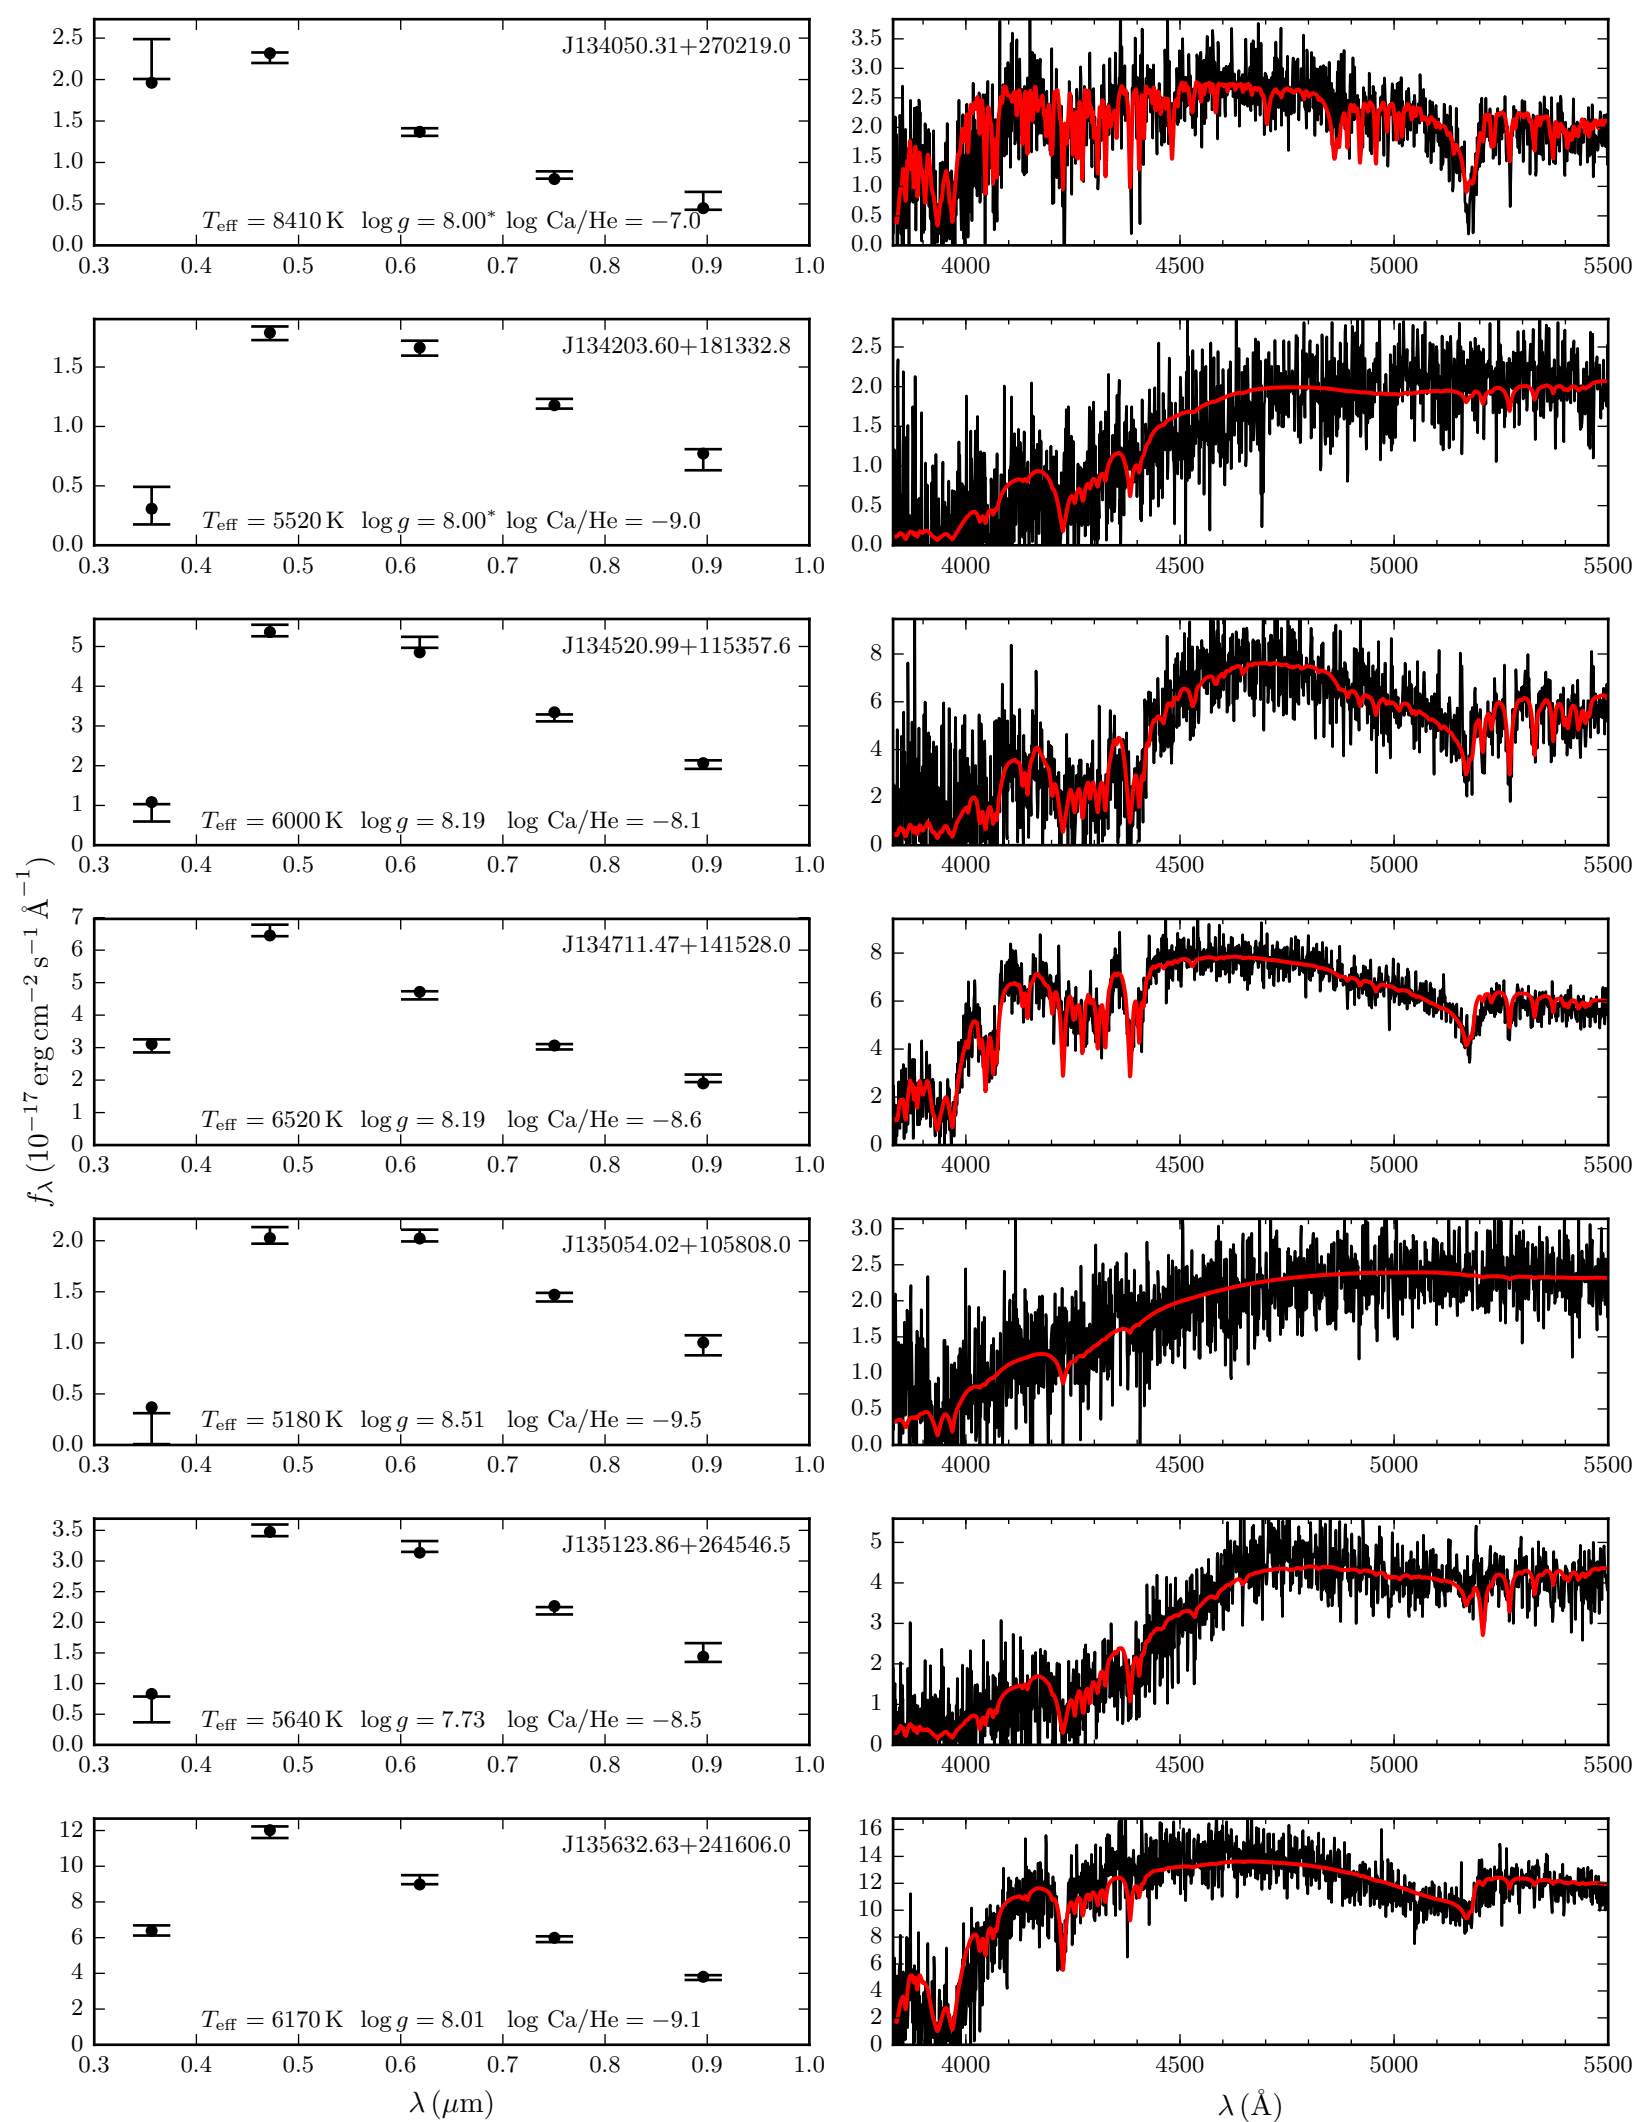

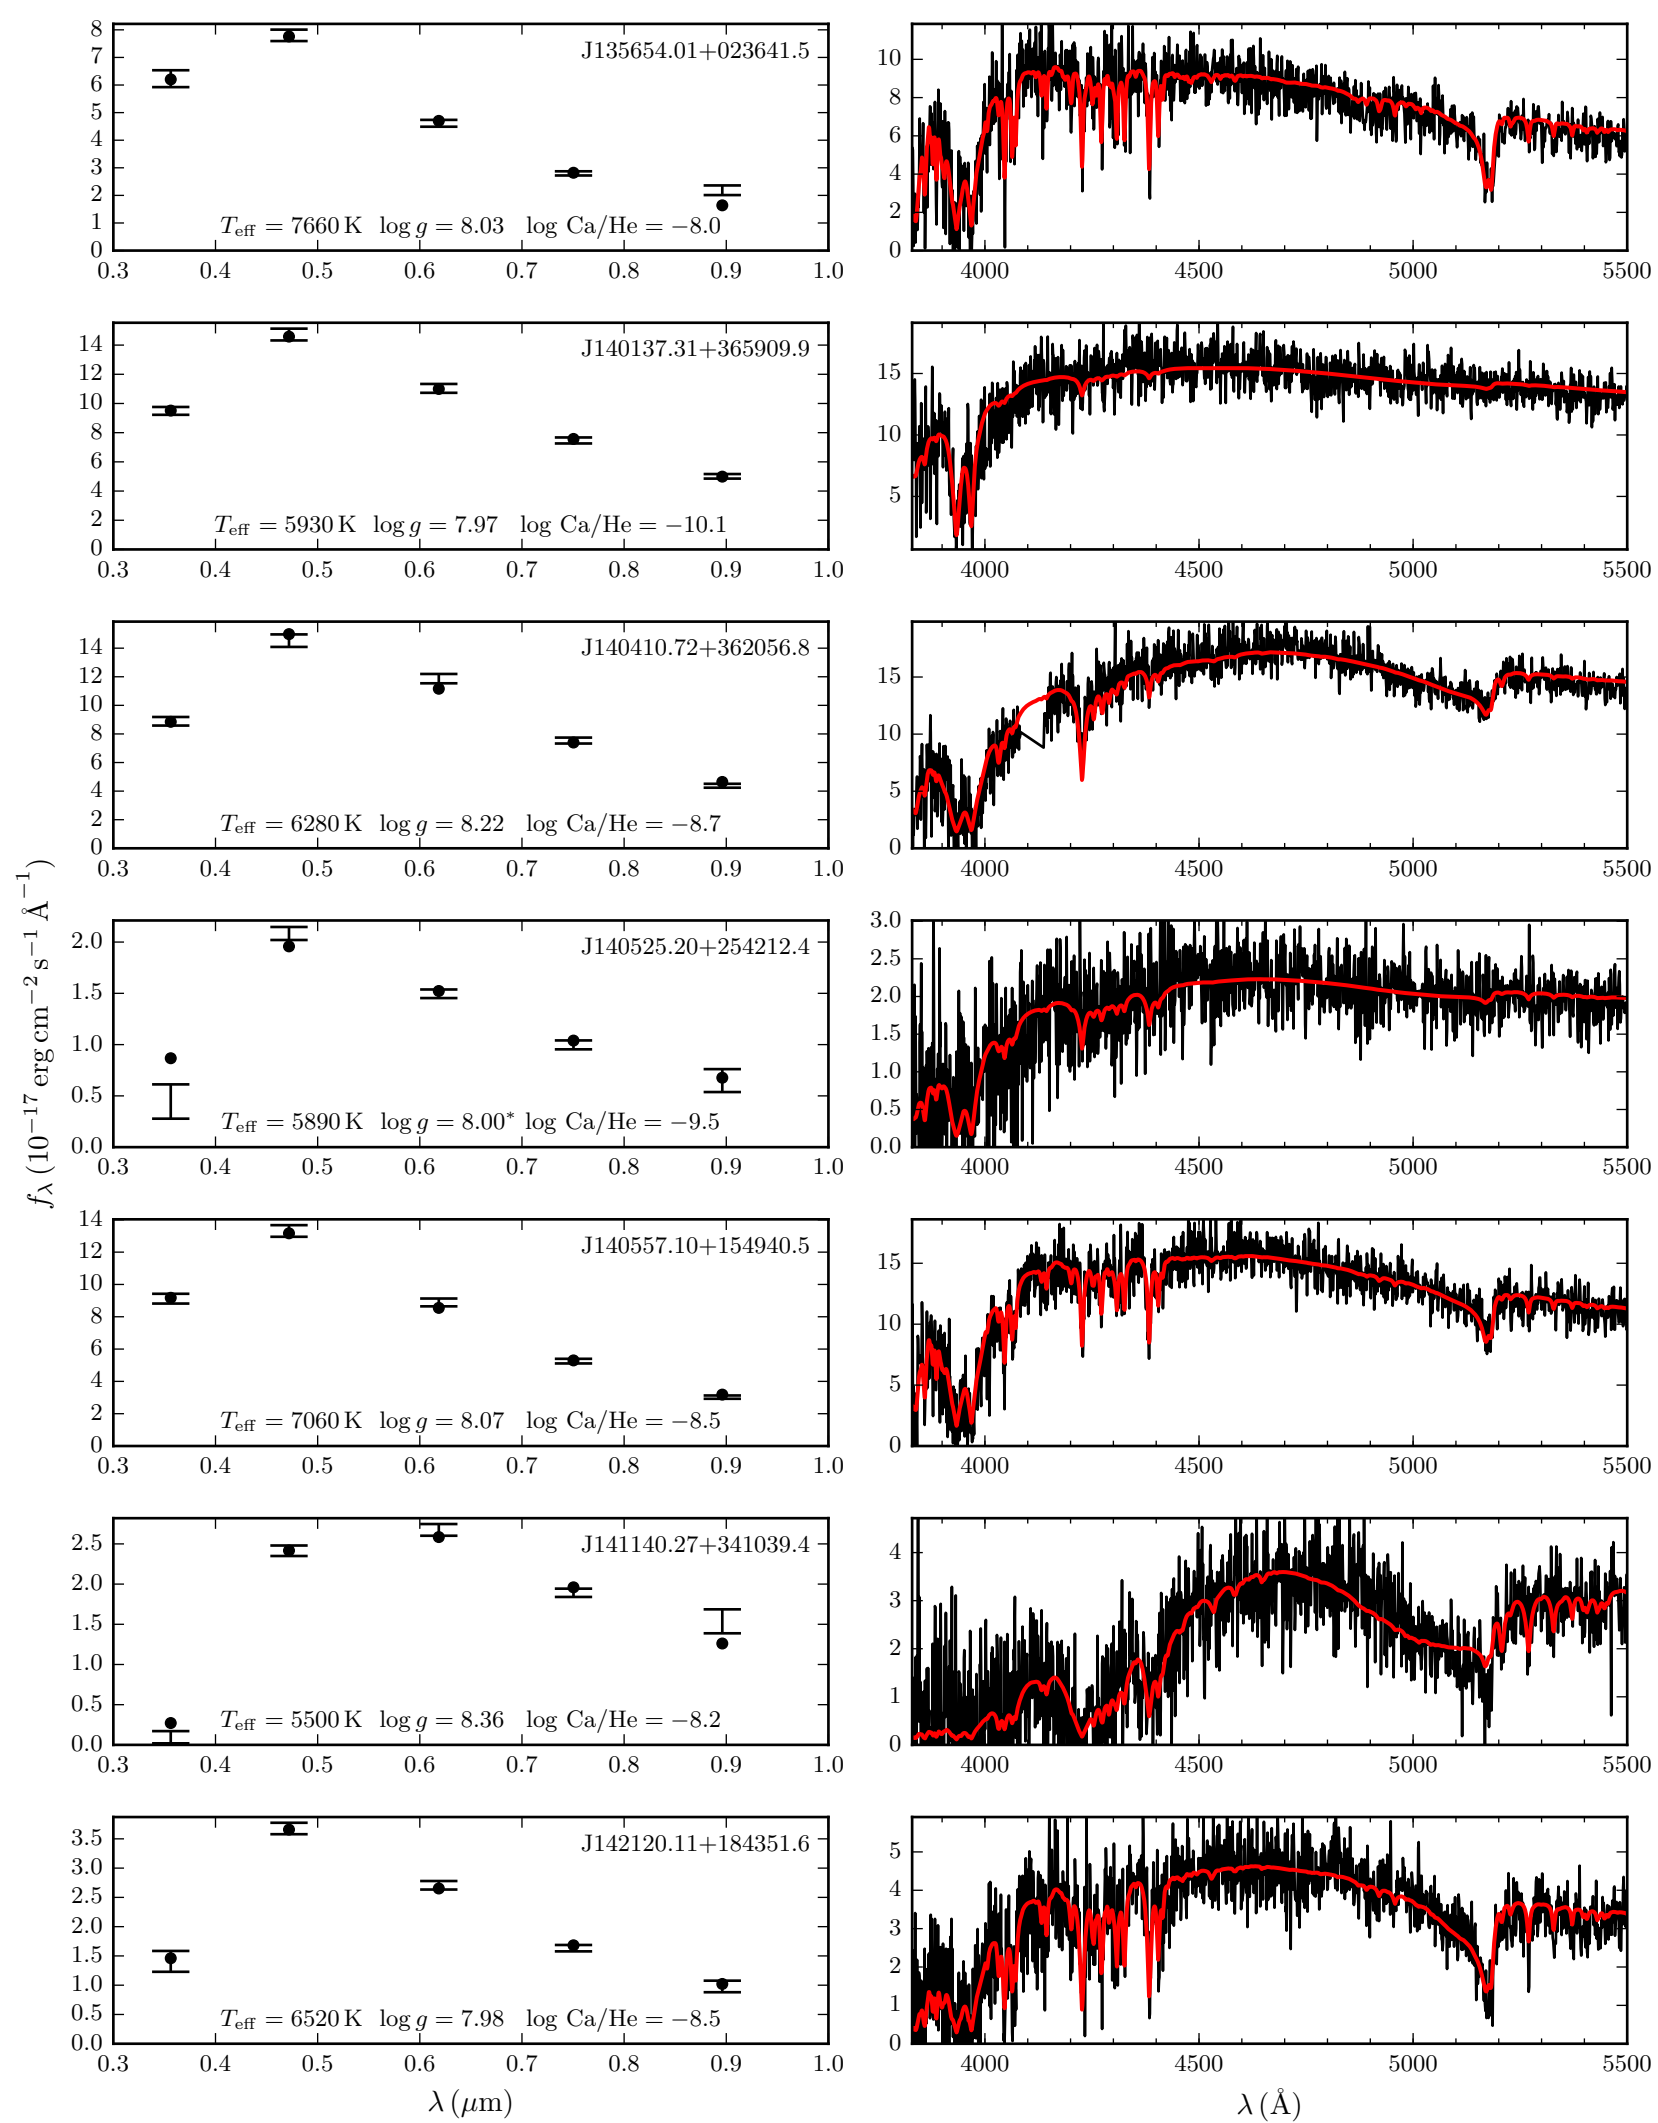

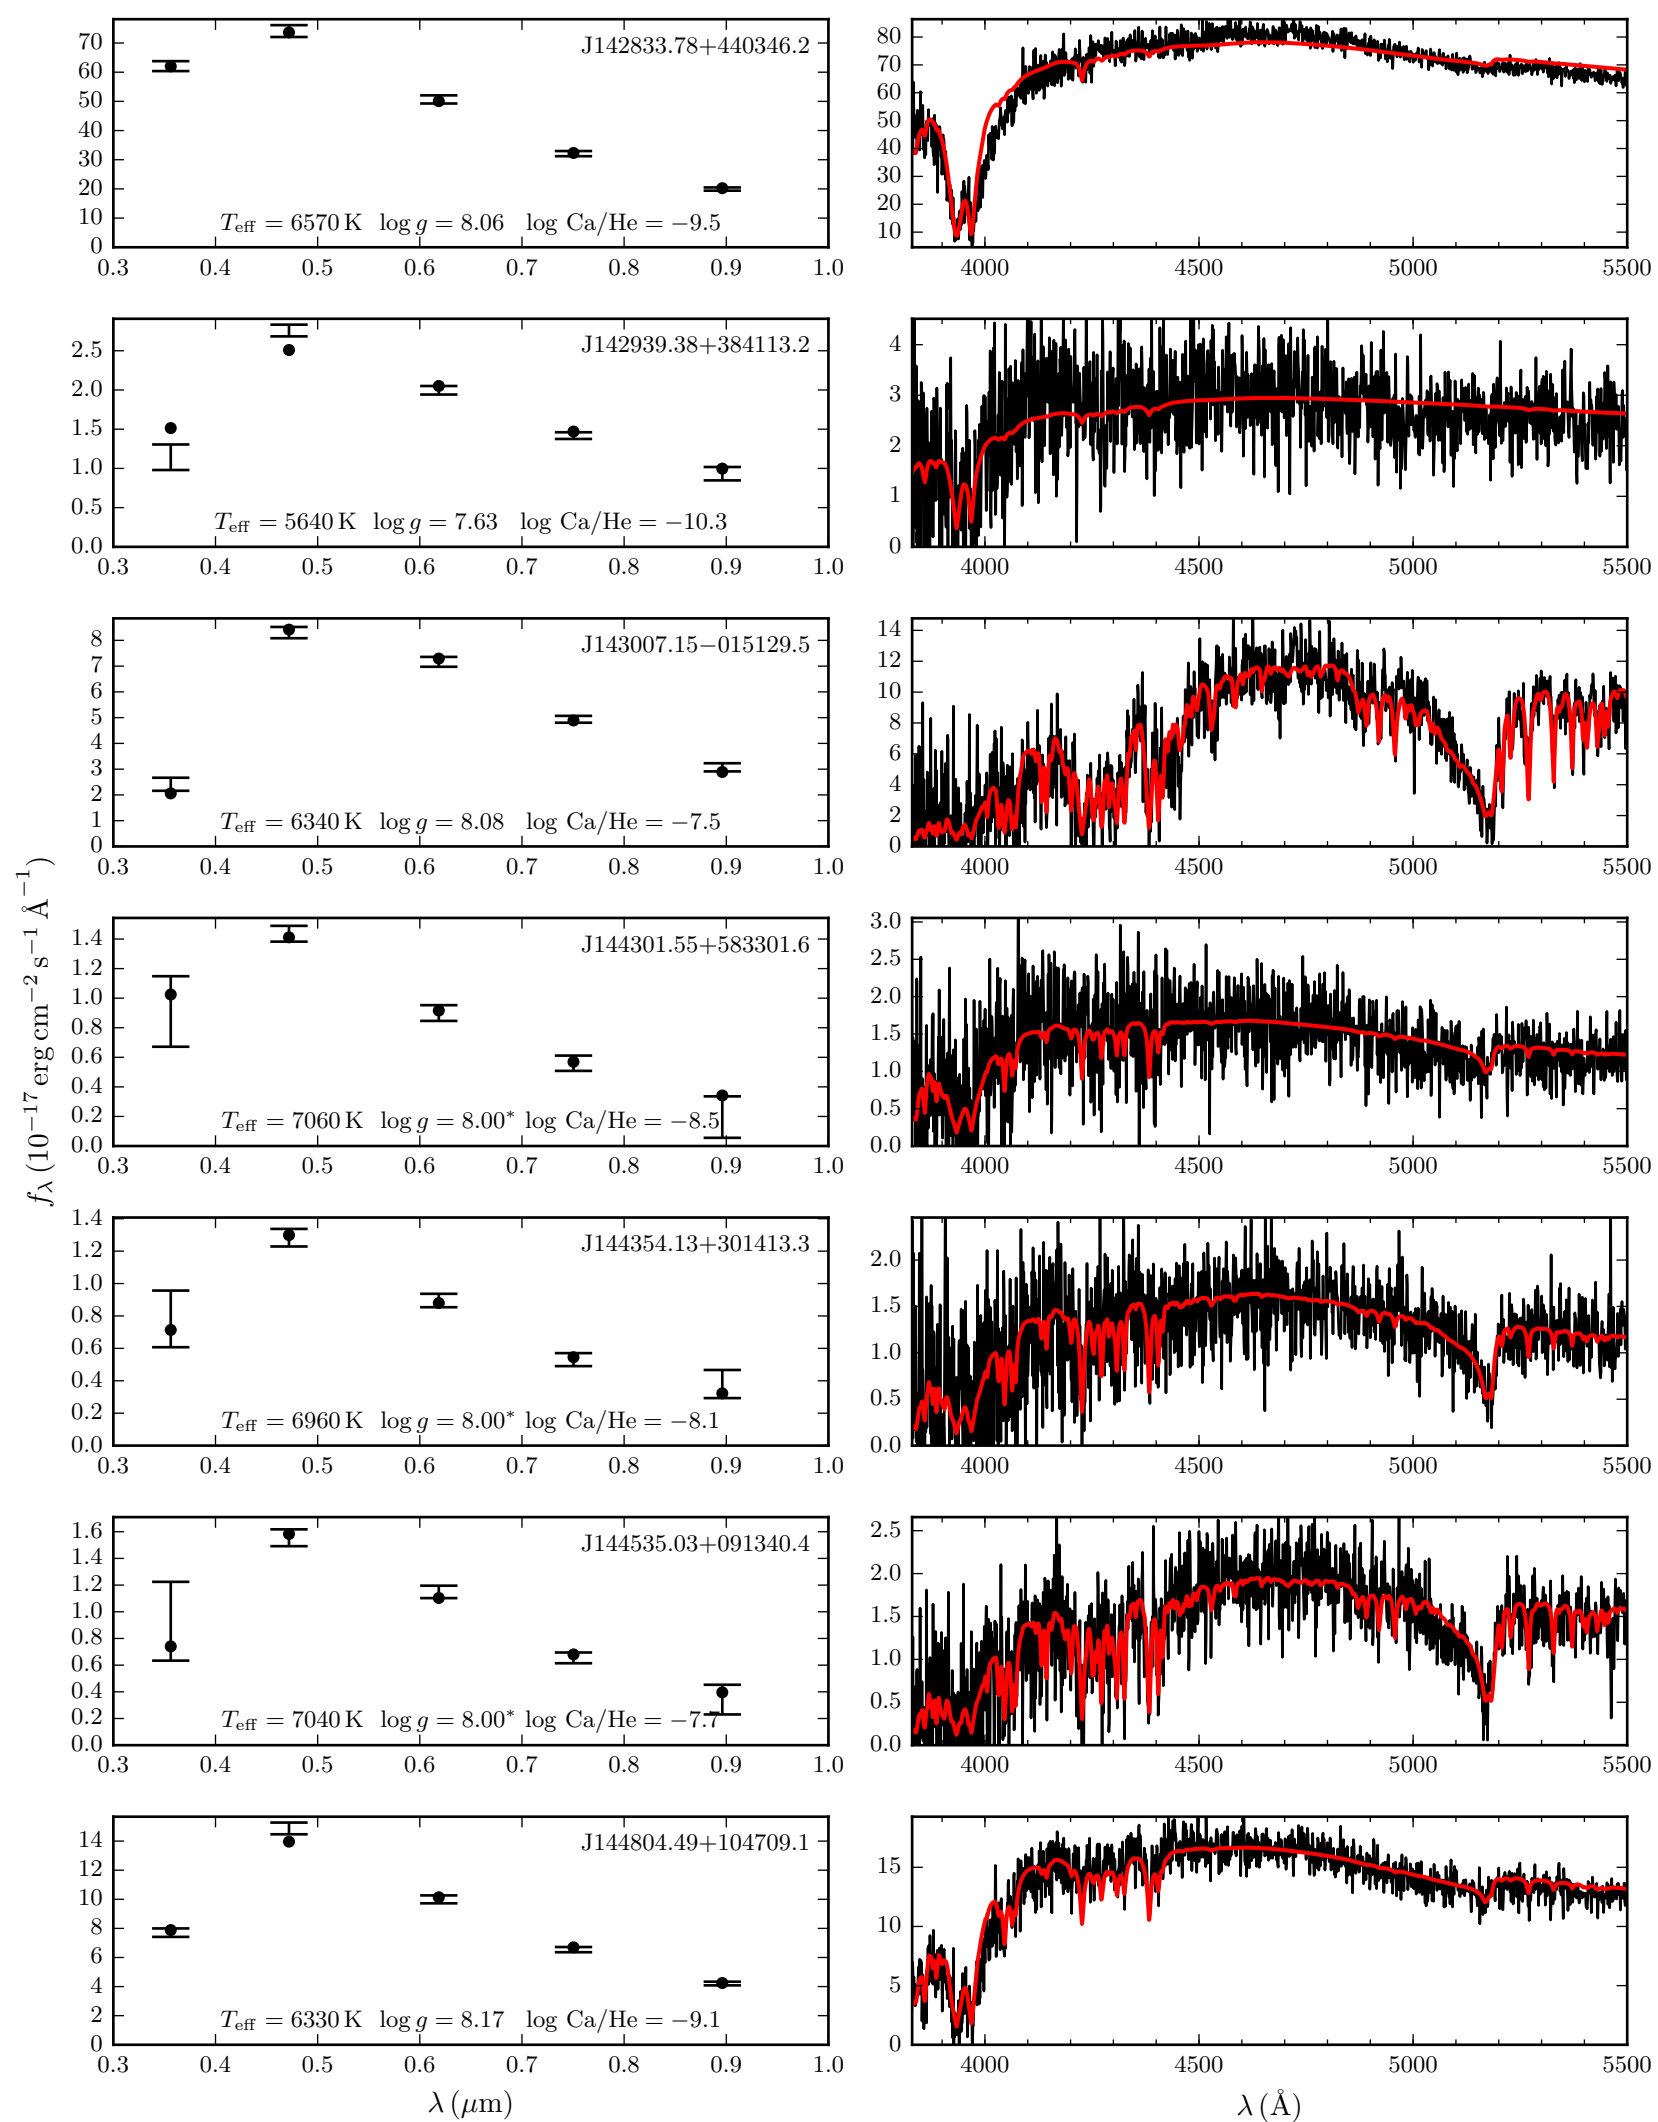



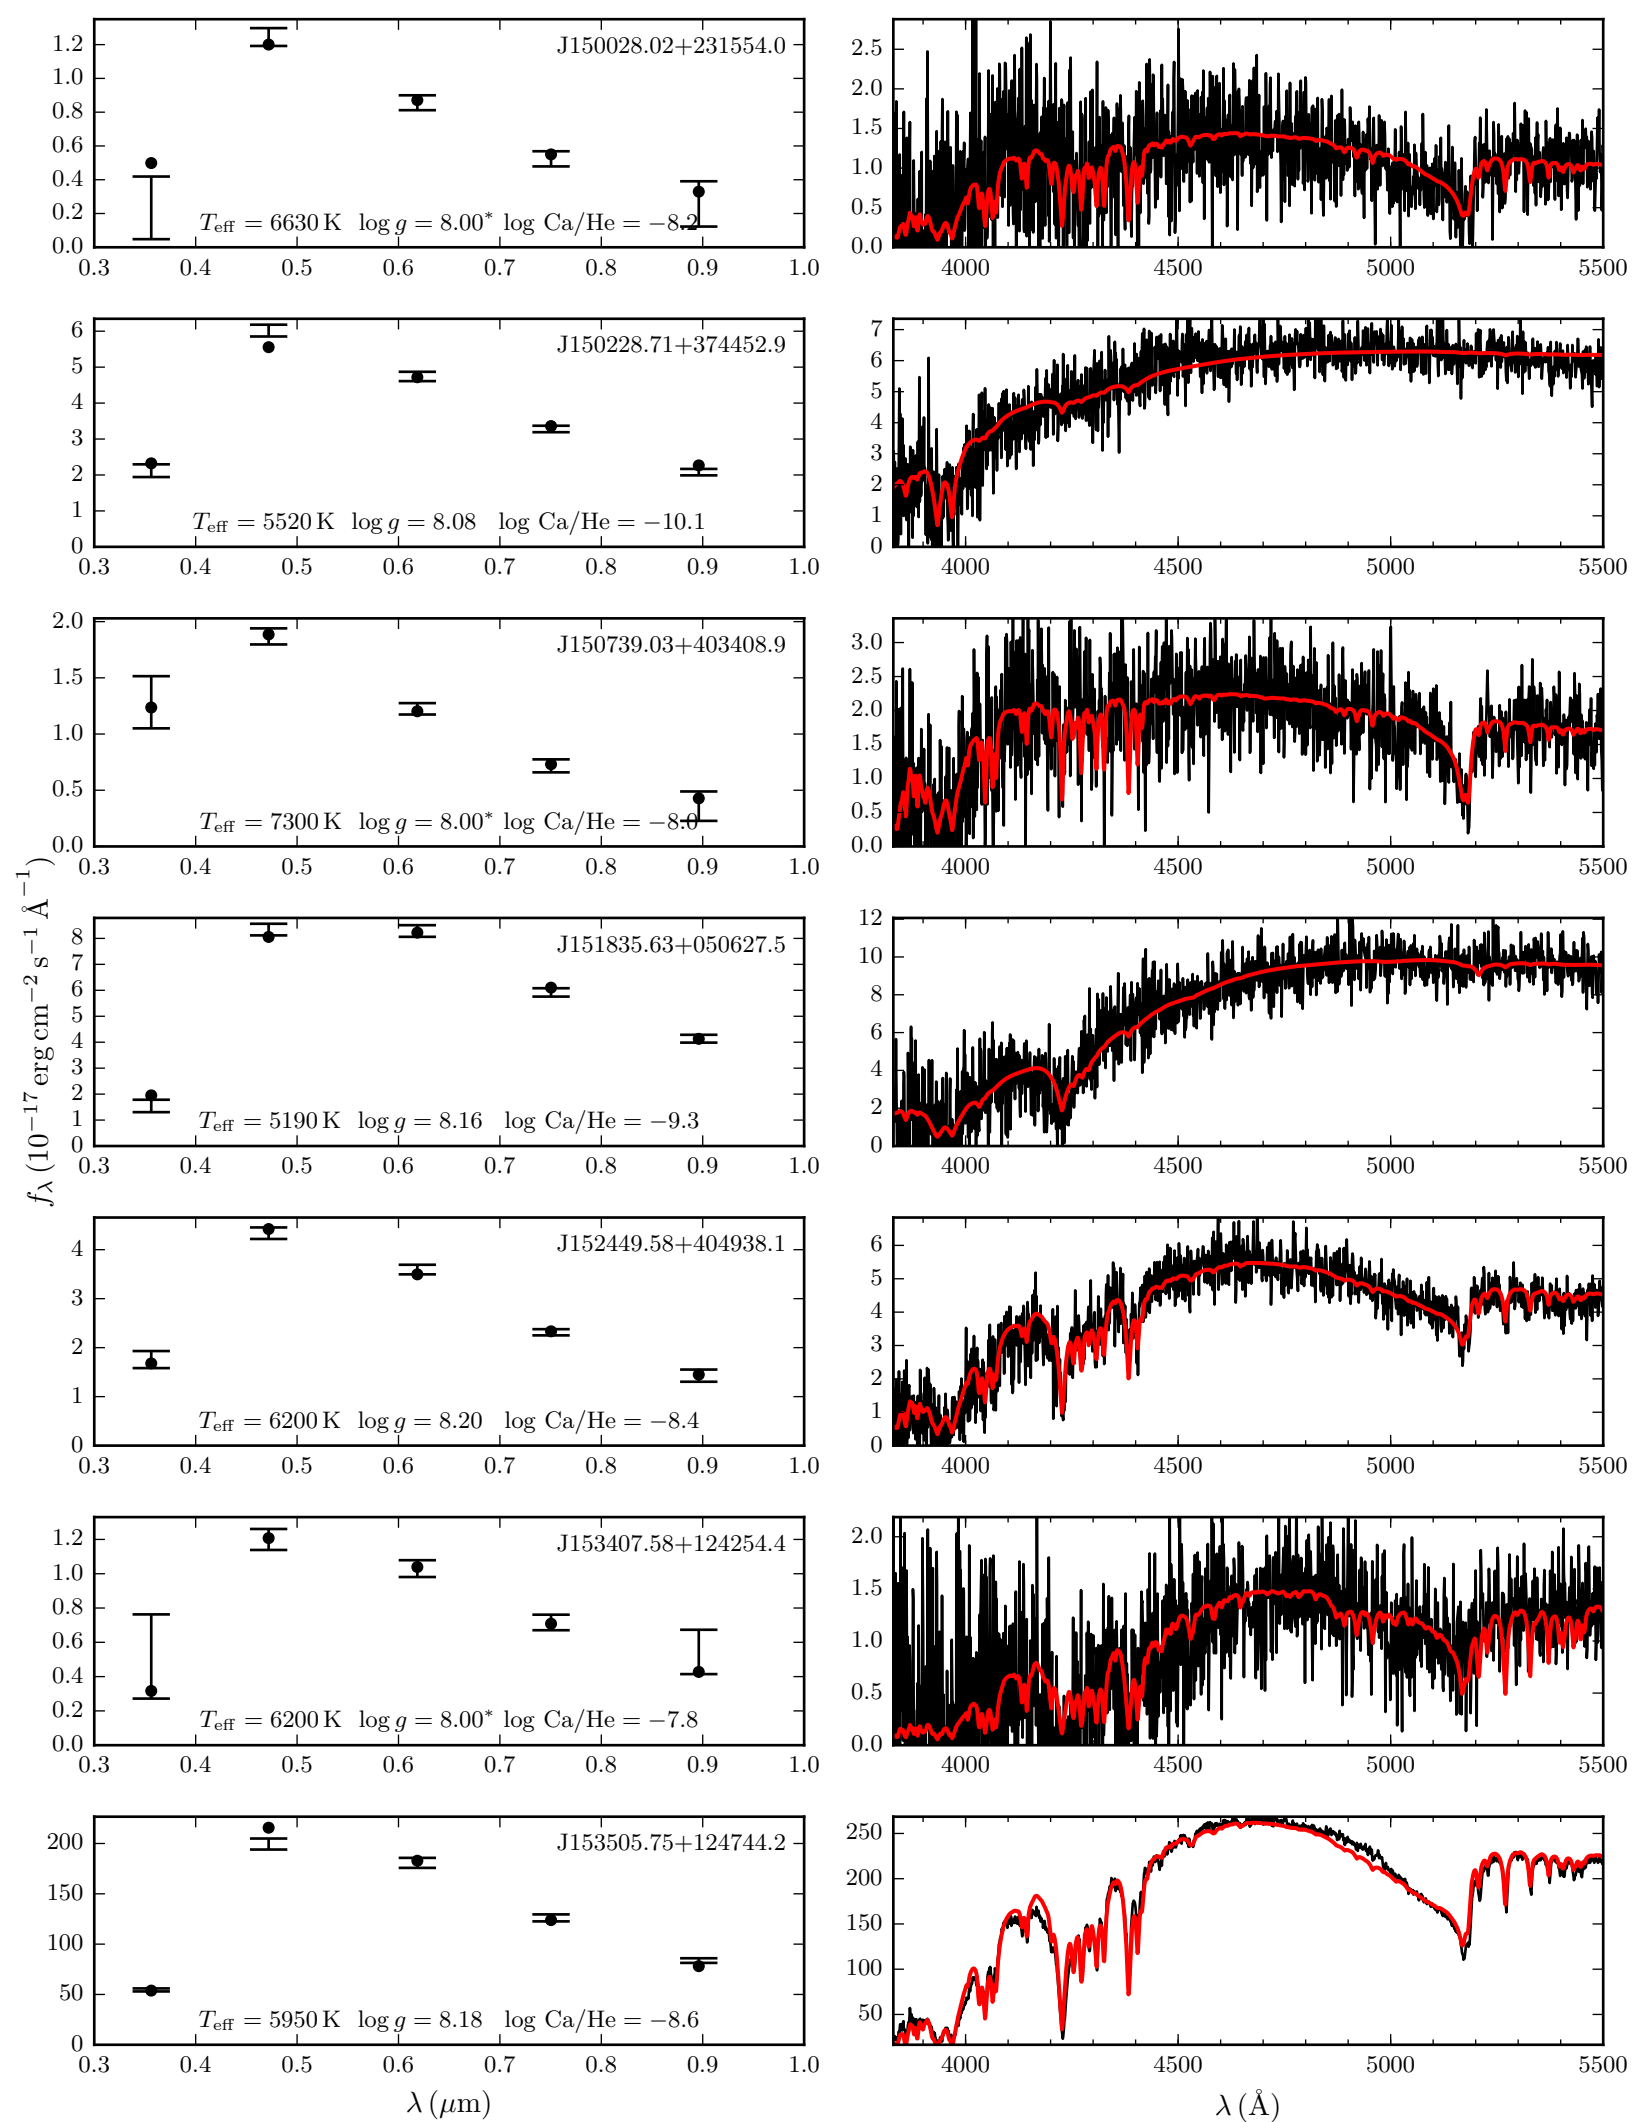

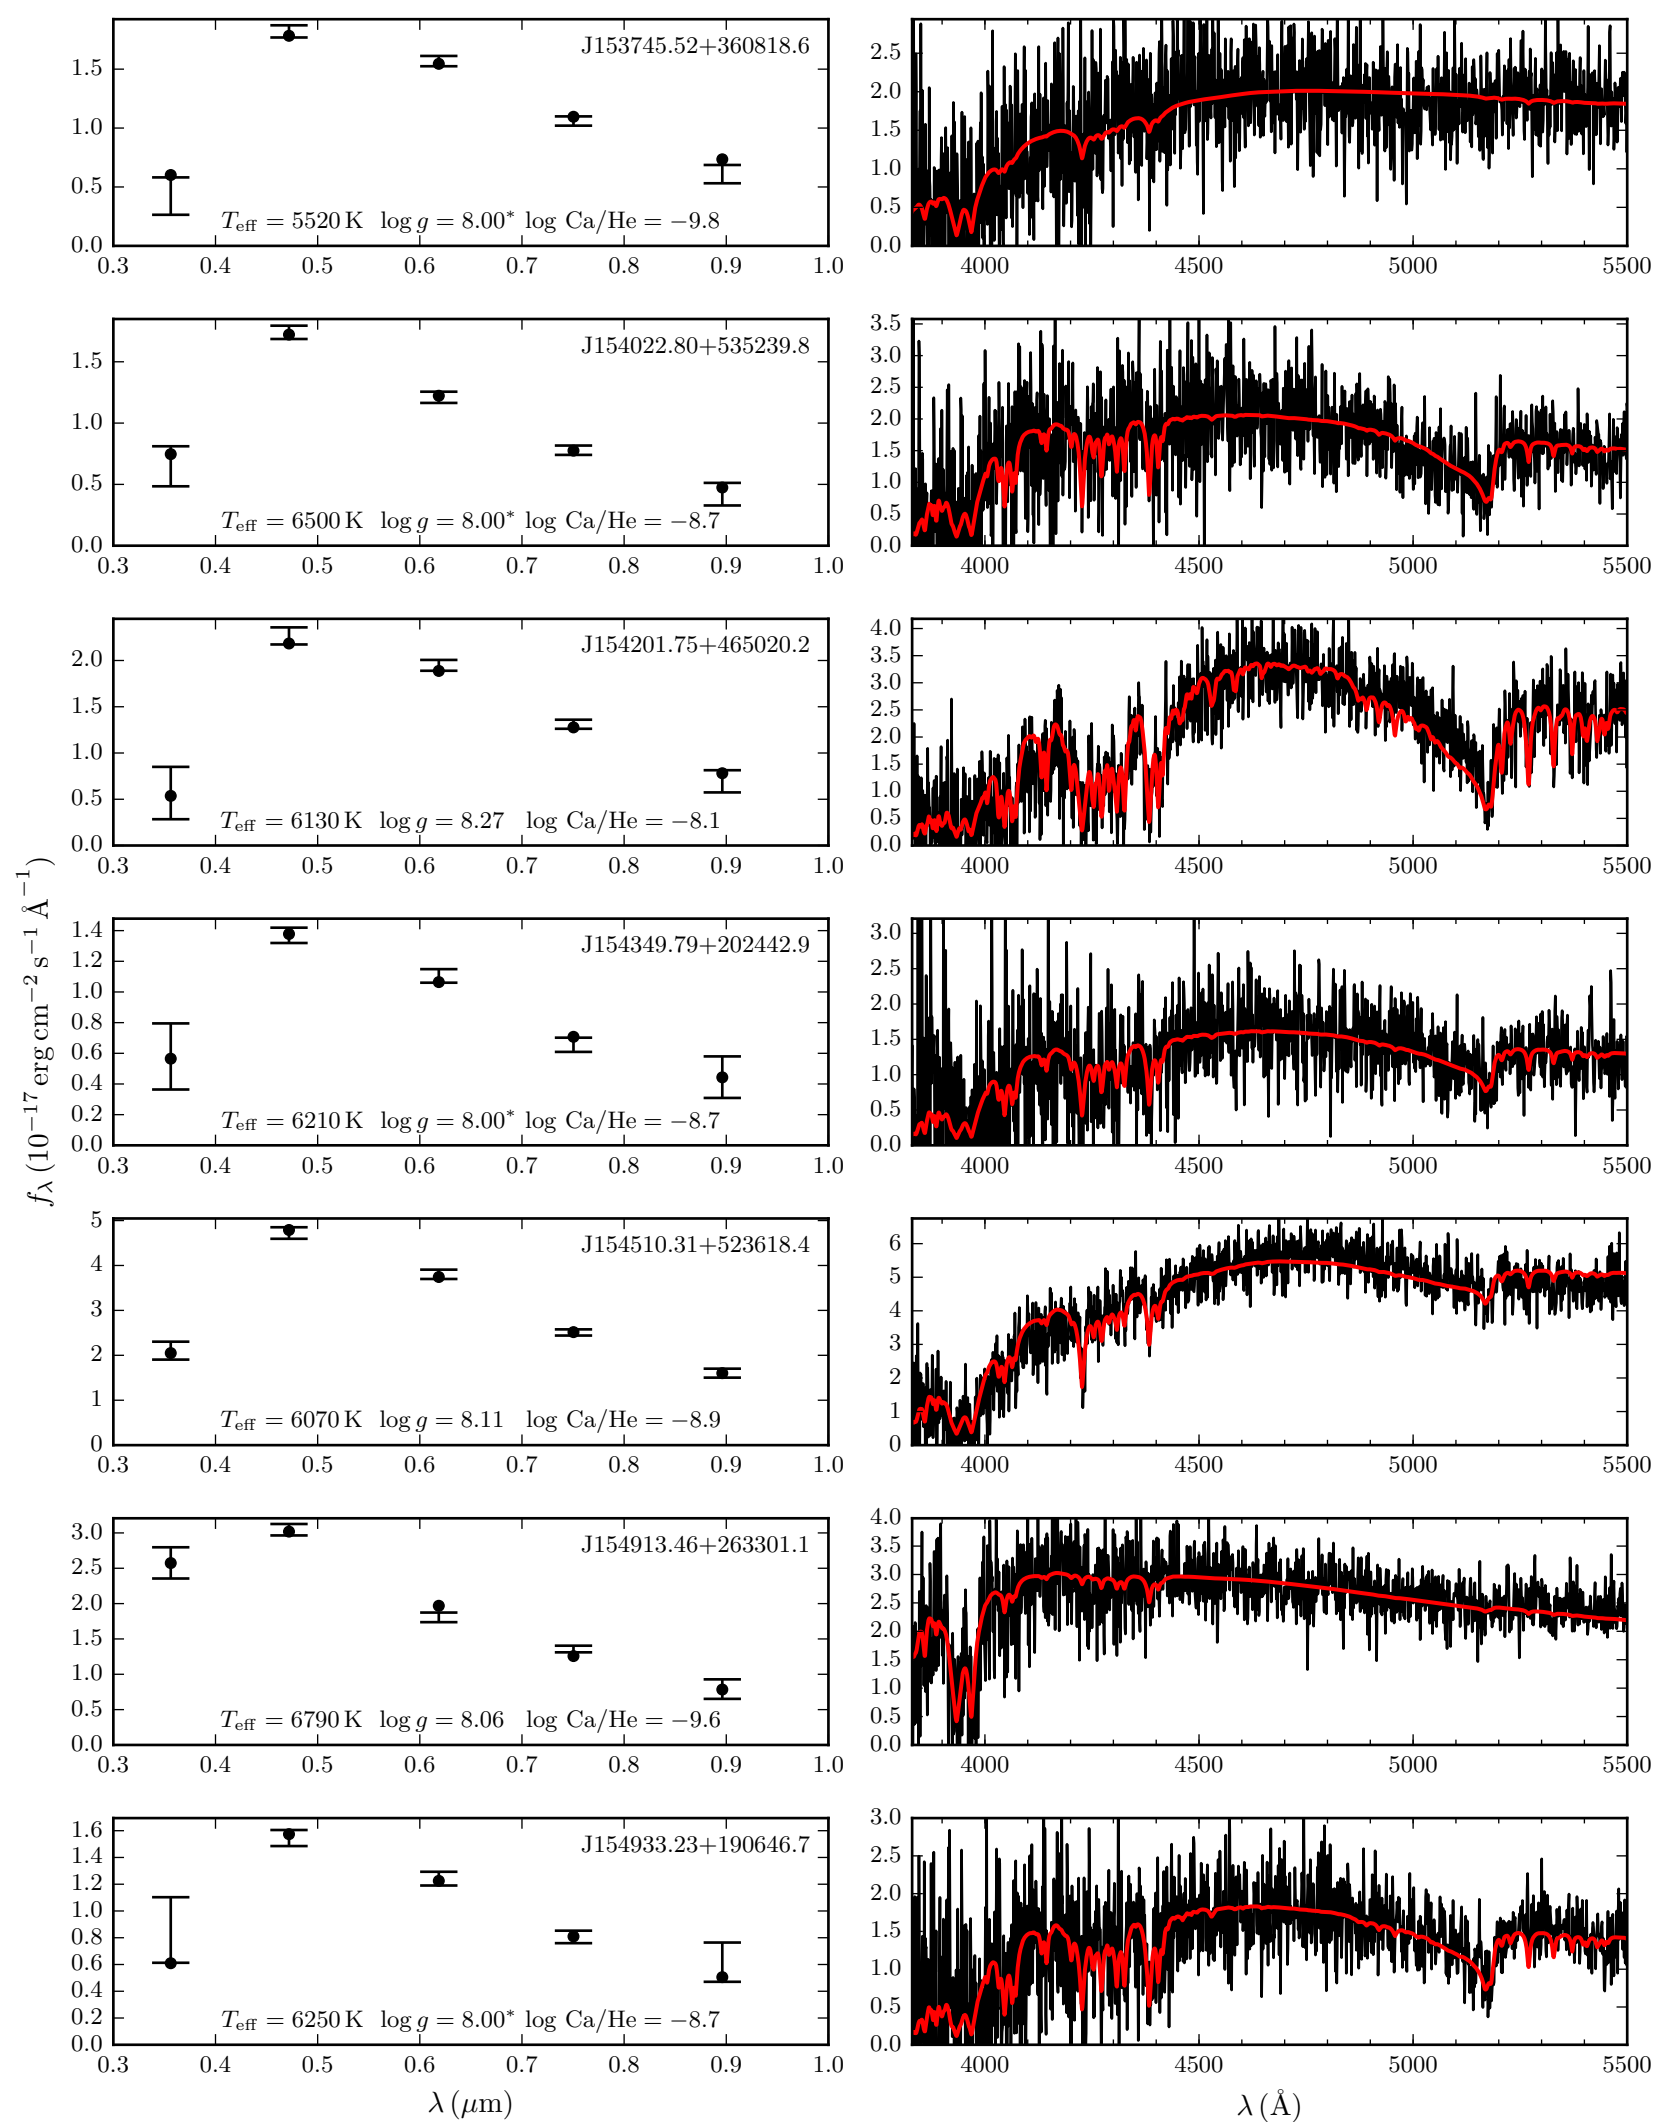

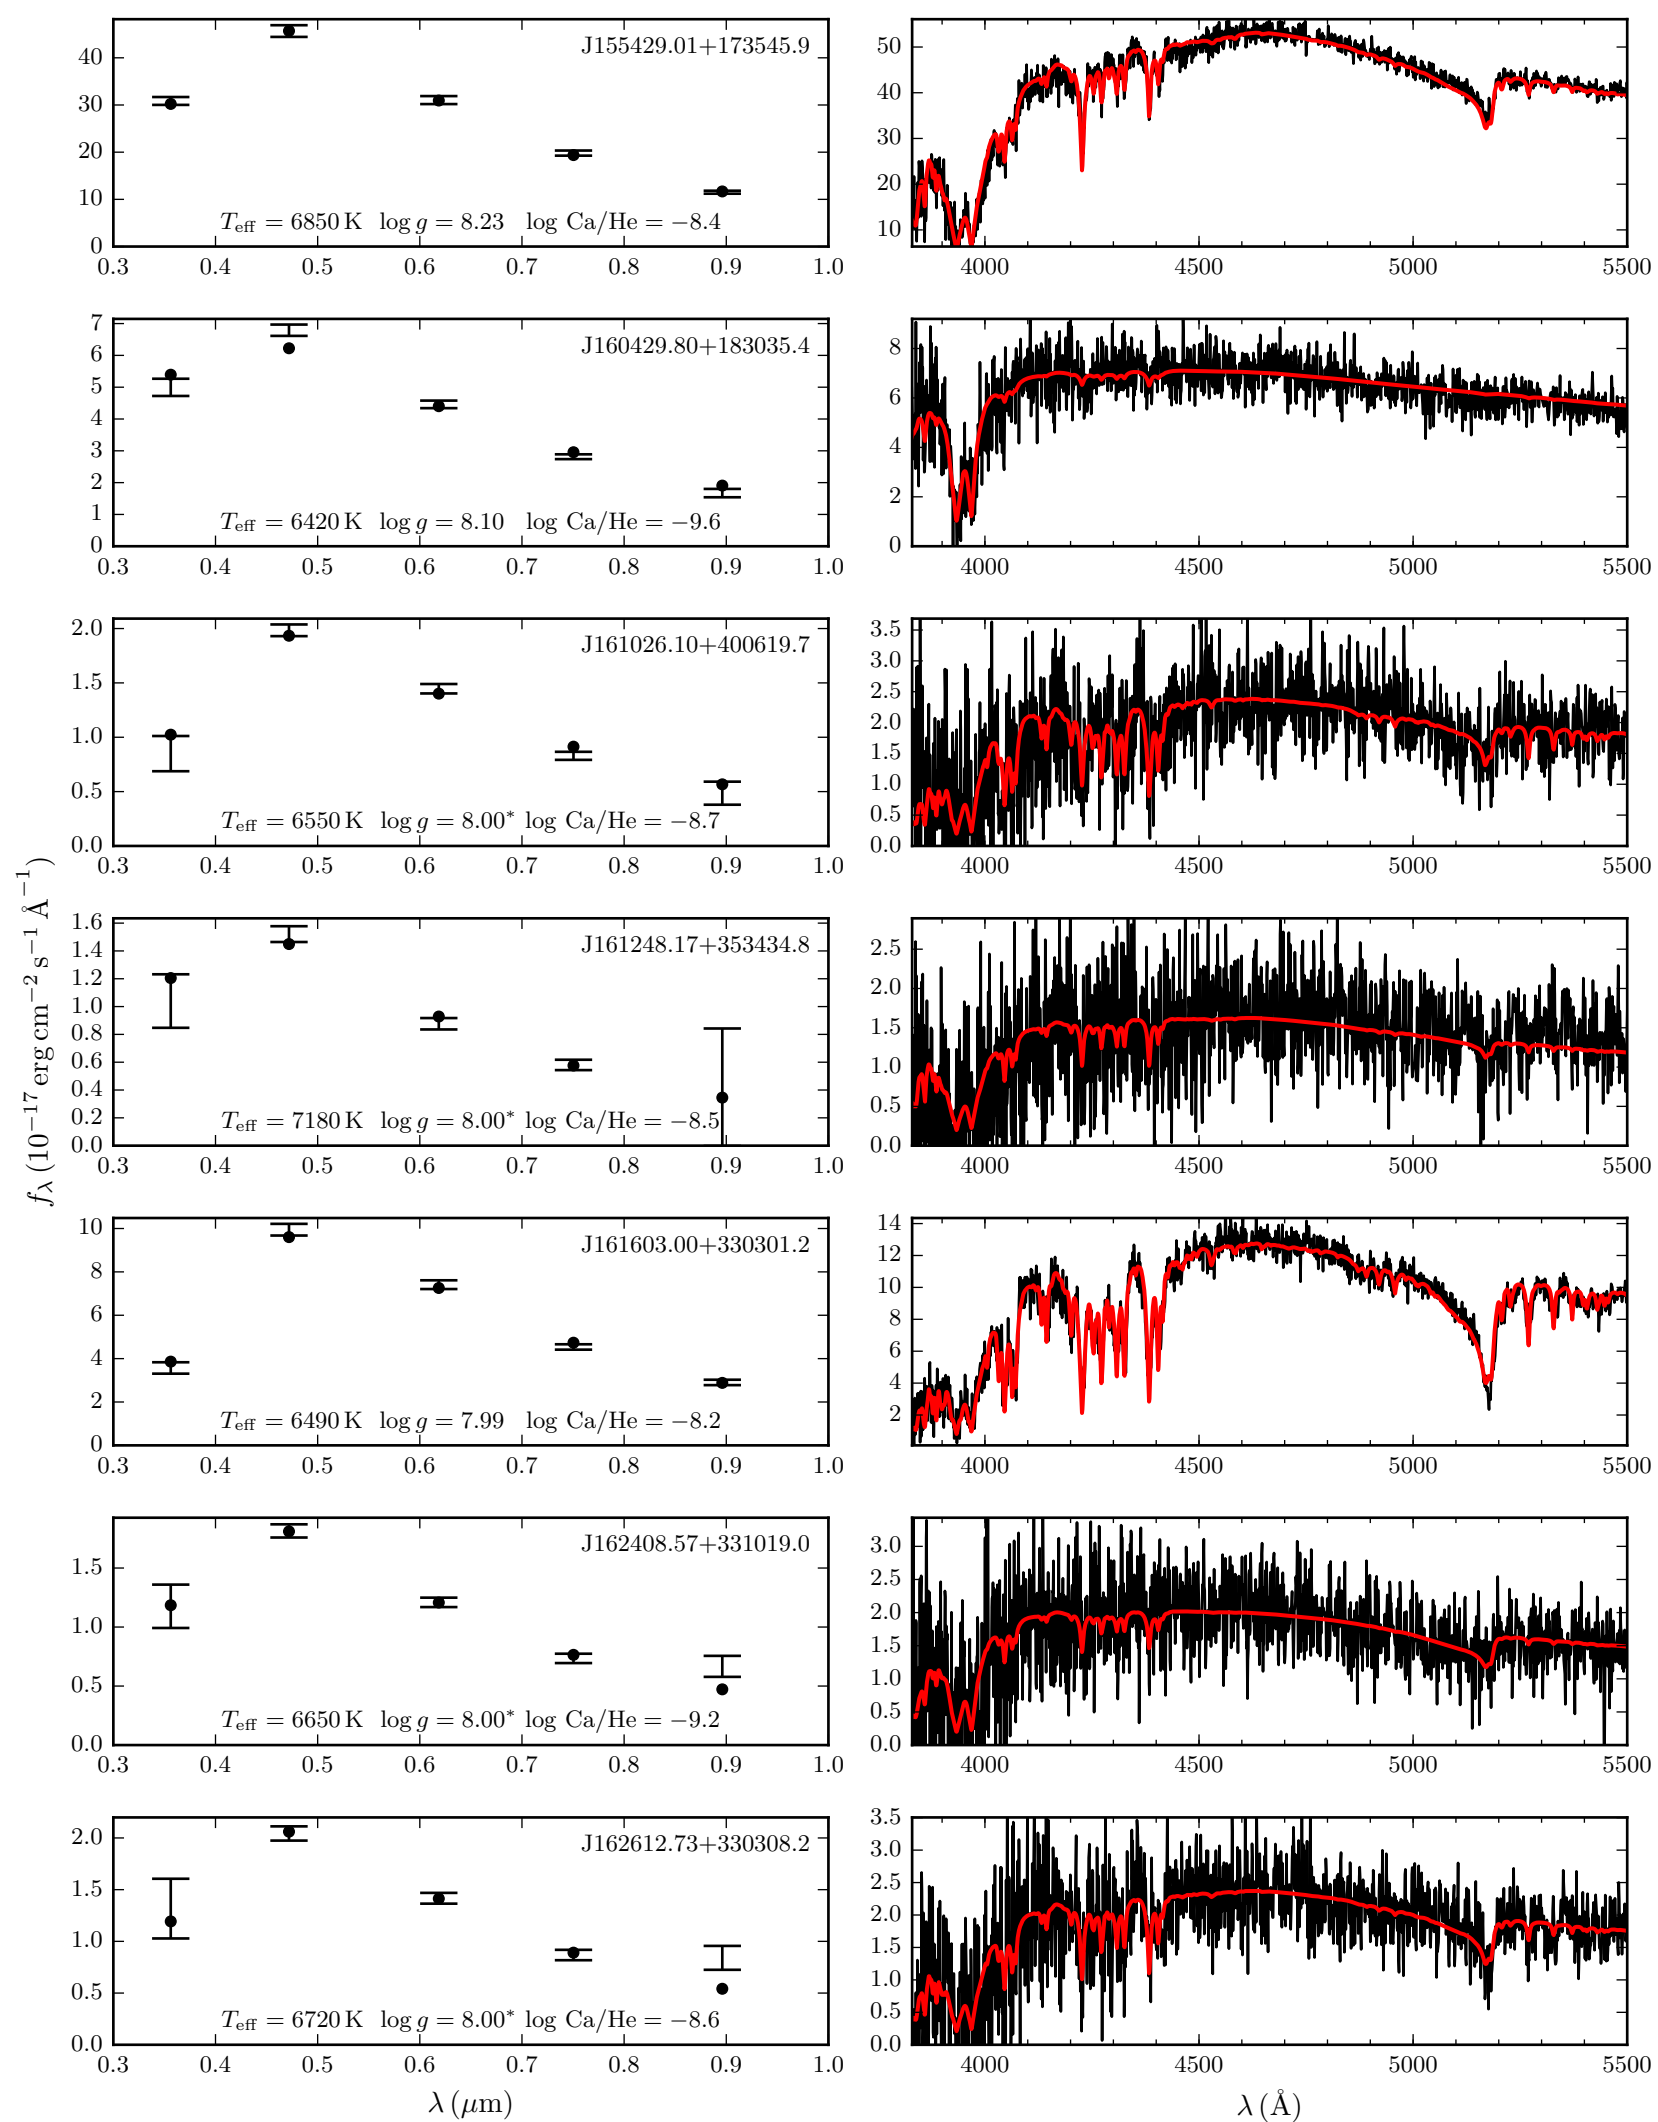

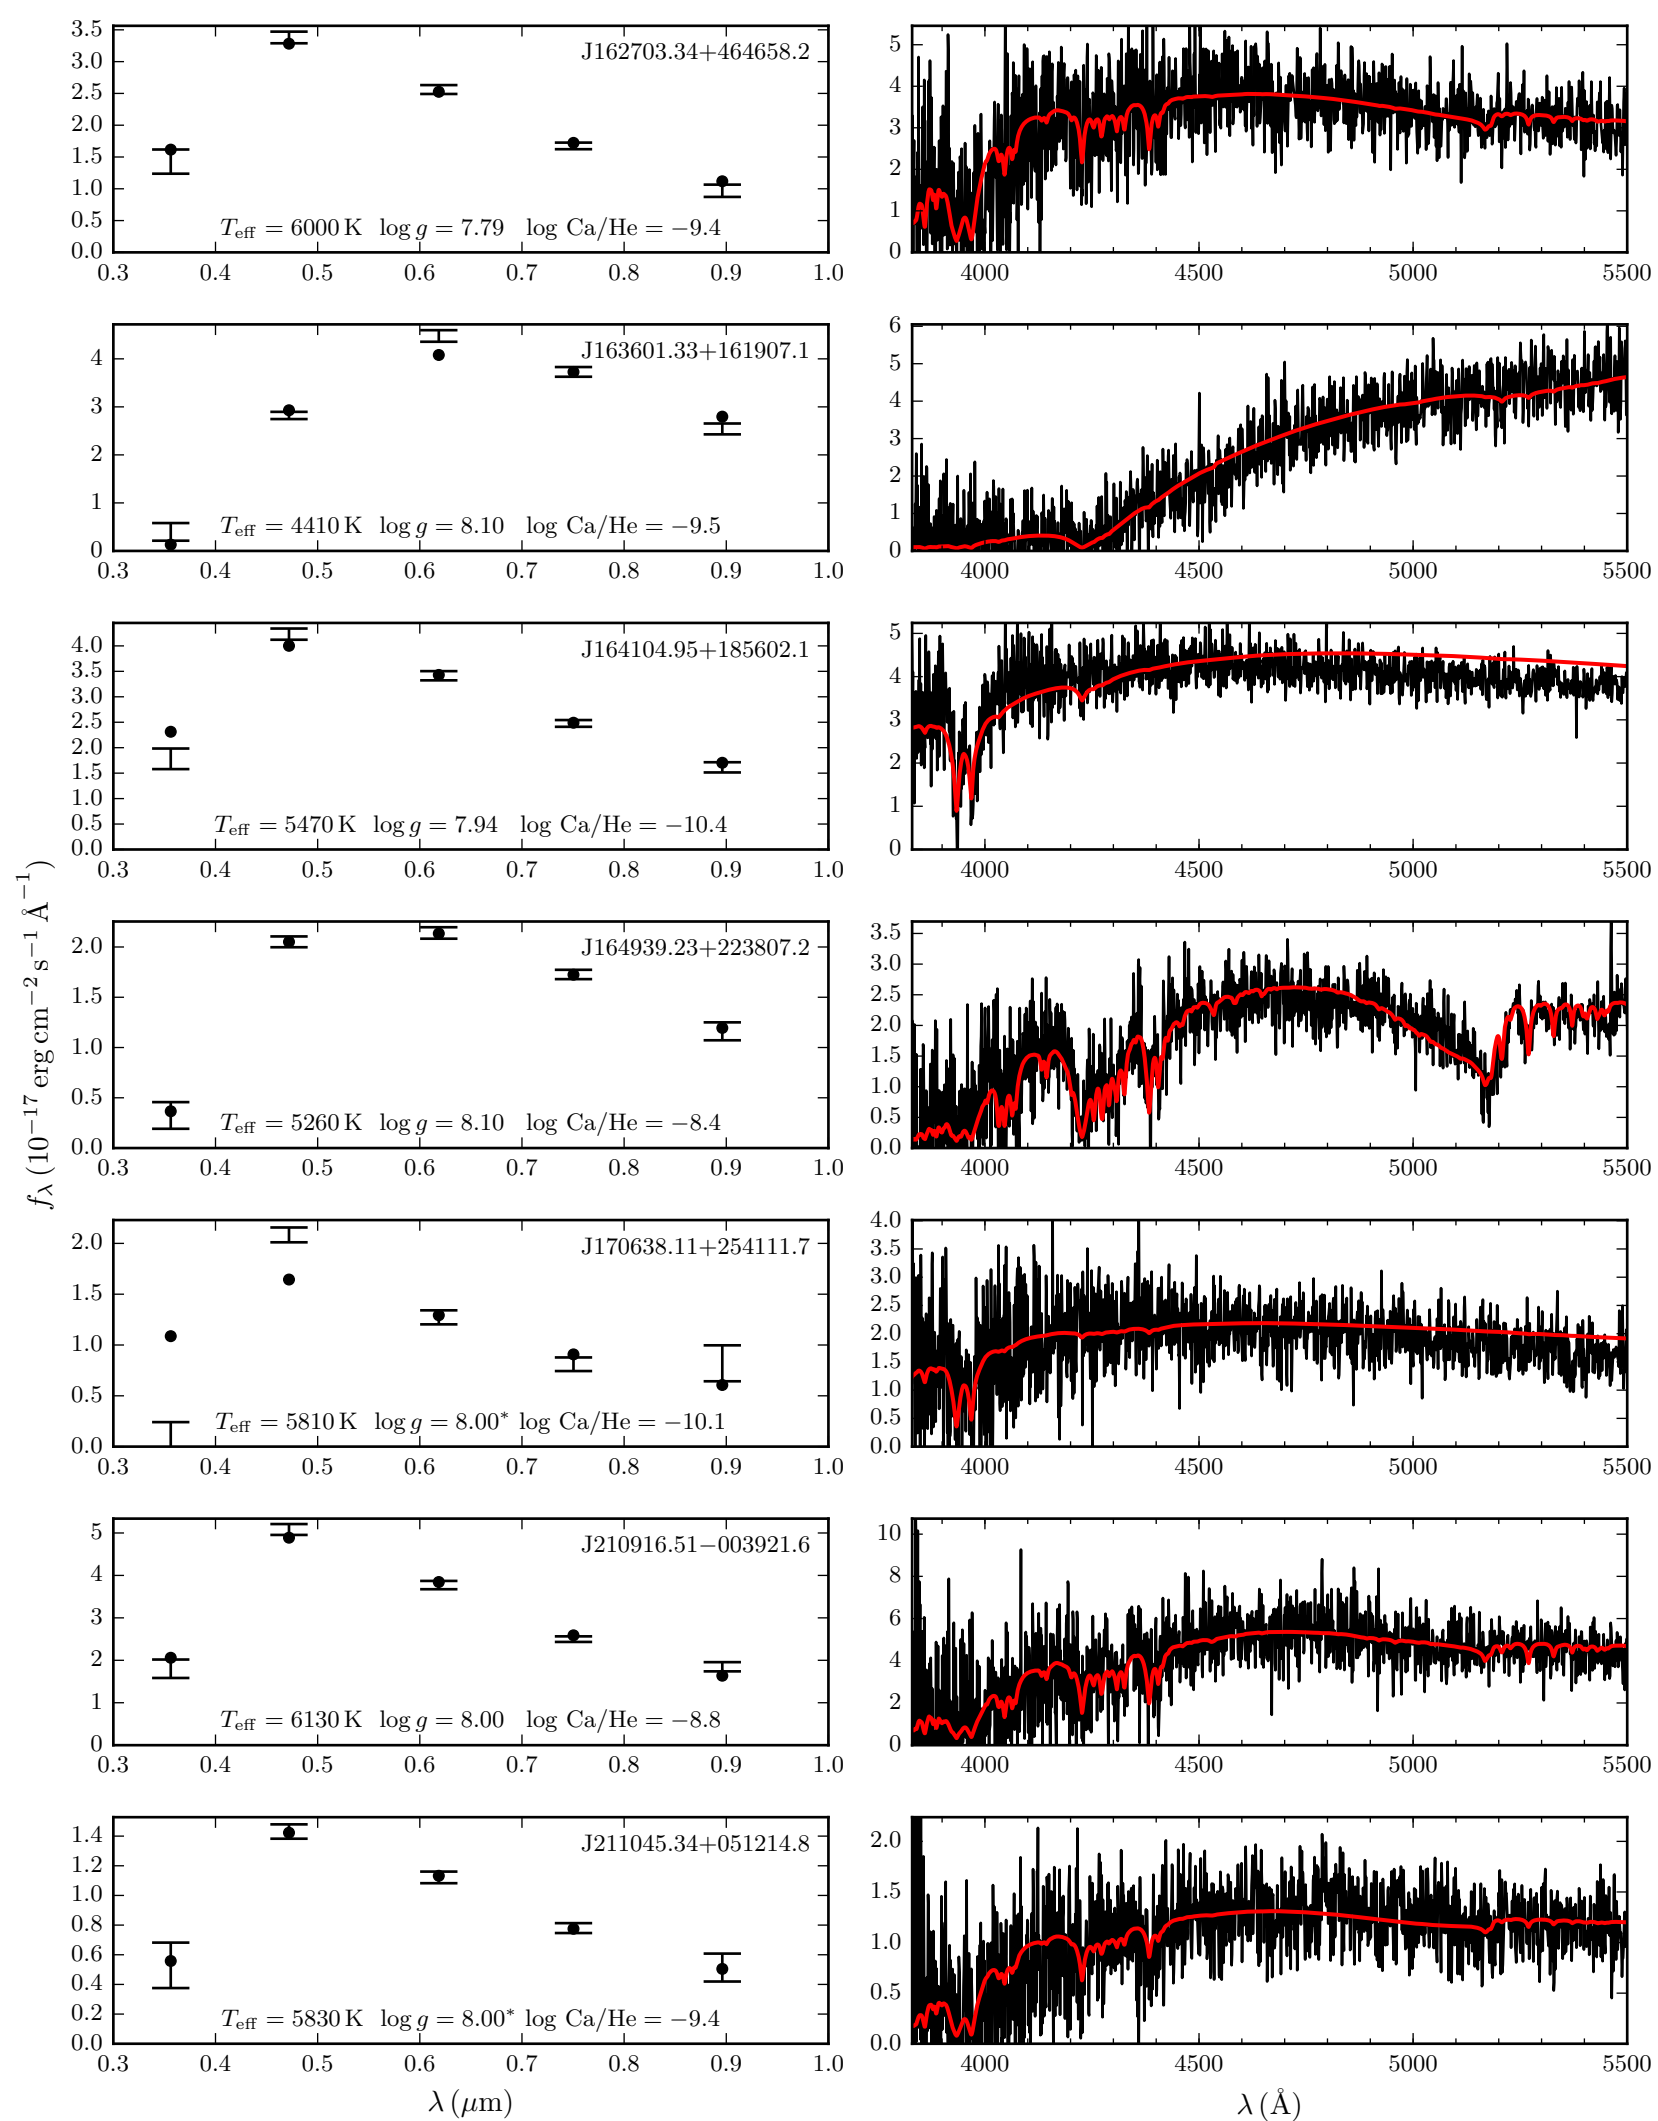

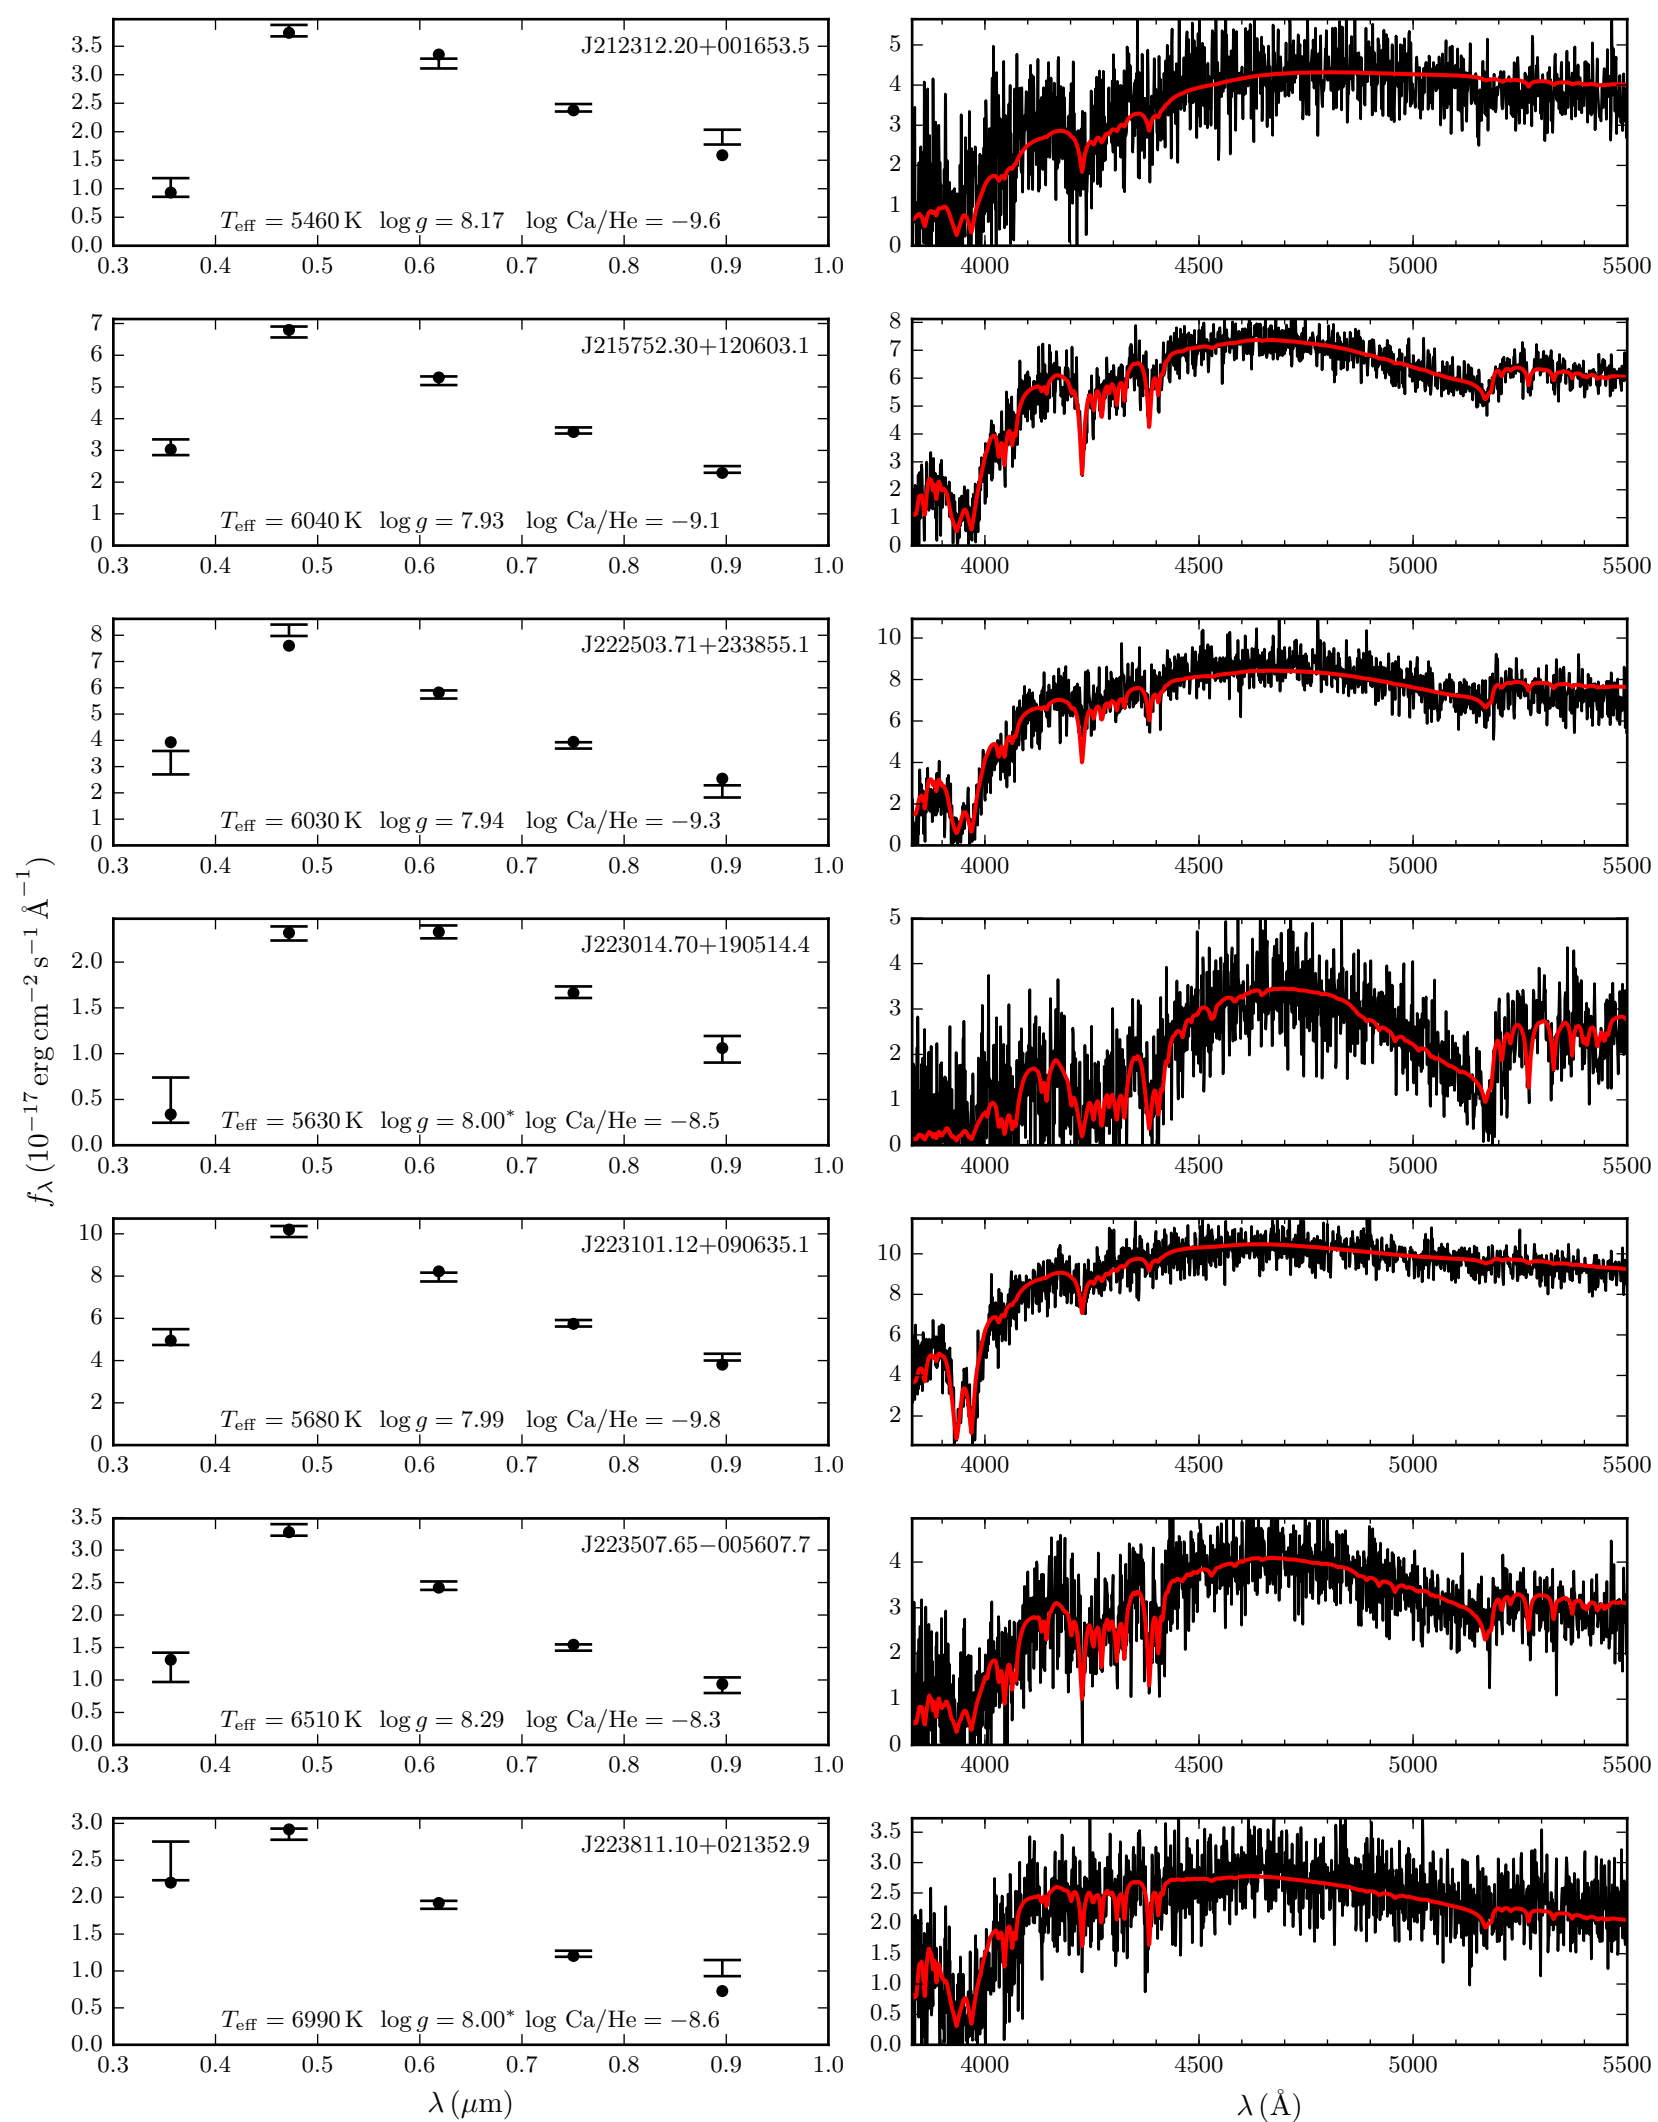

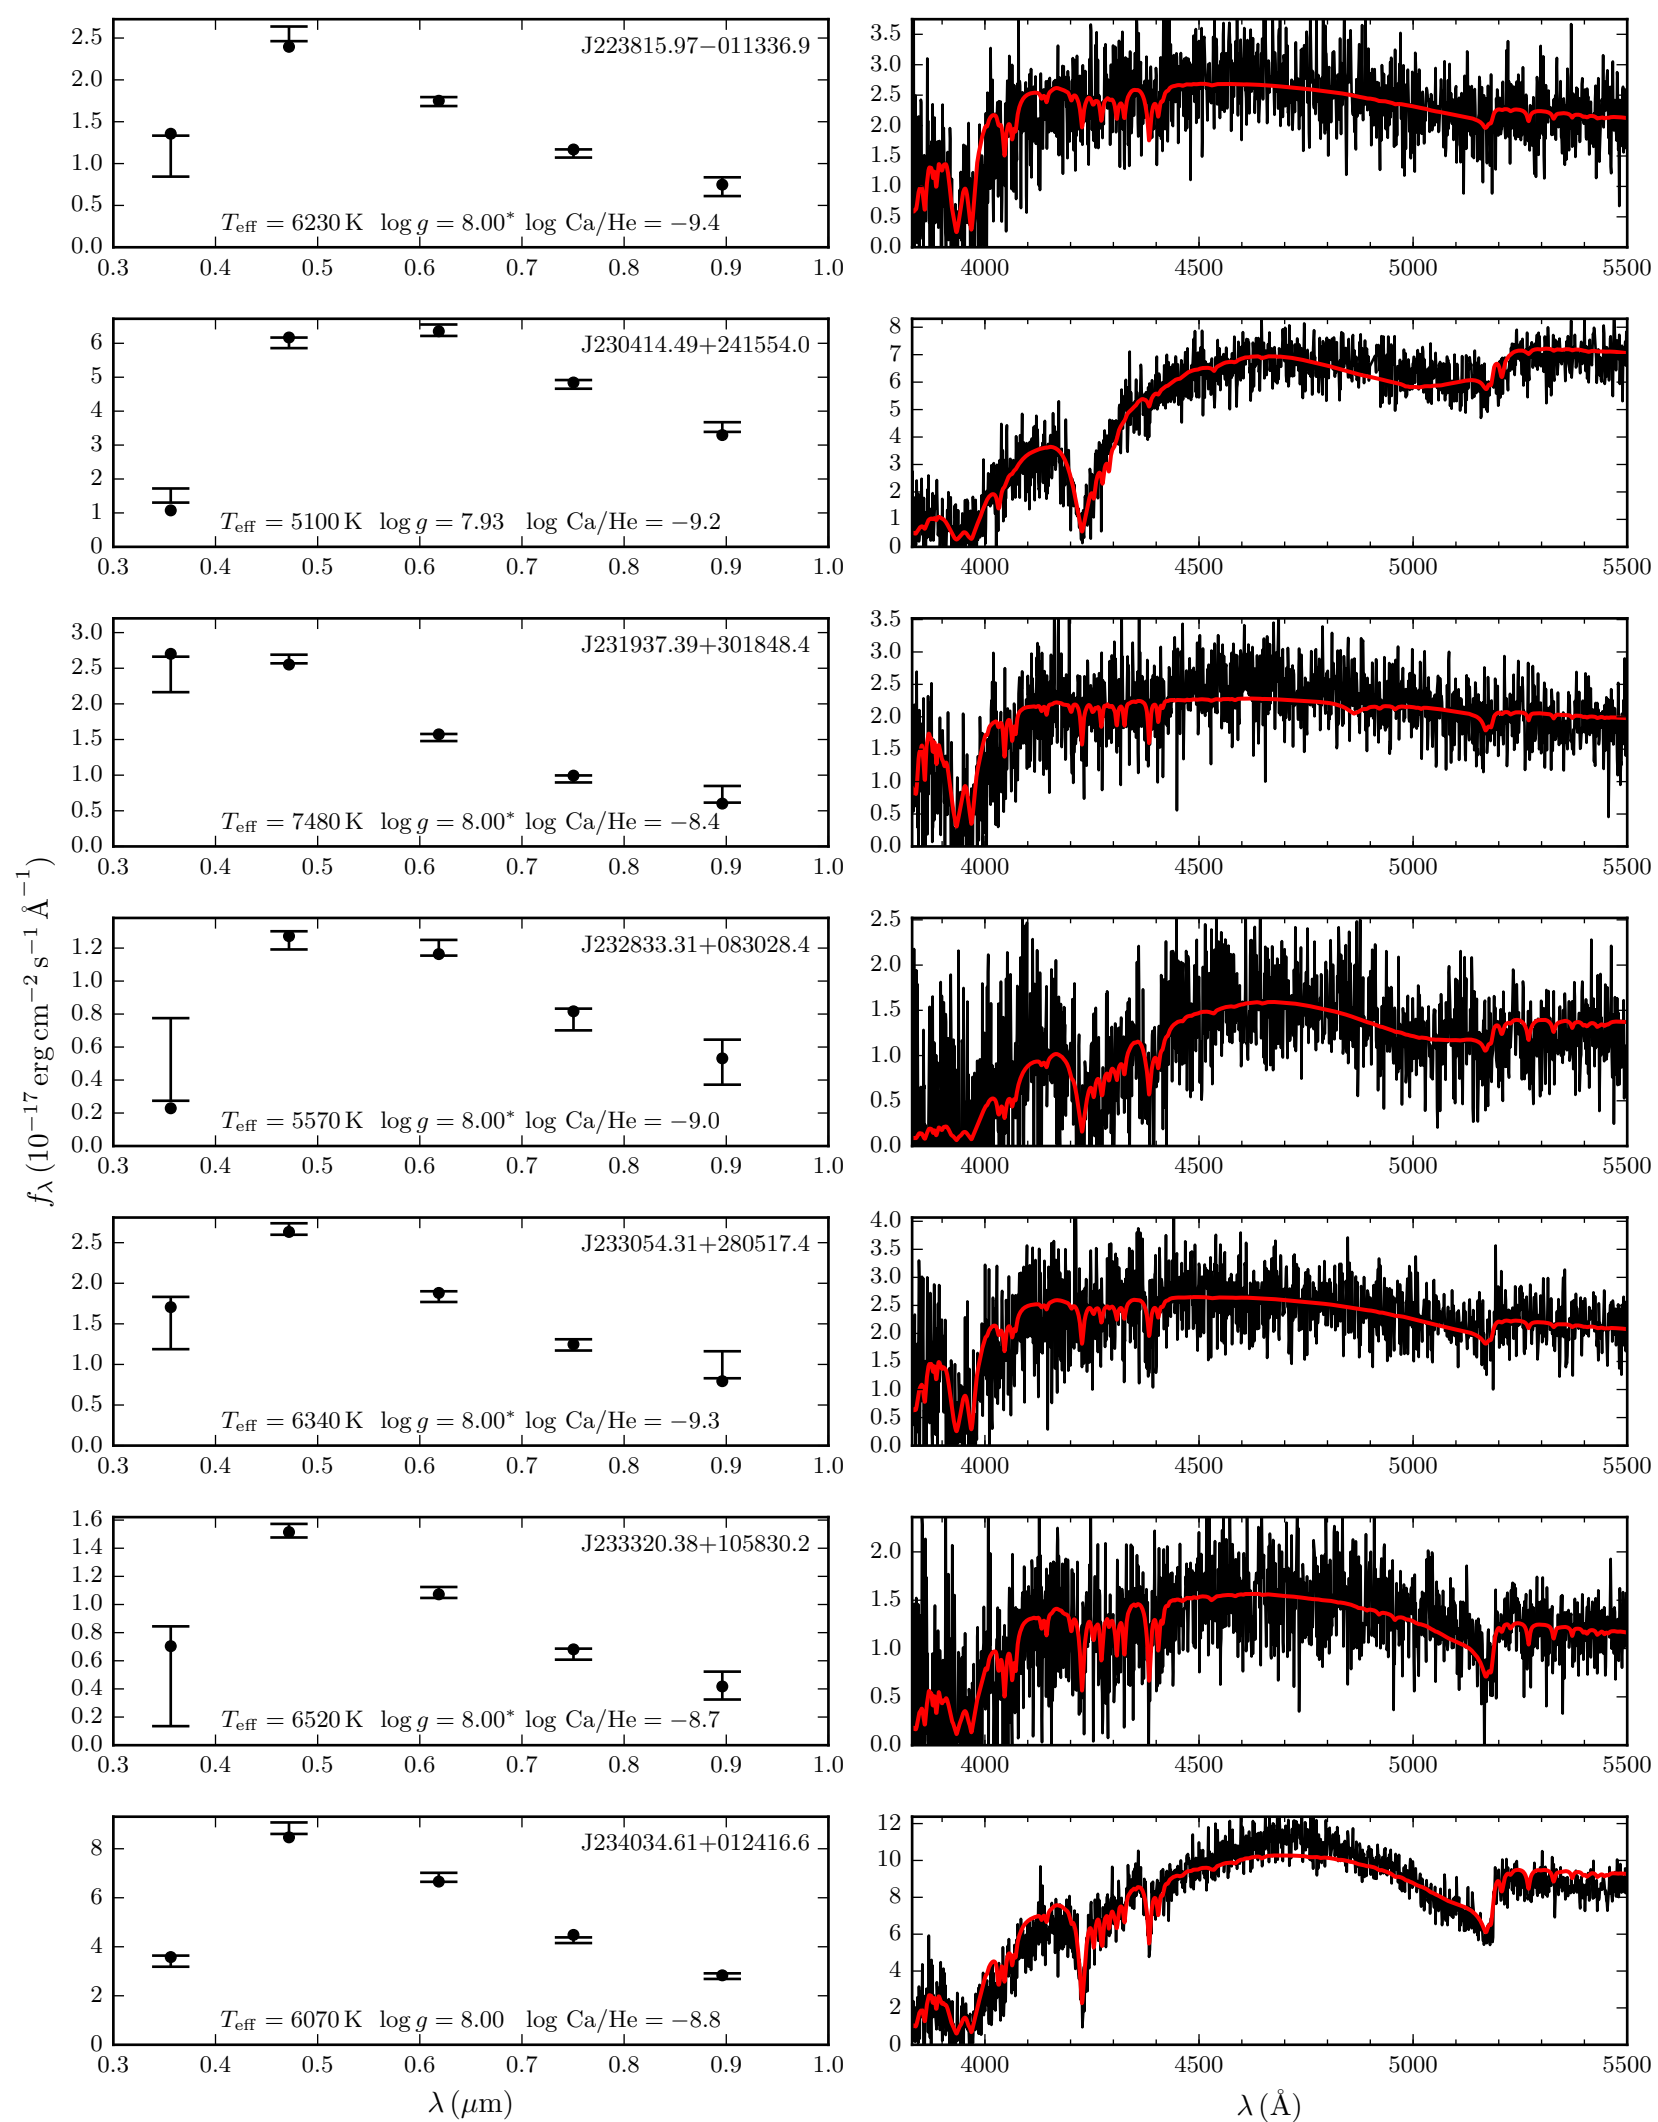

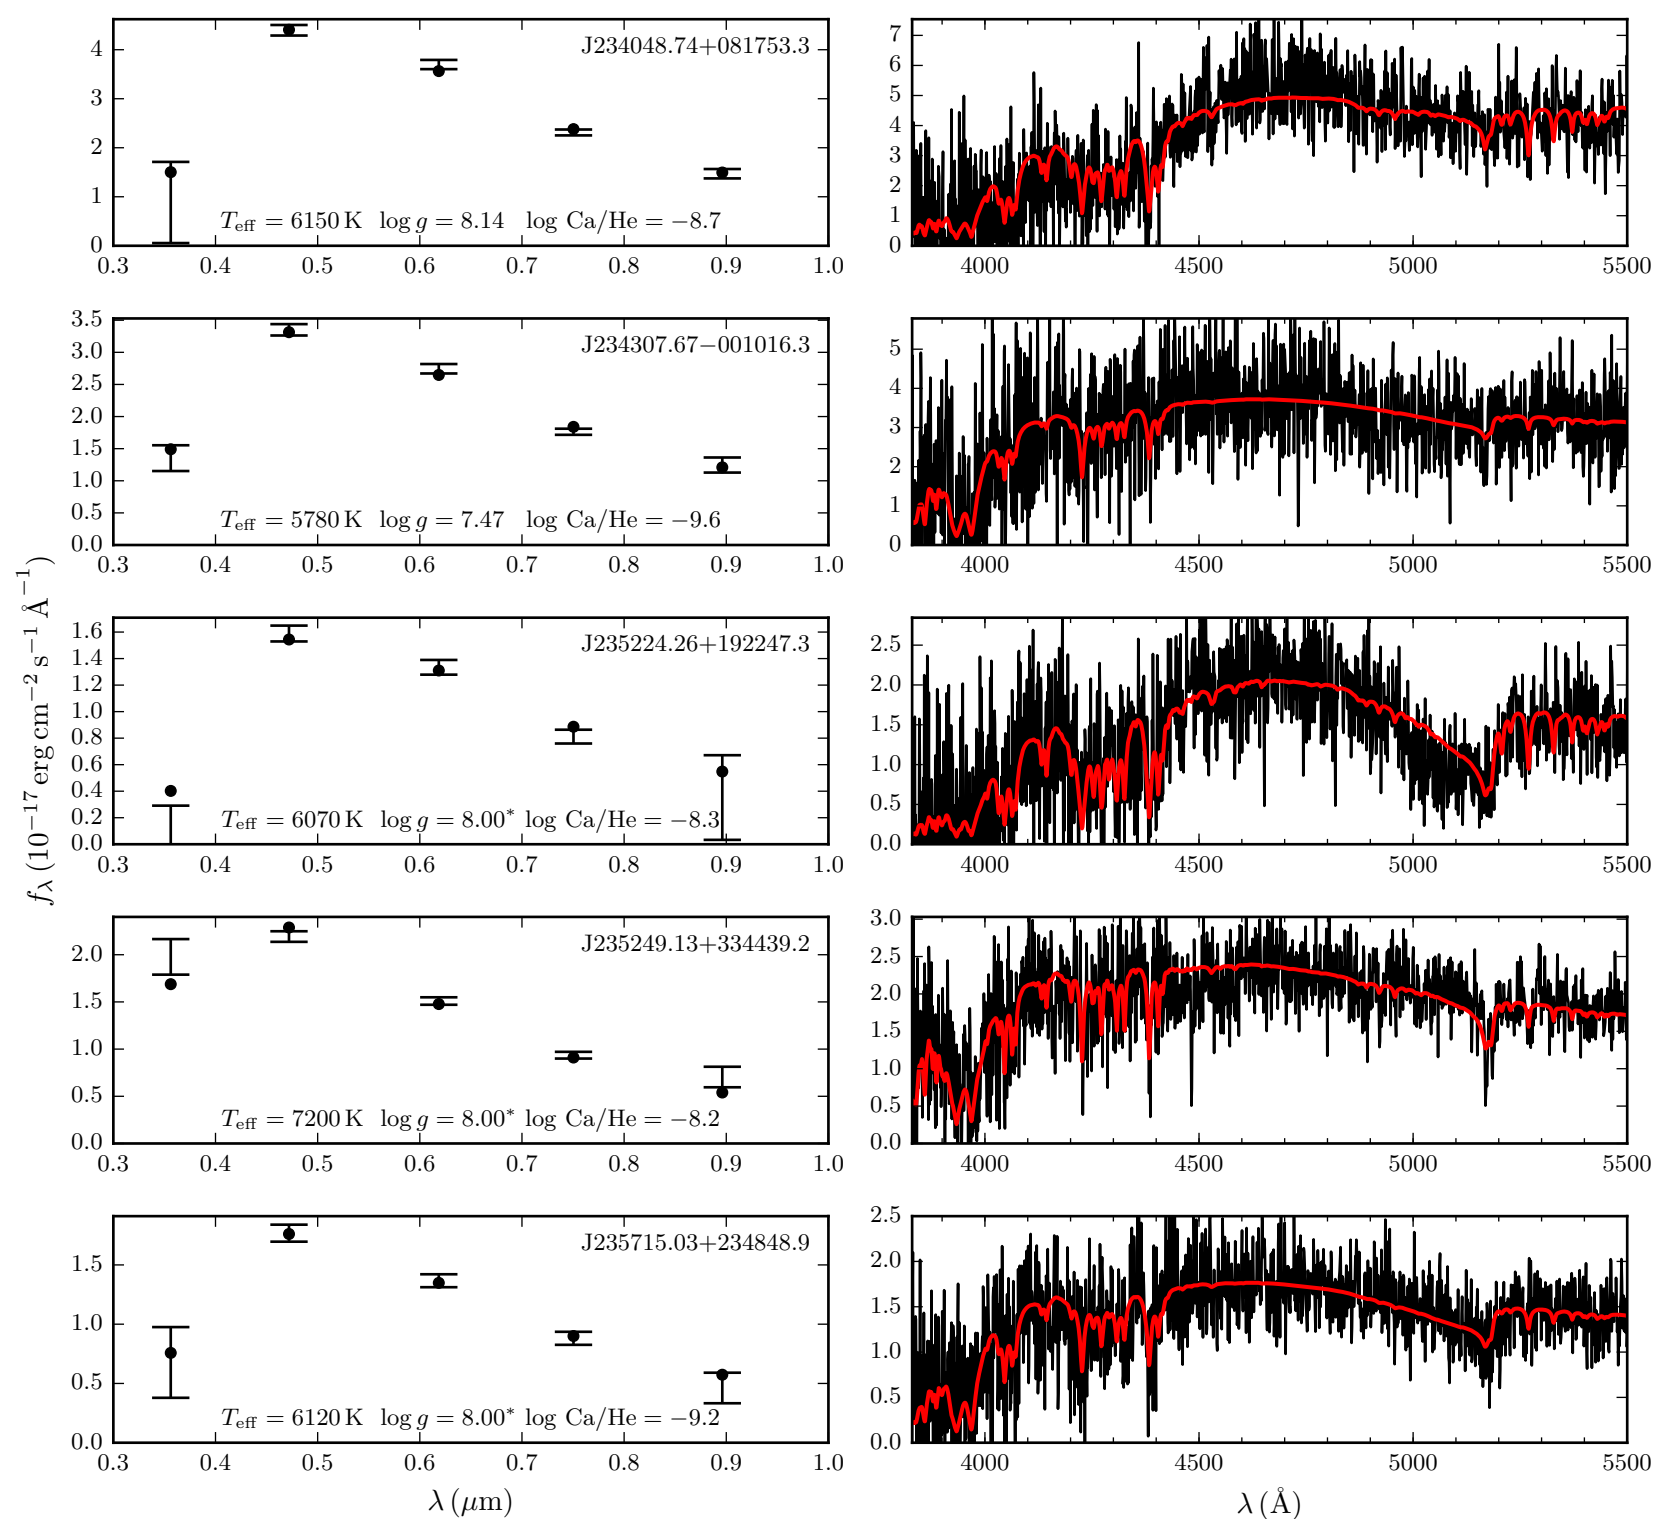

Supplement: Supplementary file 1 [file allfits.pdf]
